# Supplementary material for: NNLO QCD corrections to $\gamma \gamma \rightarrow Q\bar{Q}$ from Local Unitarity combined with Coulomb resummation and NLO EW effects
Source: arXiv:2509.13439 ancillary file (2026-03-25)
Supplement: Supplementary file 1 [file NLO_graphs.pdf]

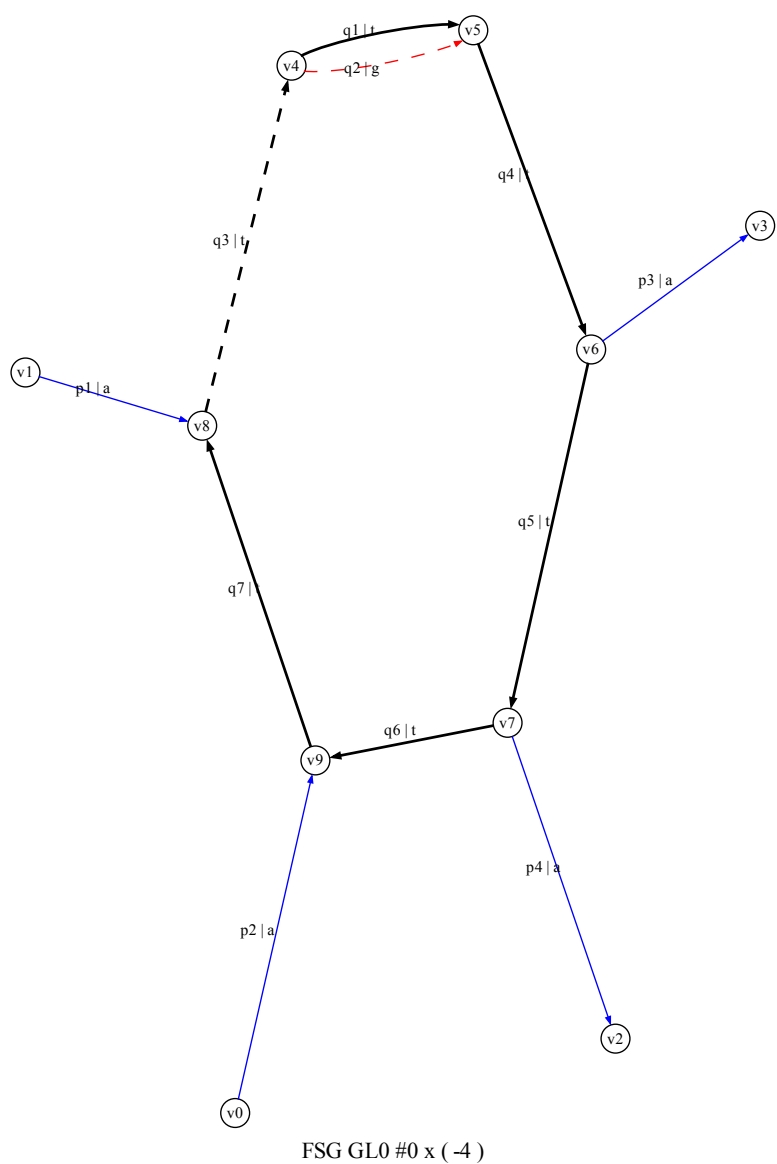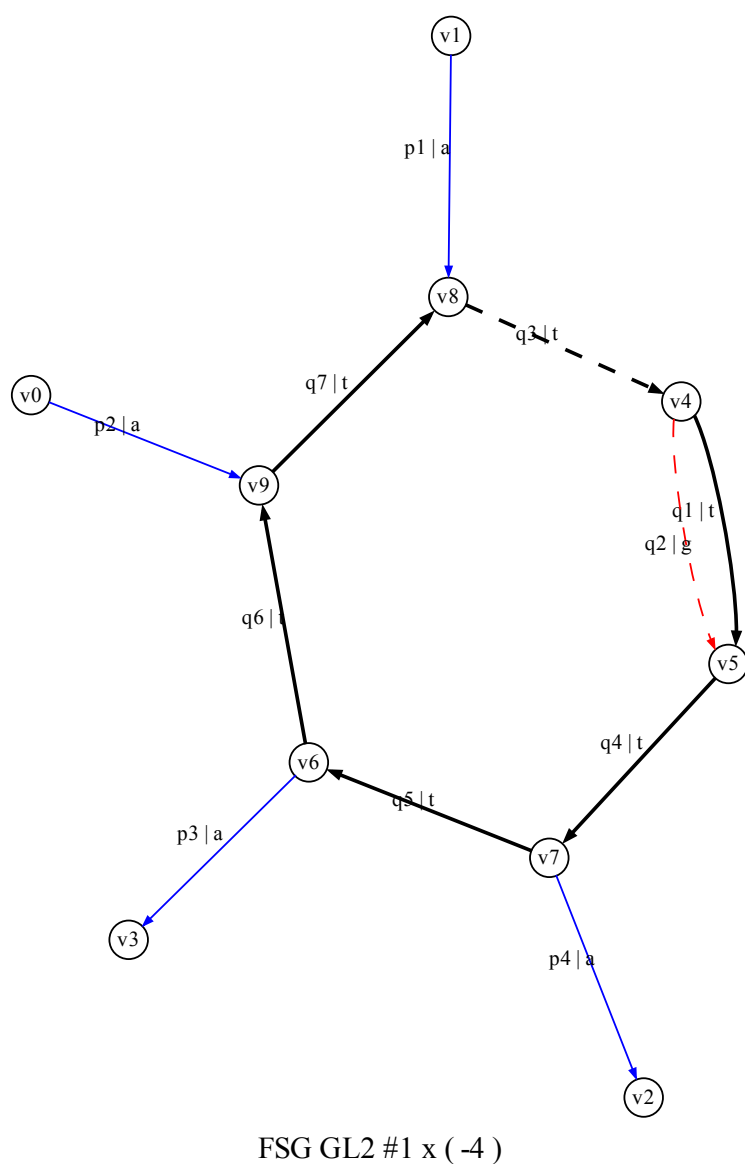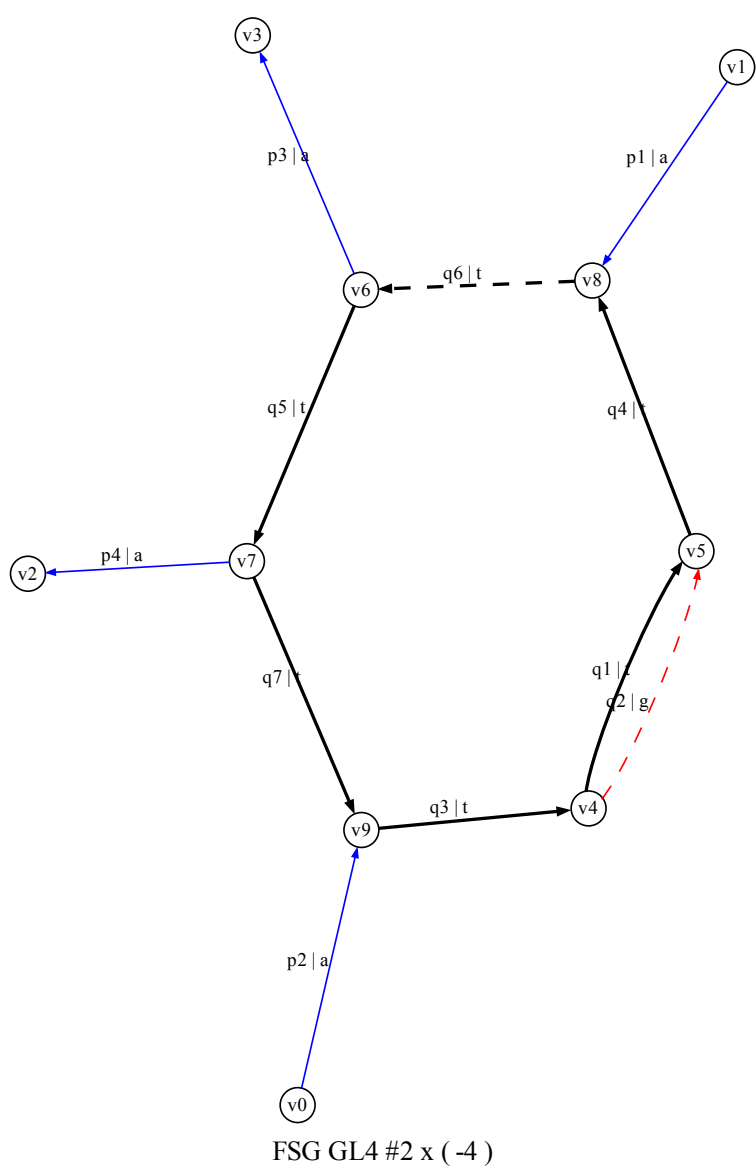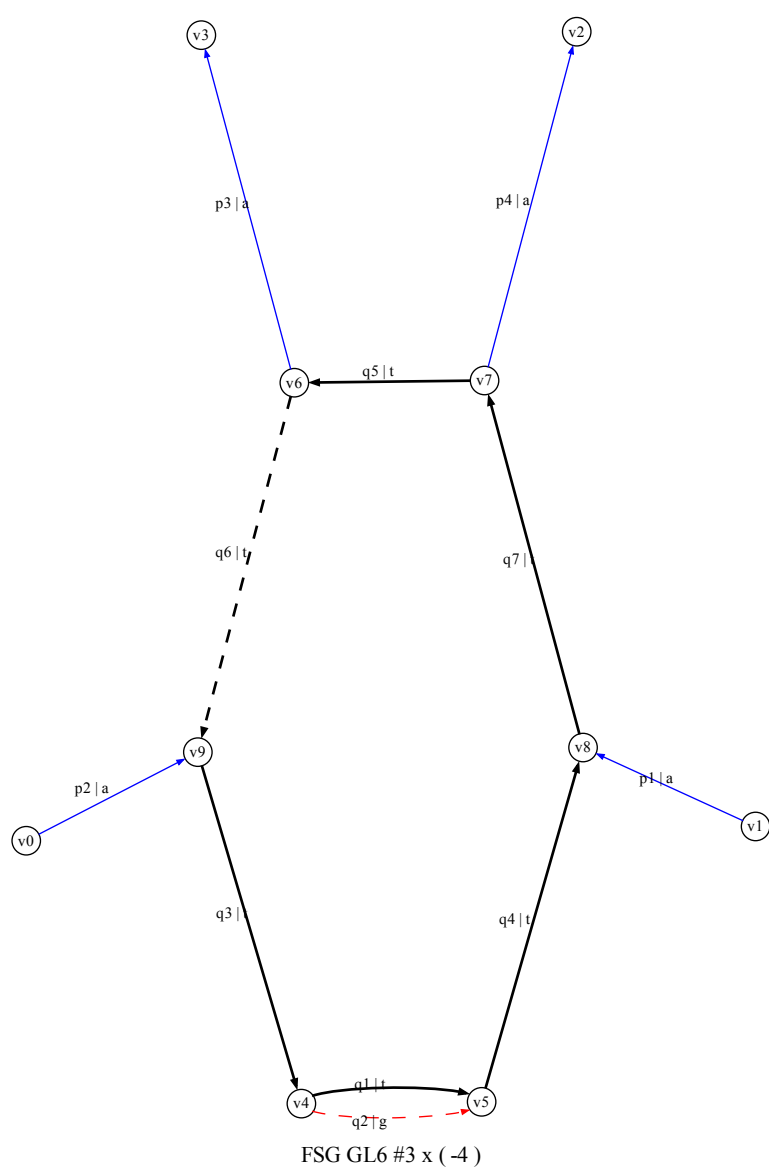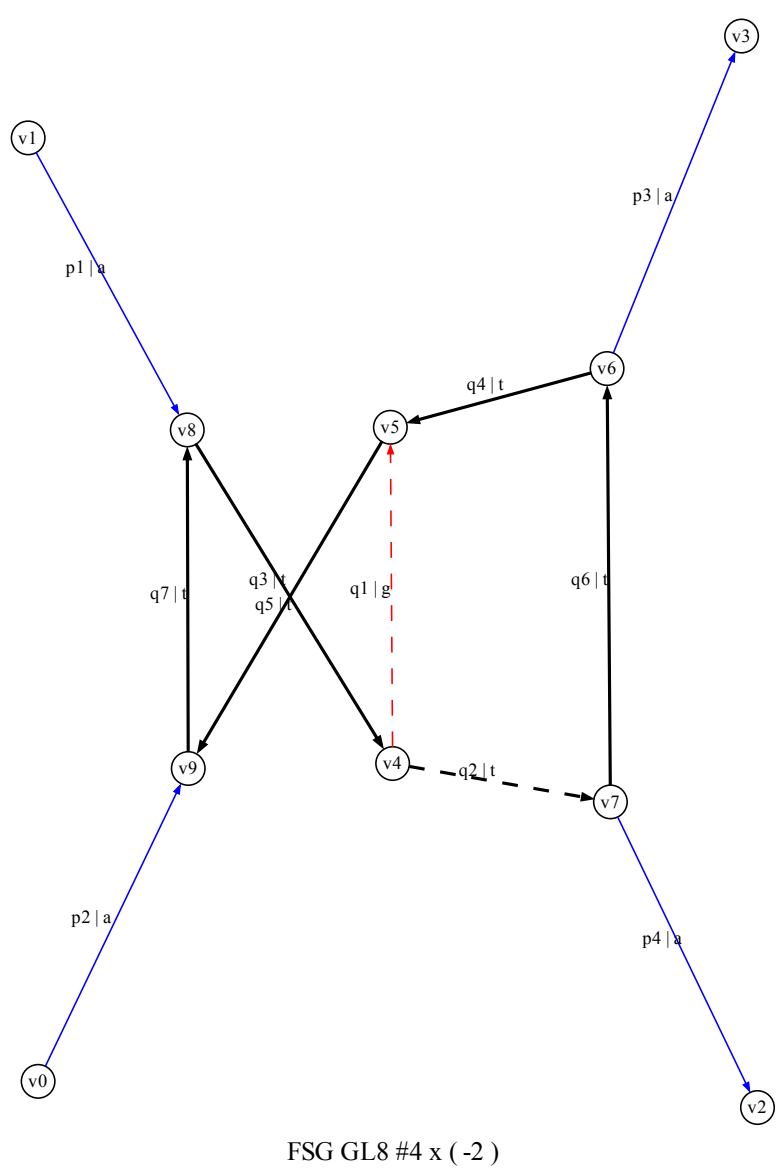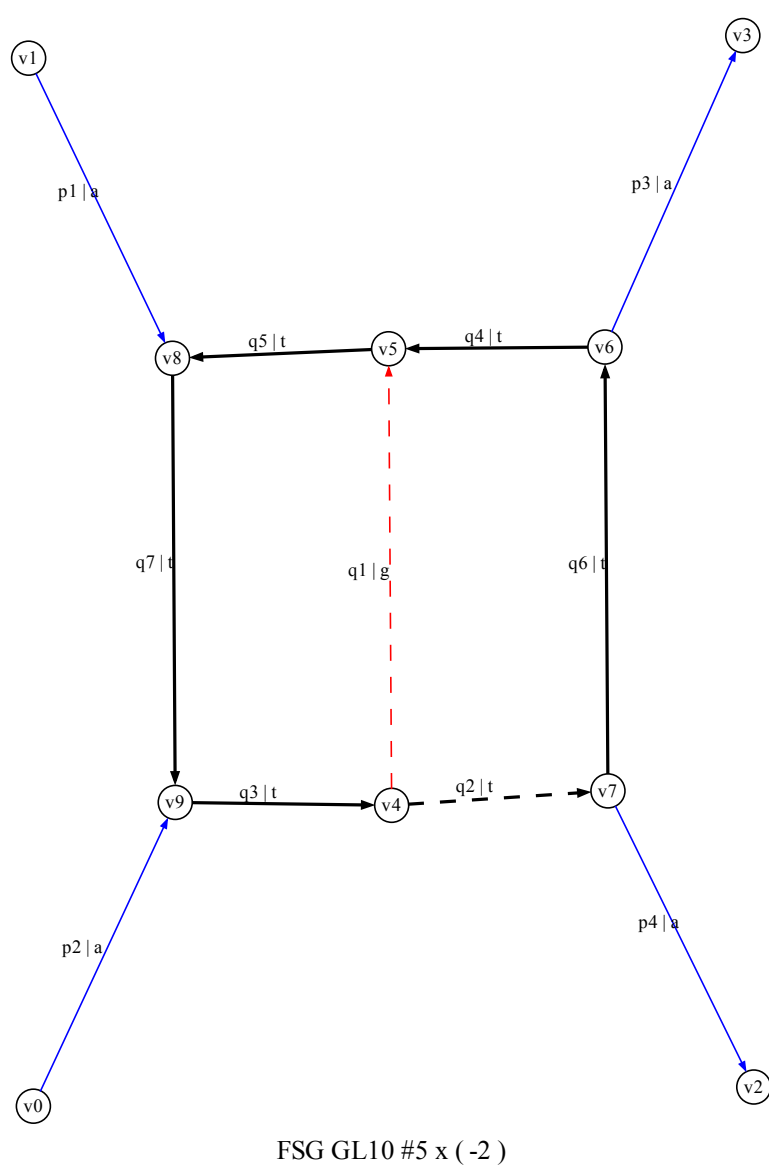

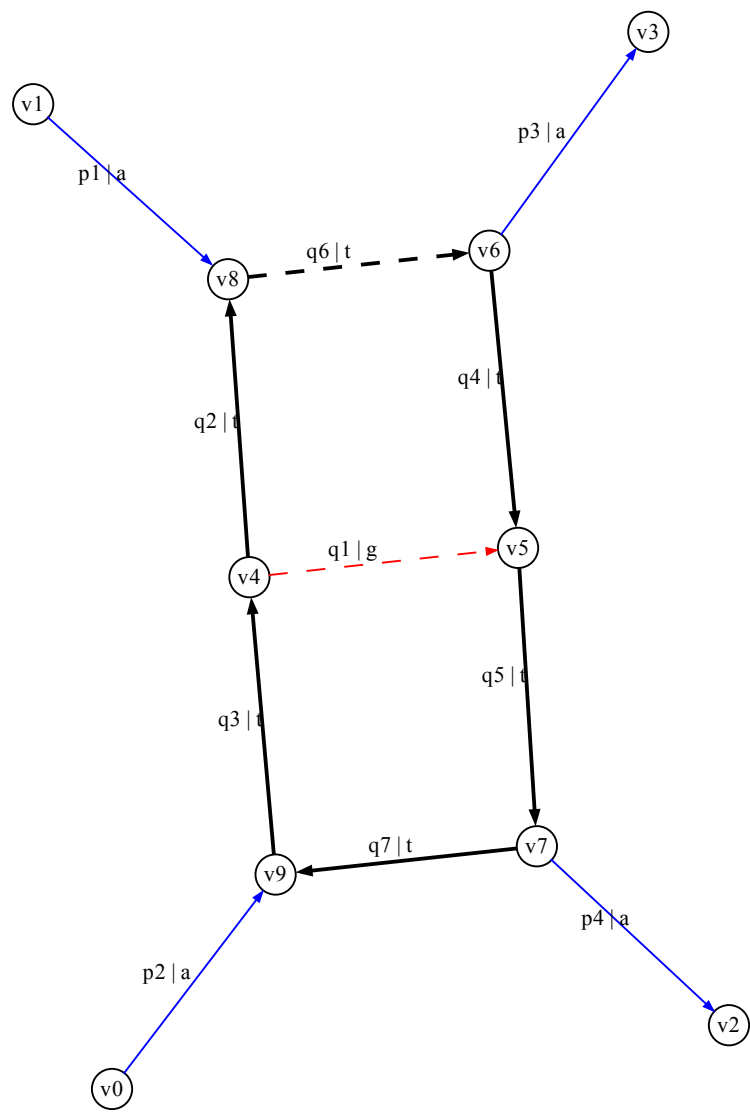

FSG GL16 #6 x (-2)

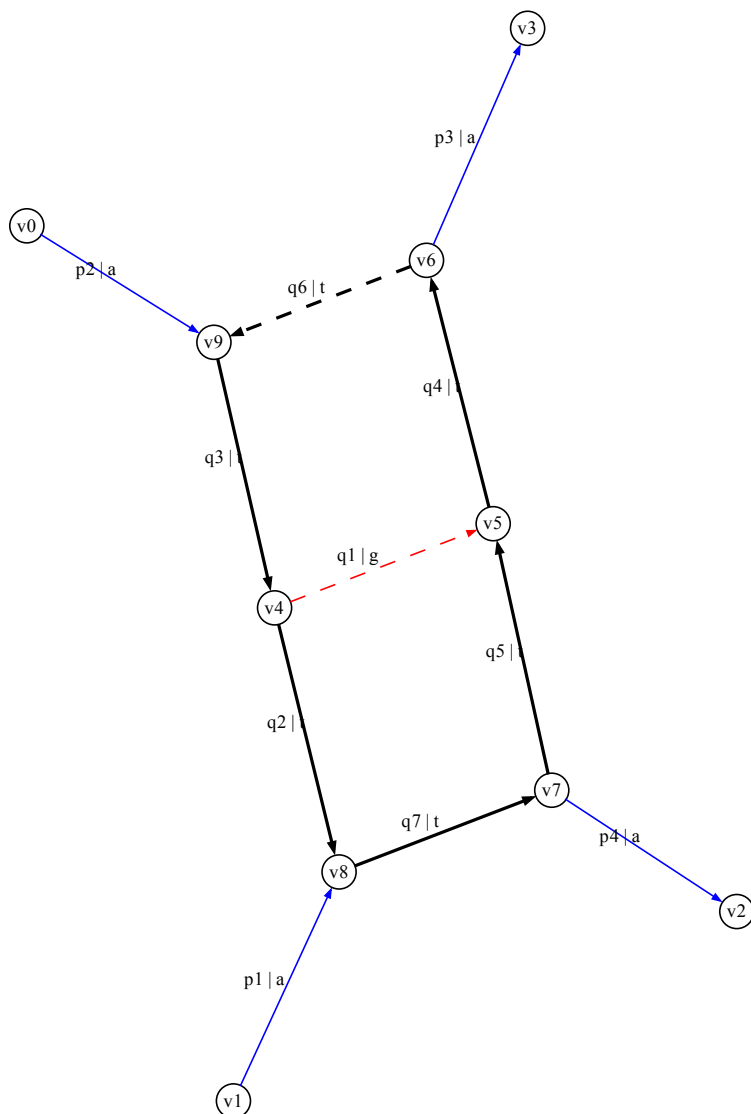

FSG GL18 #7 x (-2)

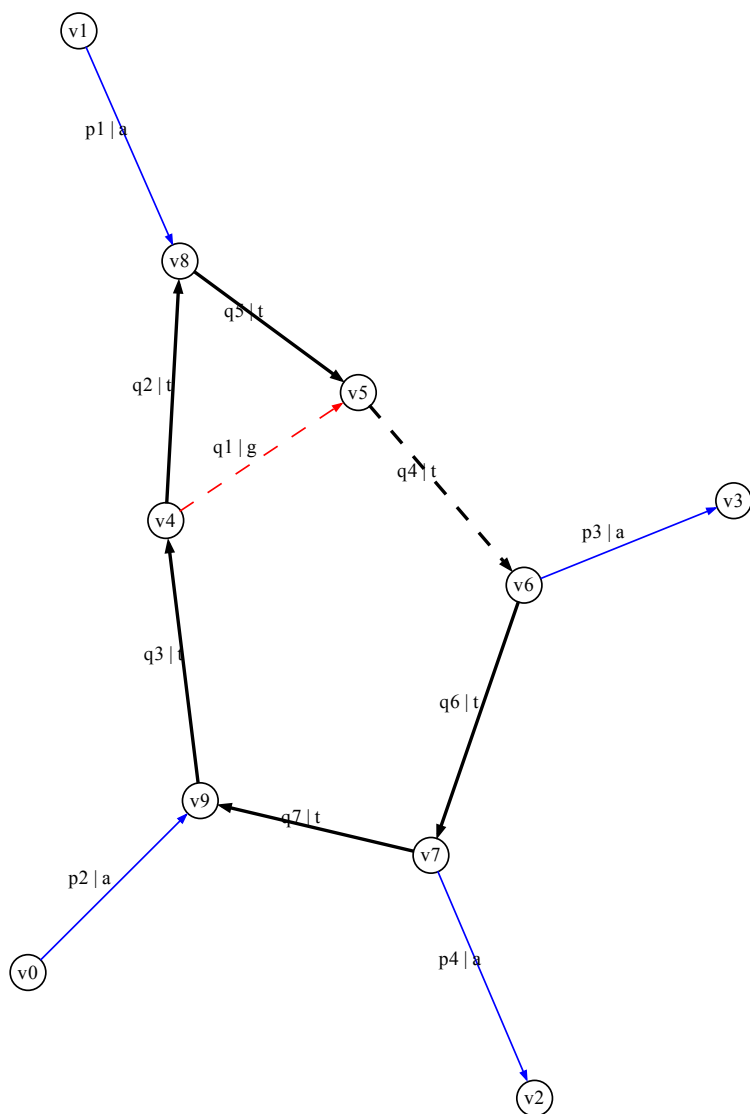

FSG GL20 #8 x (-8)

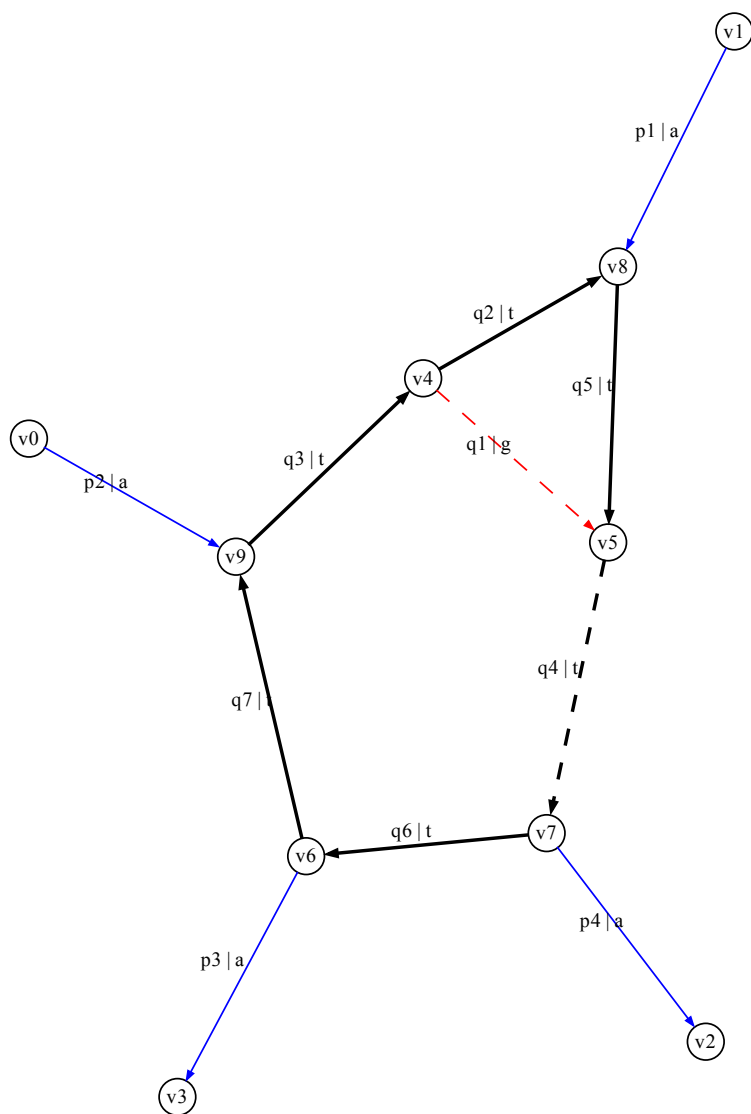

FSG GL22 #9 x (-8)
