# Supplementary material for: NNLO QCD corrections to $\gamma \gamma \rightarrow Q\bar{Q}$ from Local Unitarity combined with Coulomb resummation and NLO EW effects
Source: arXiv:2509.13439 ancillary file (2026-03-25)
Supplement: Supplementary file 2 [file NNLO_graphs.pdf]

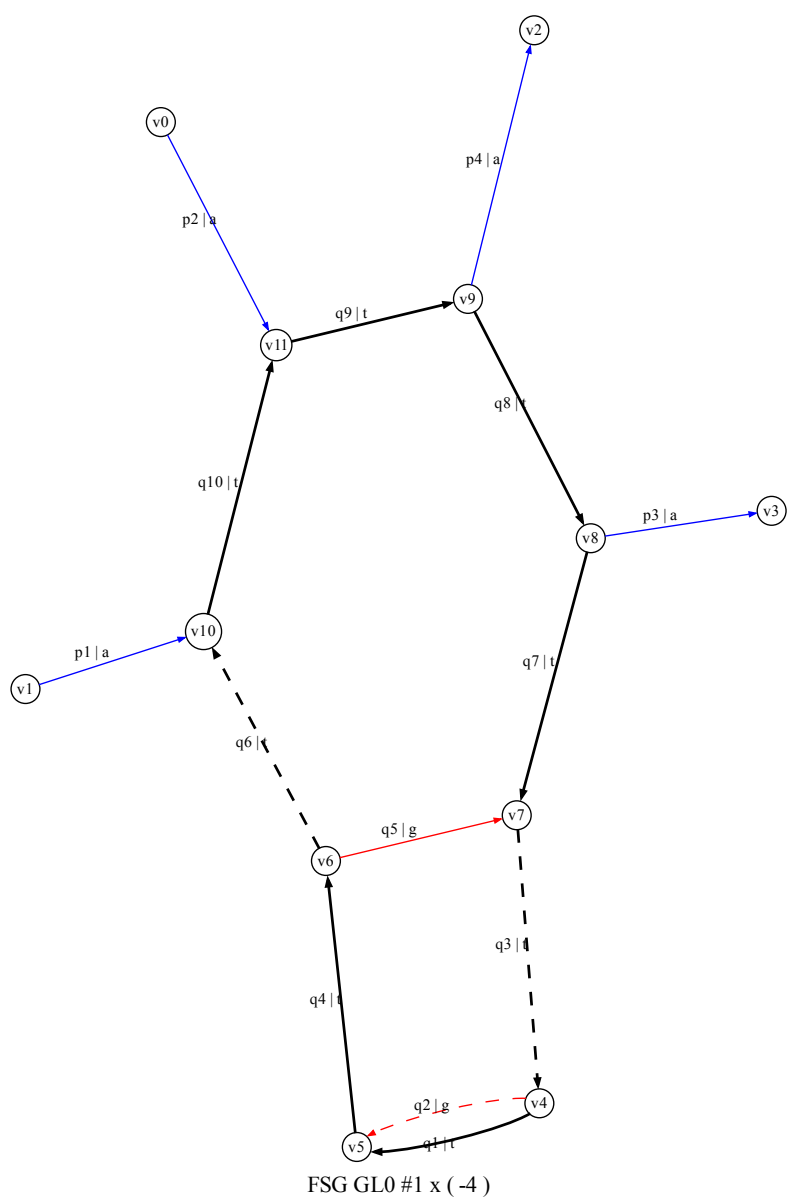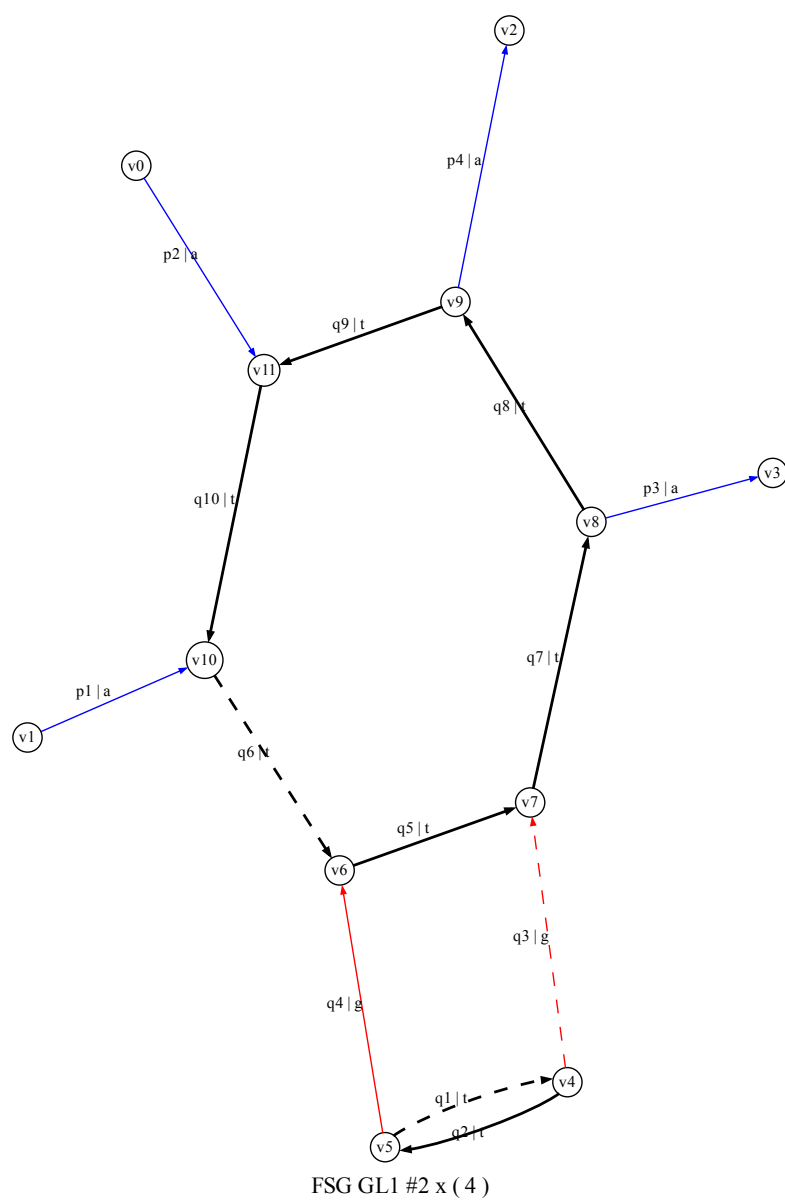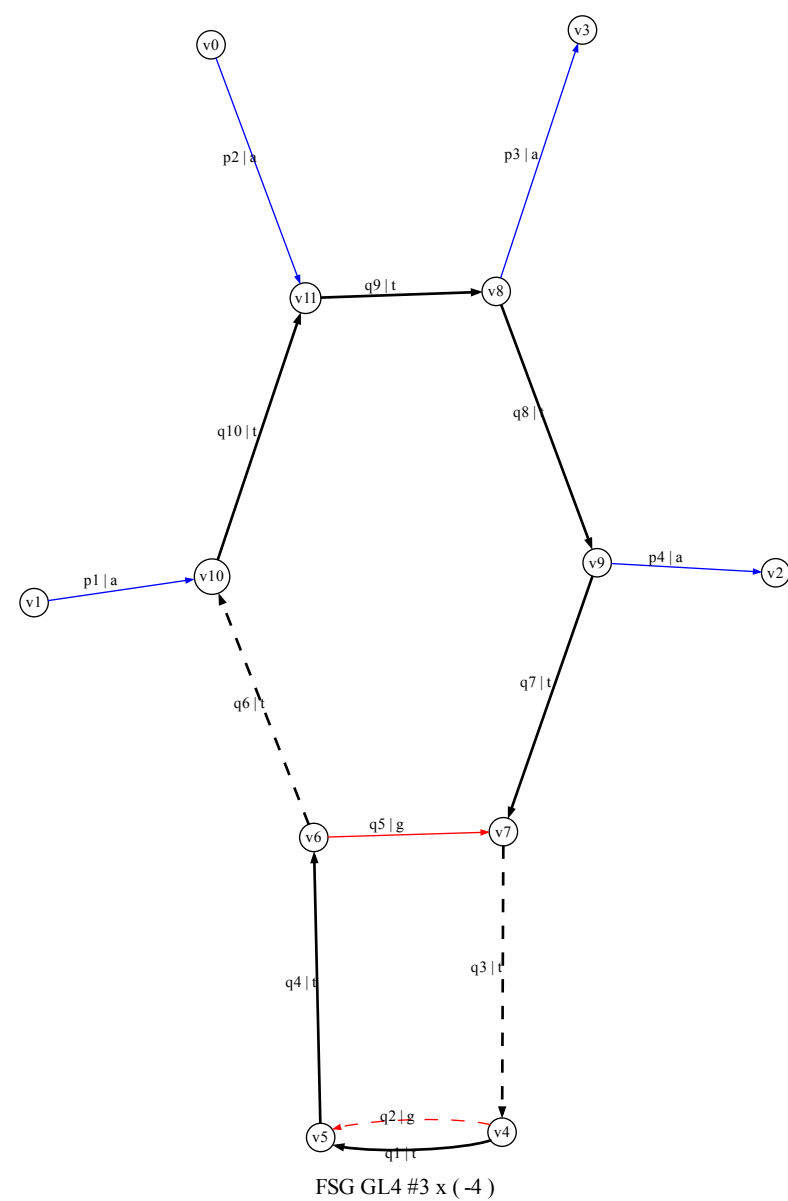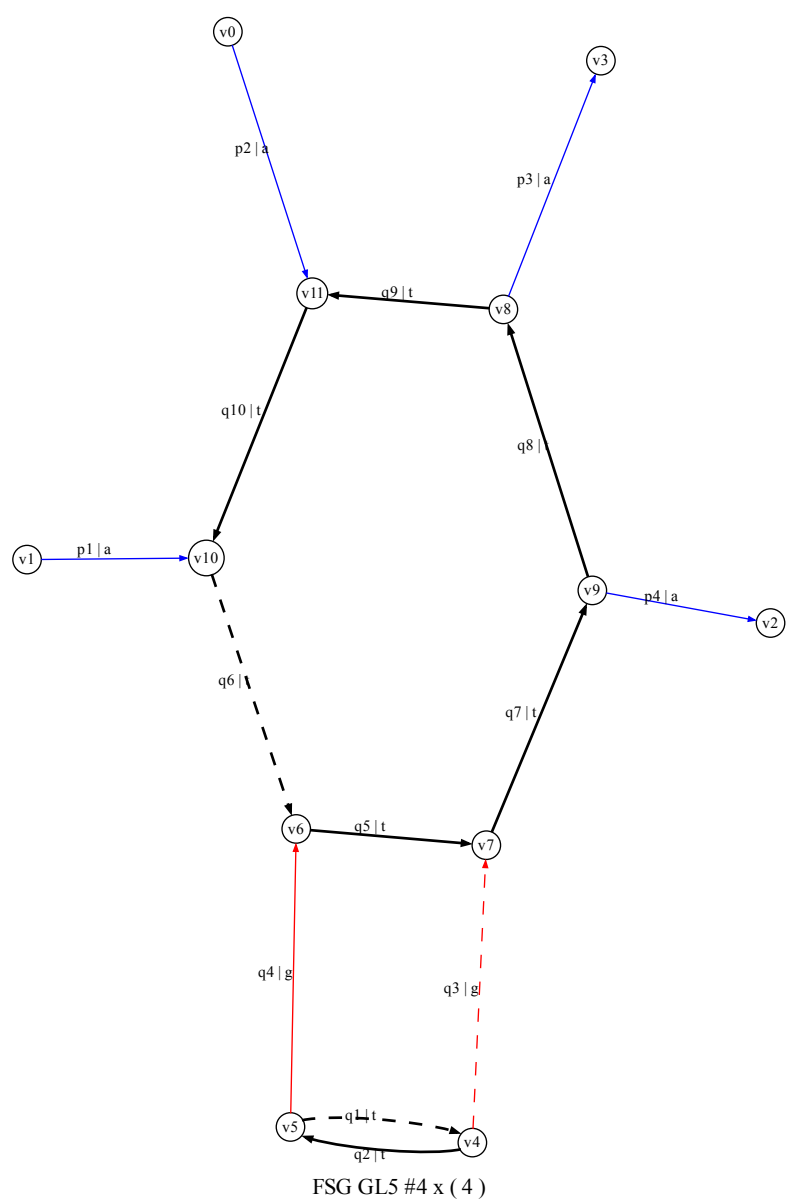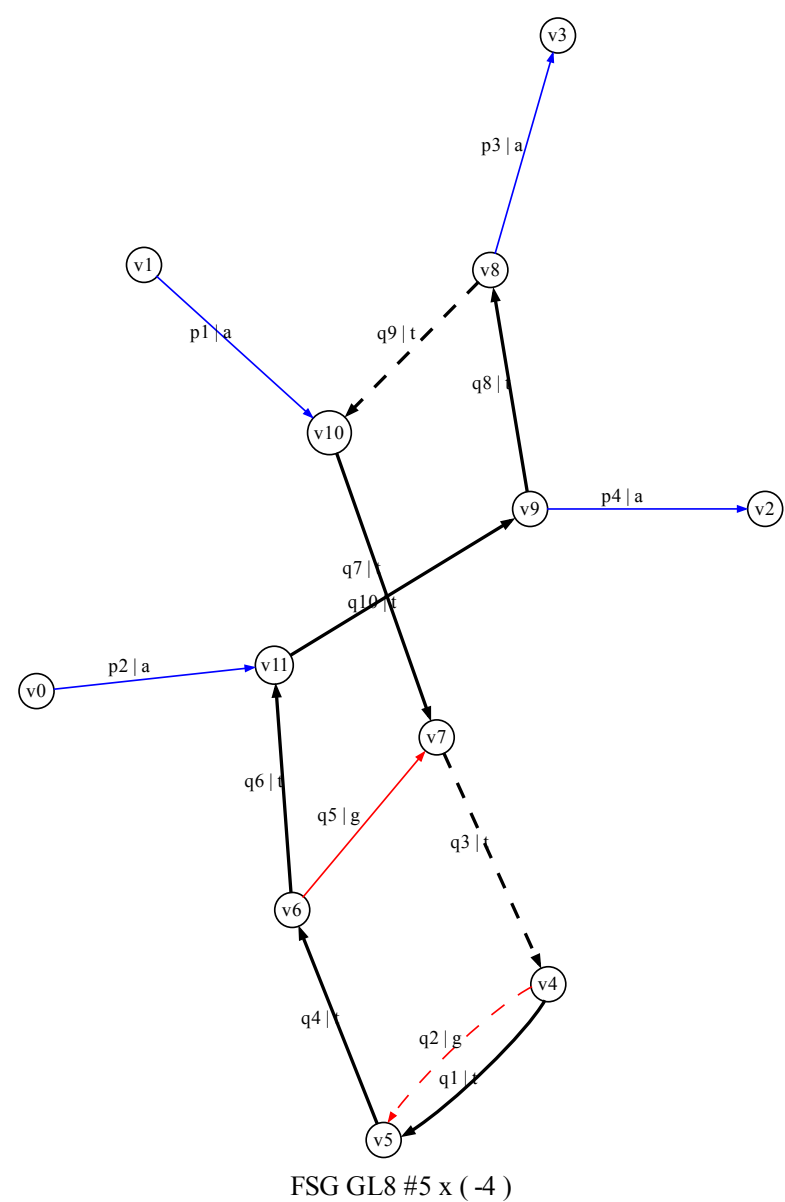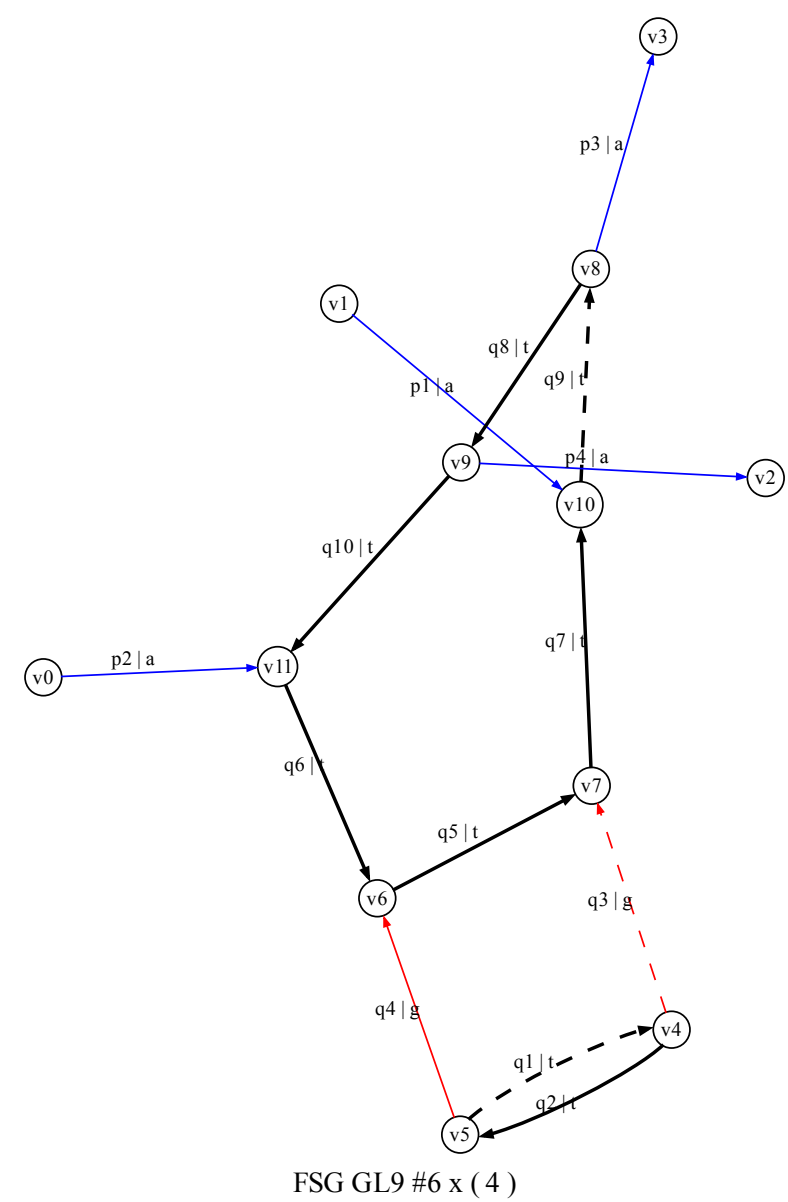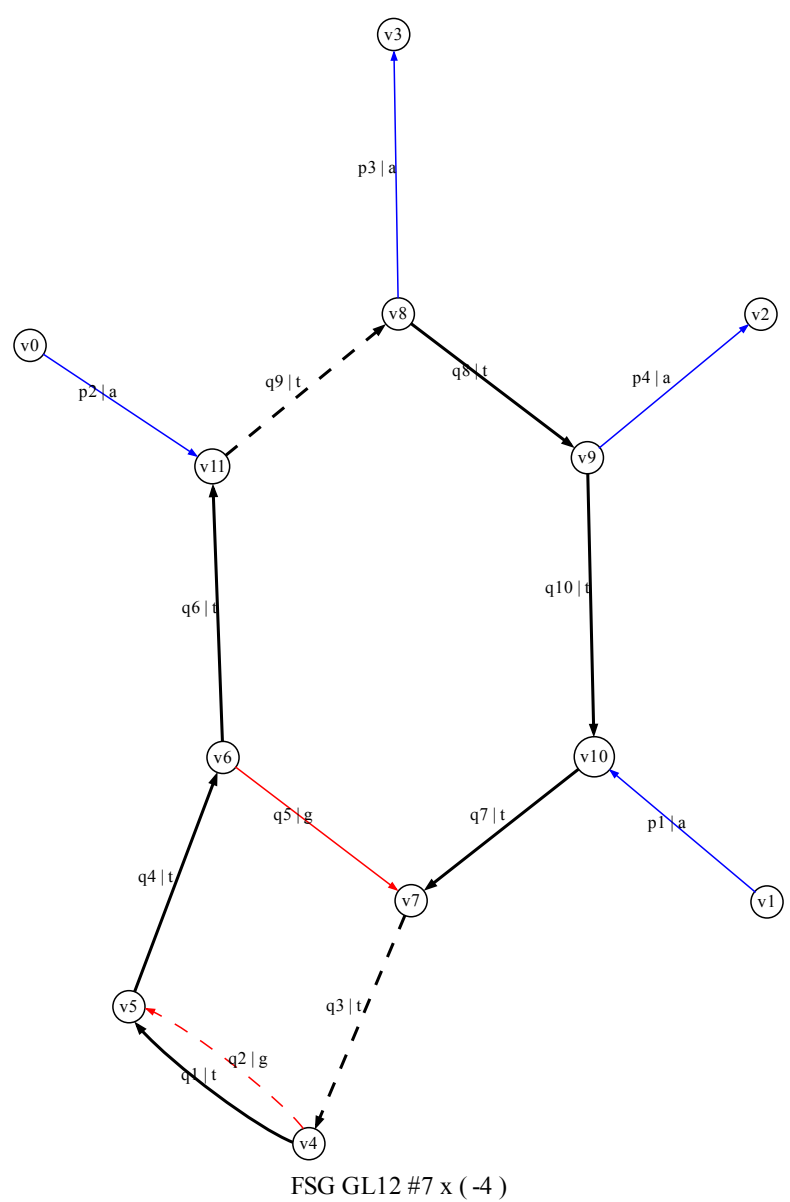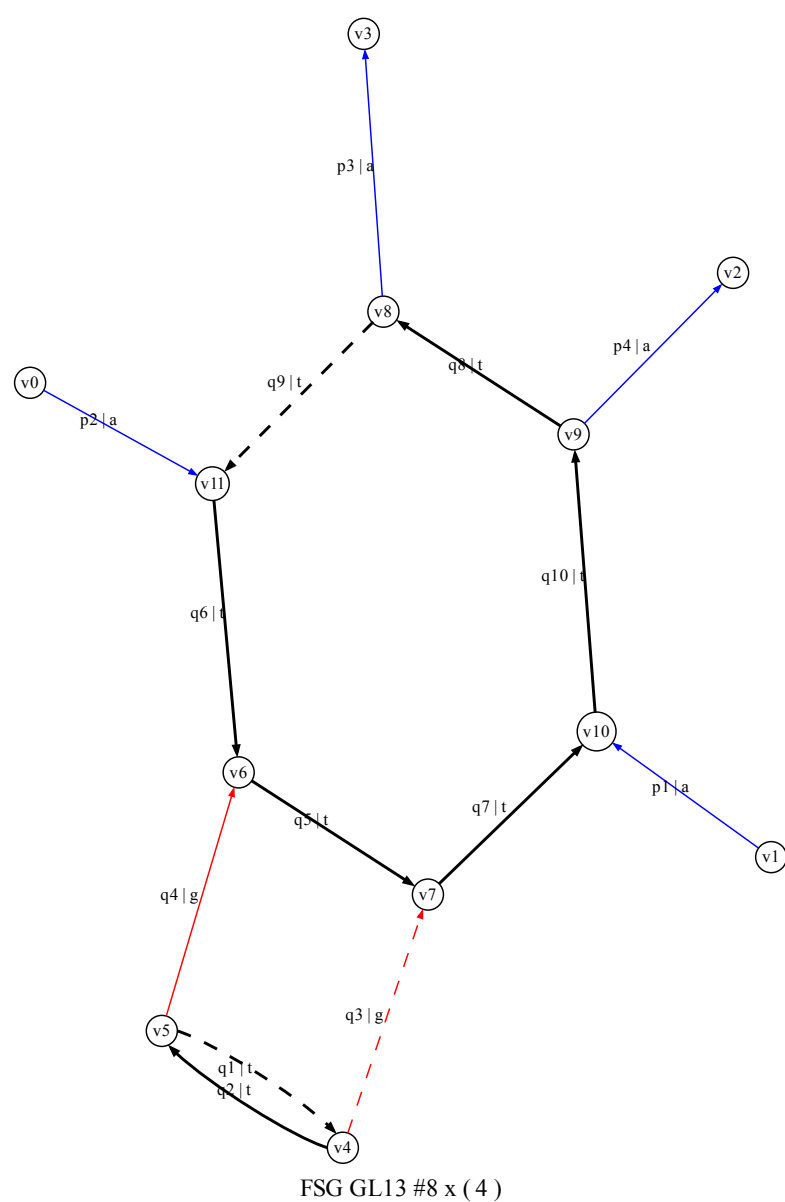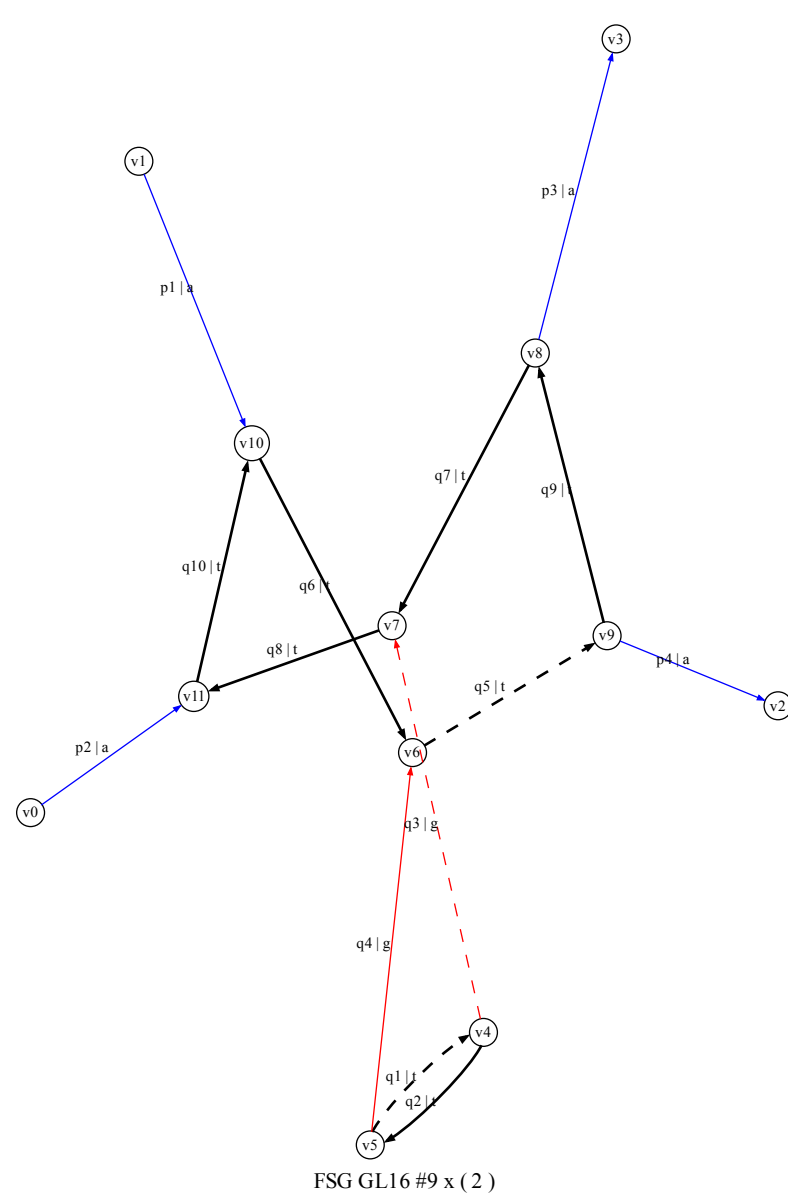

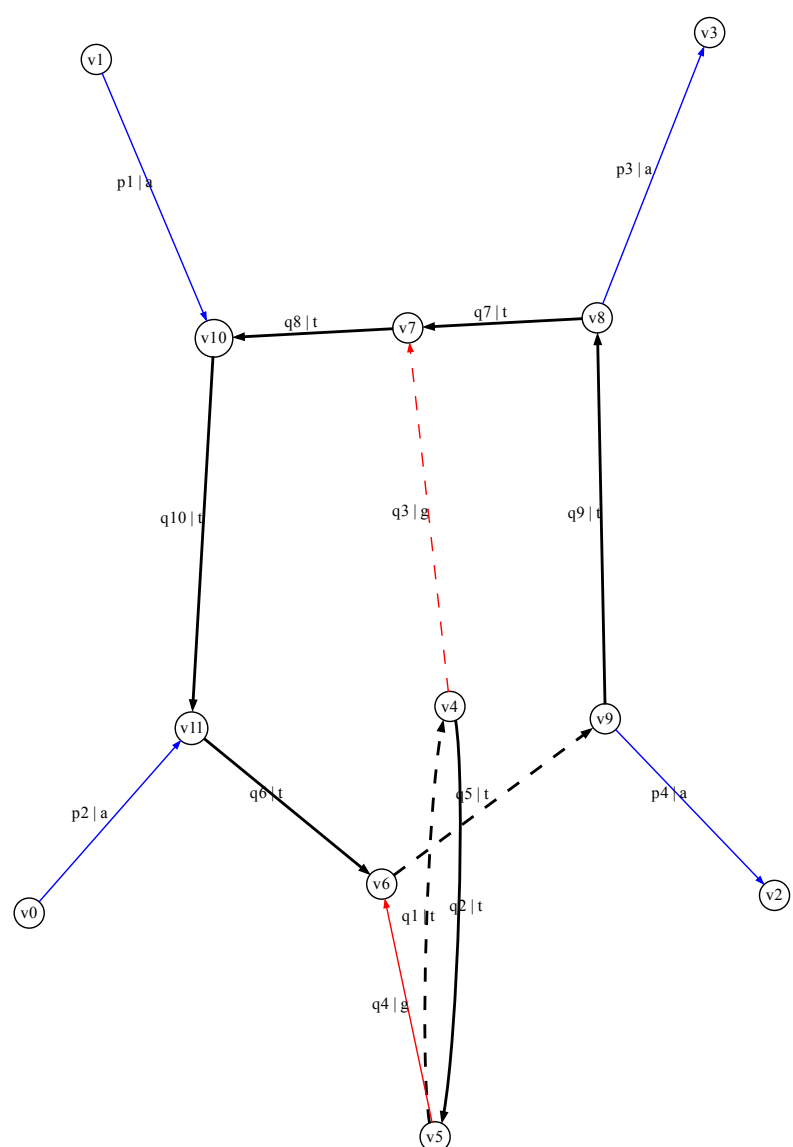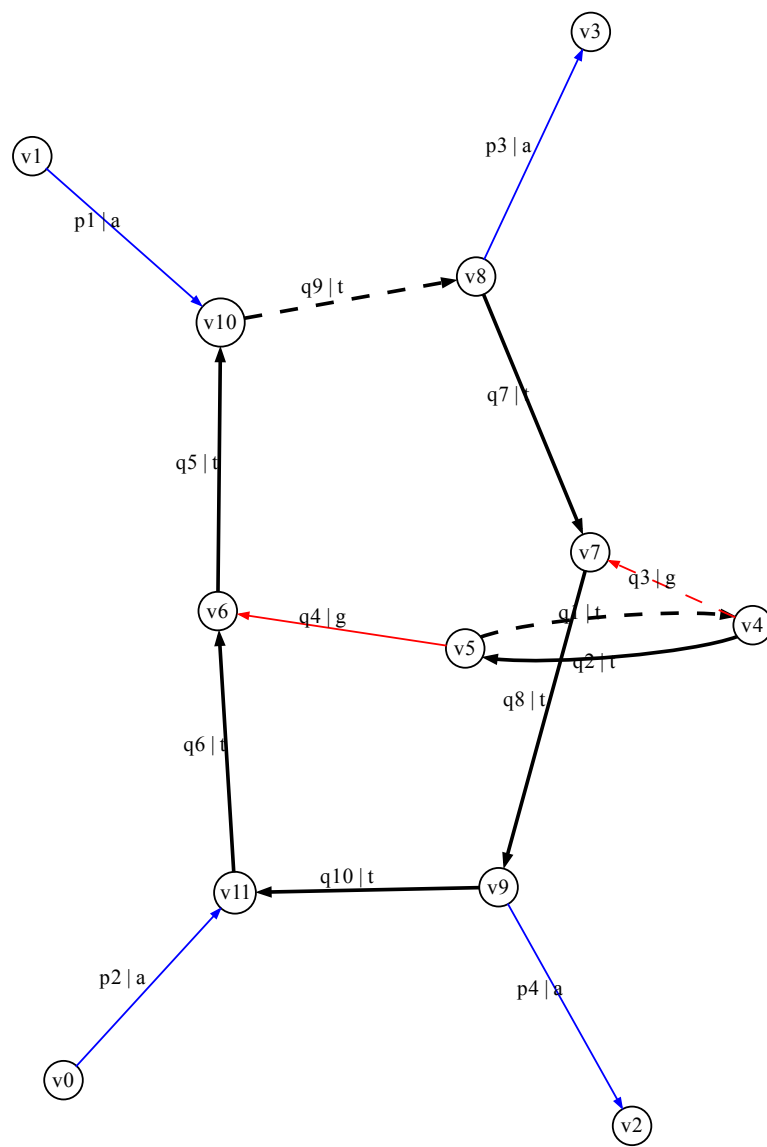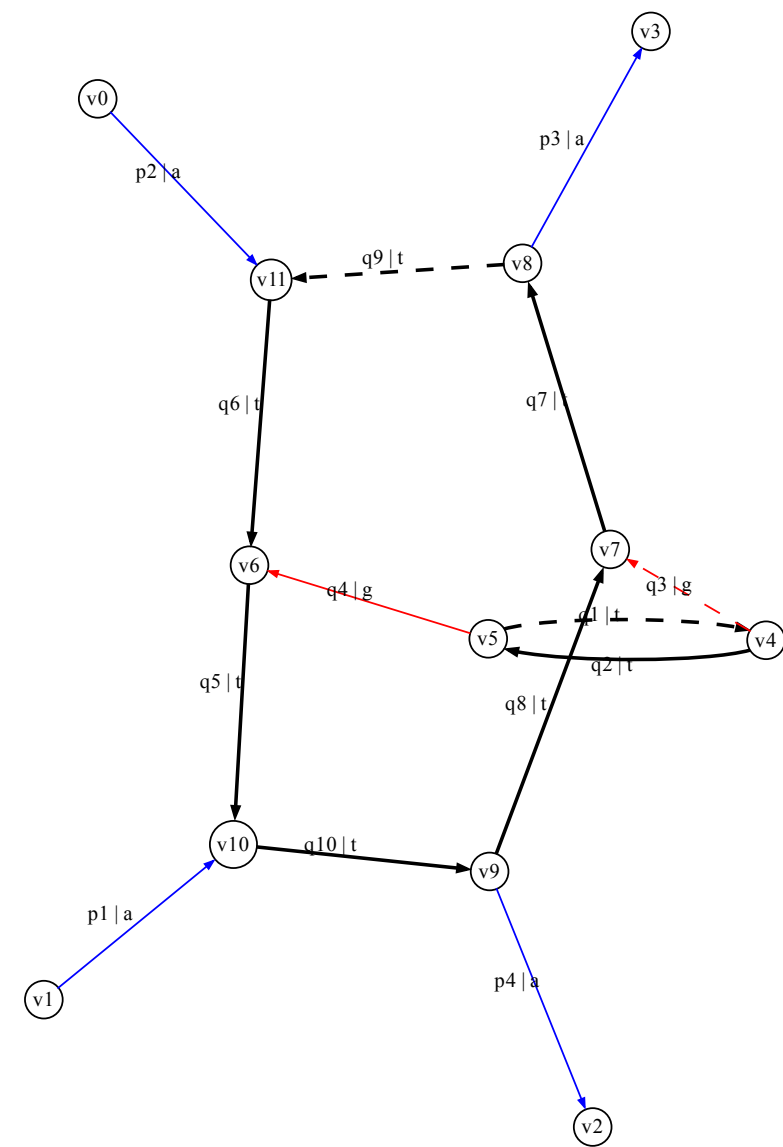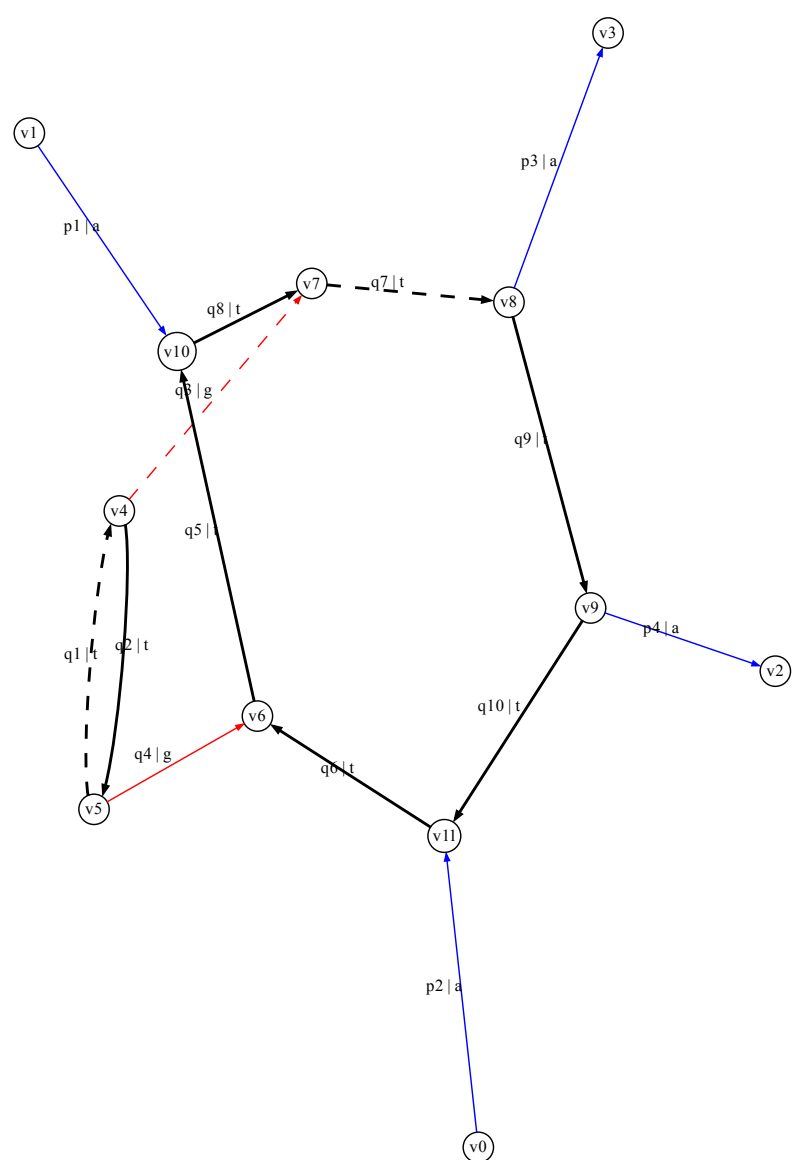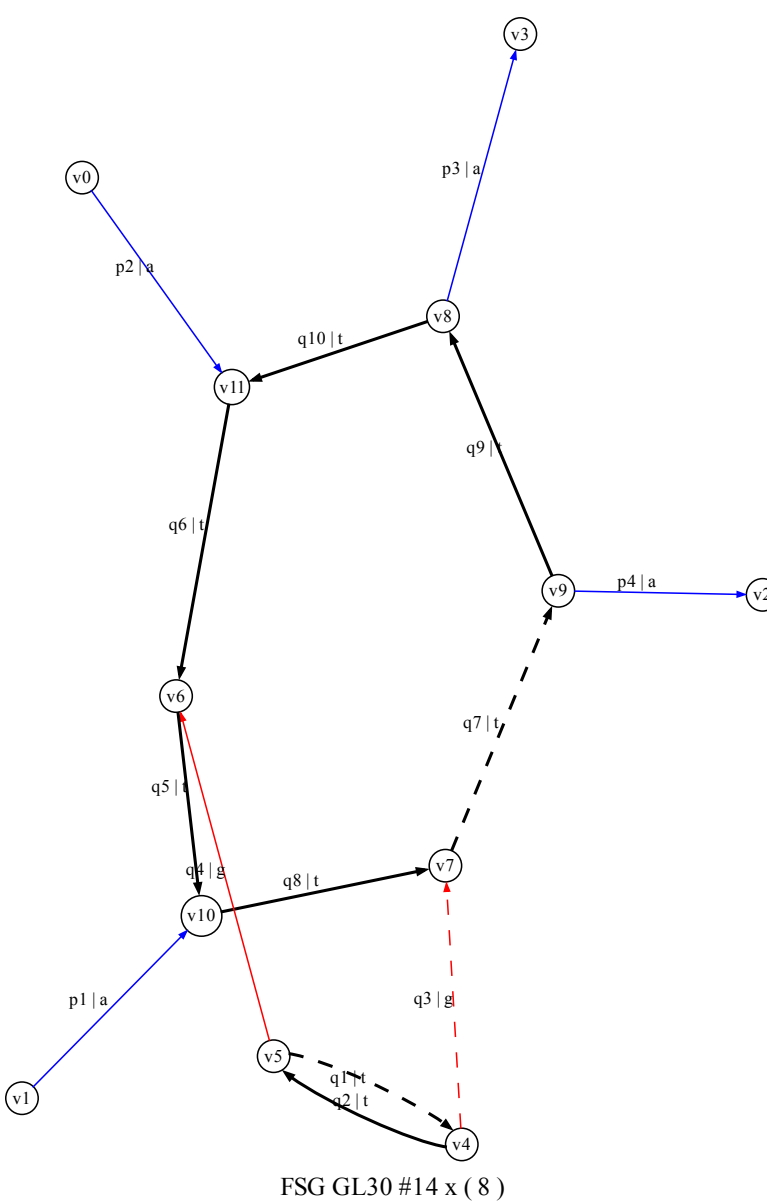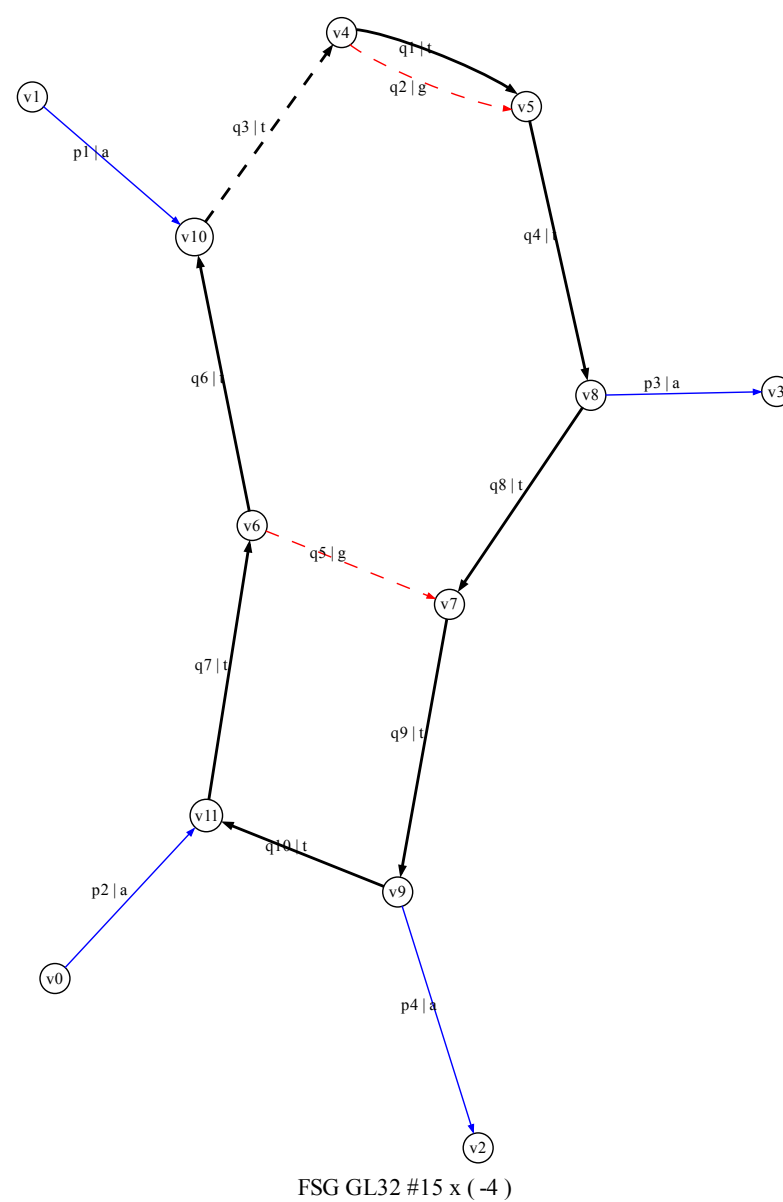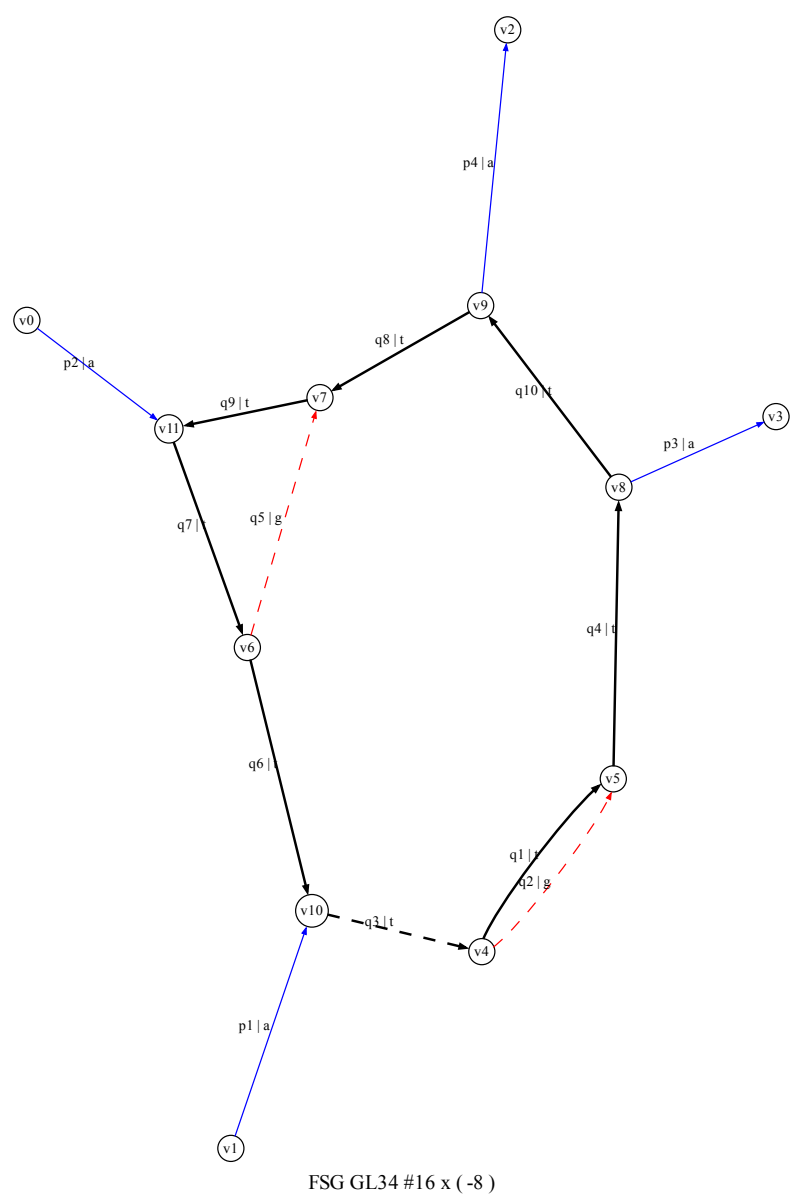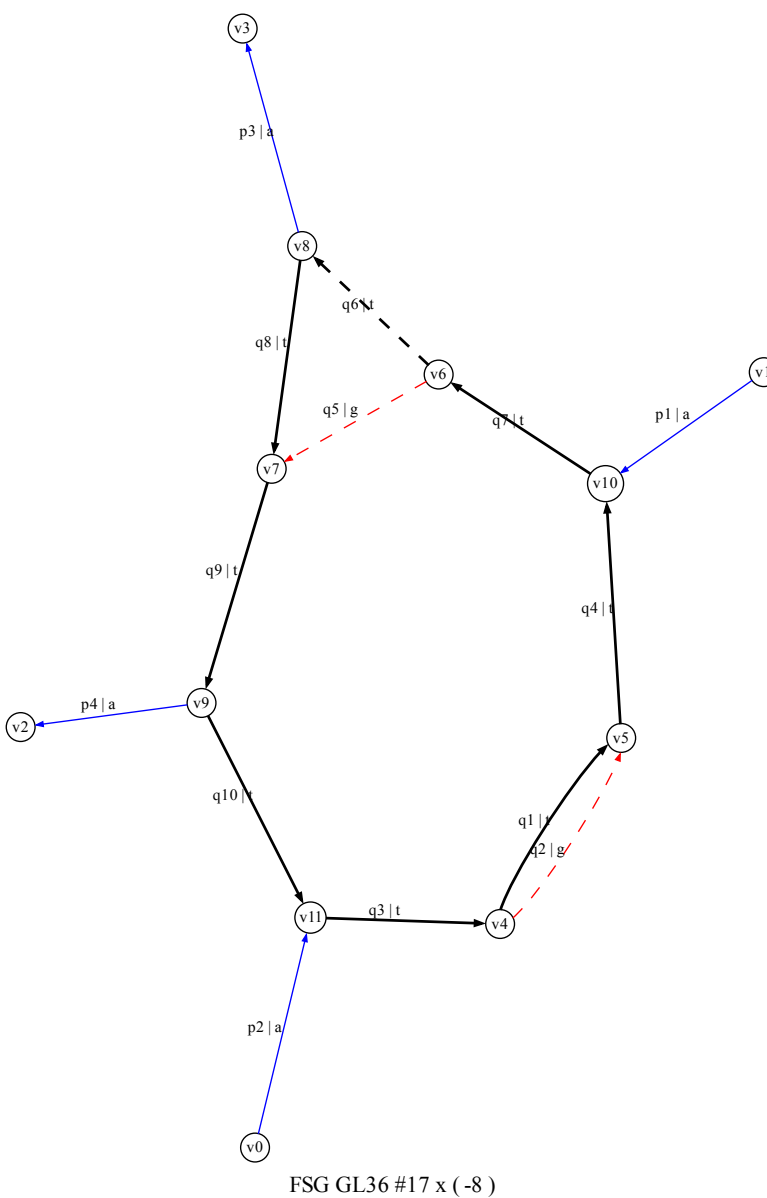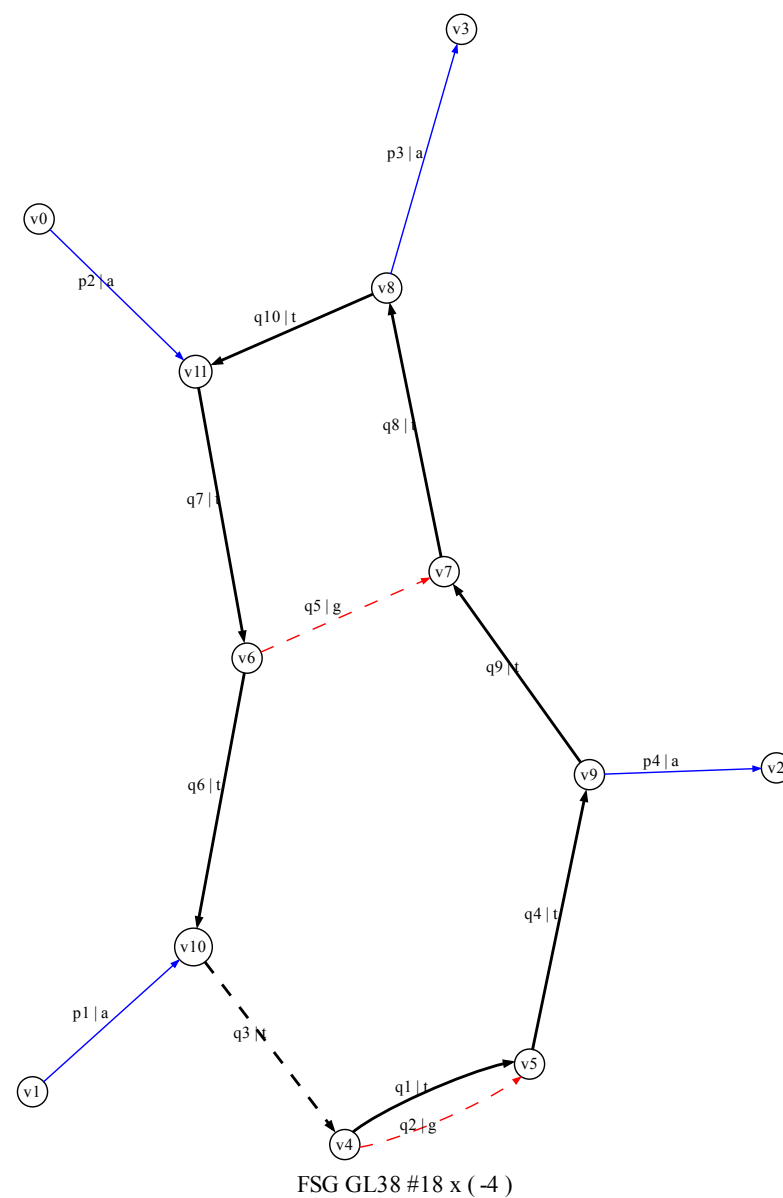

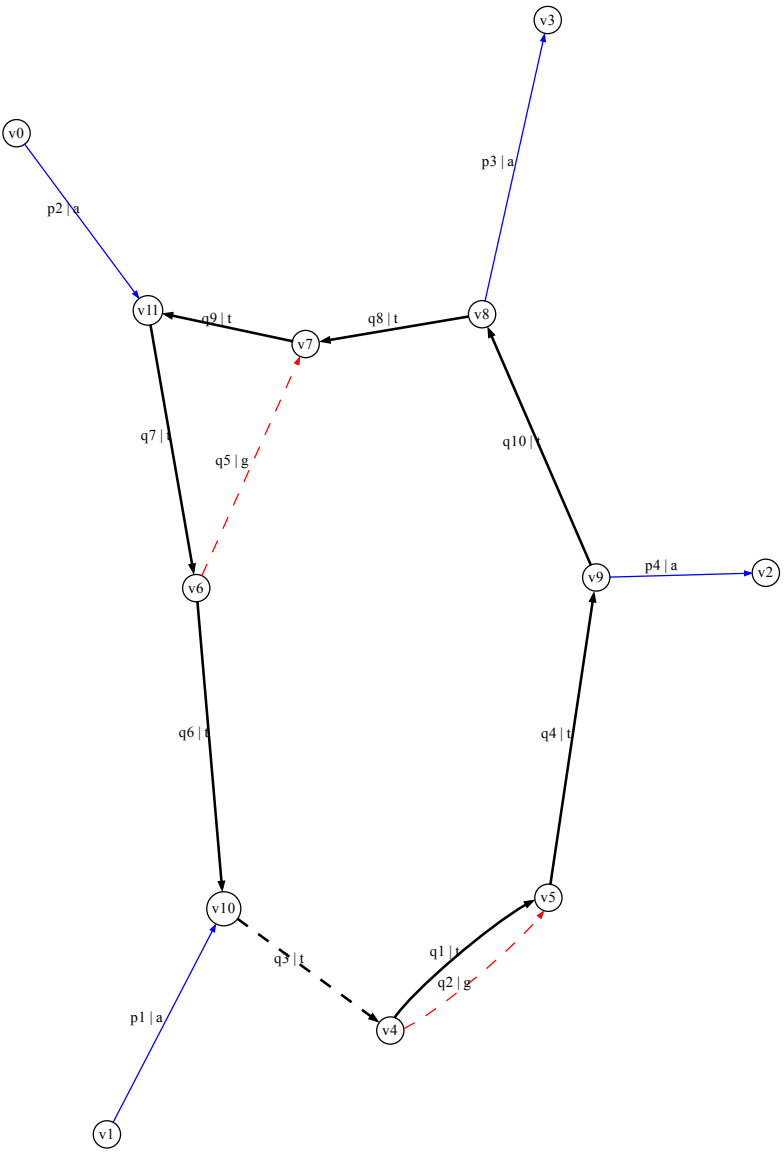

FSG GL40 #19 x (-8 )

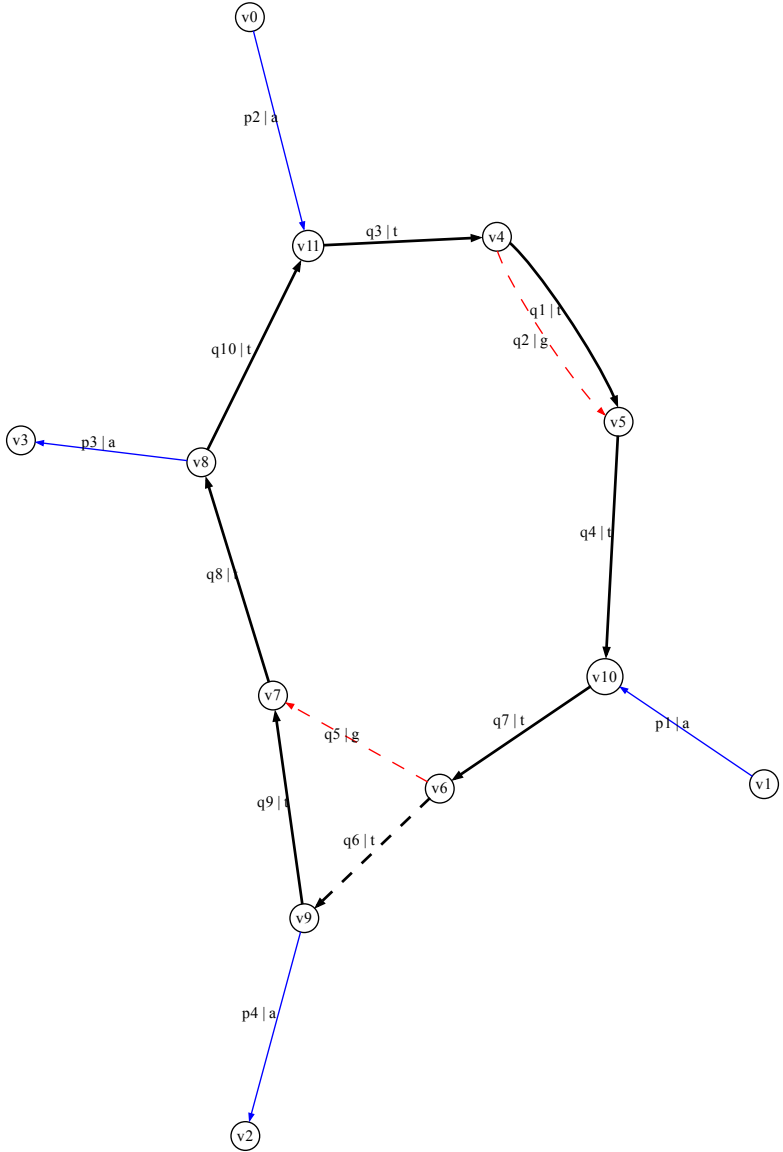

FSG GL42 #20 x (-8 )

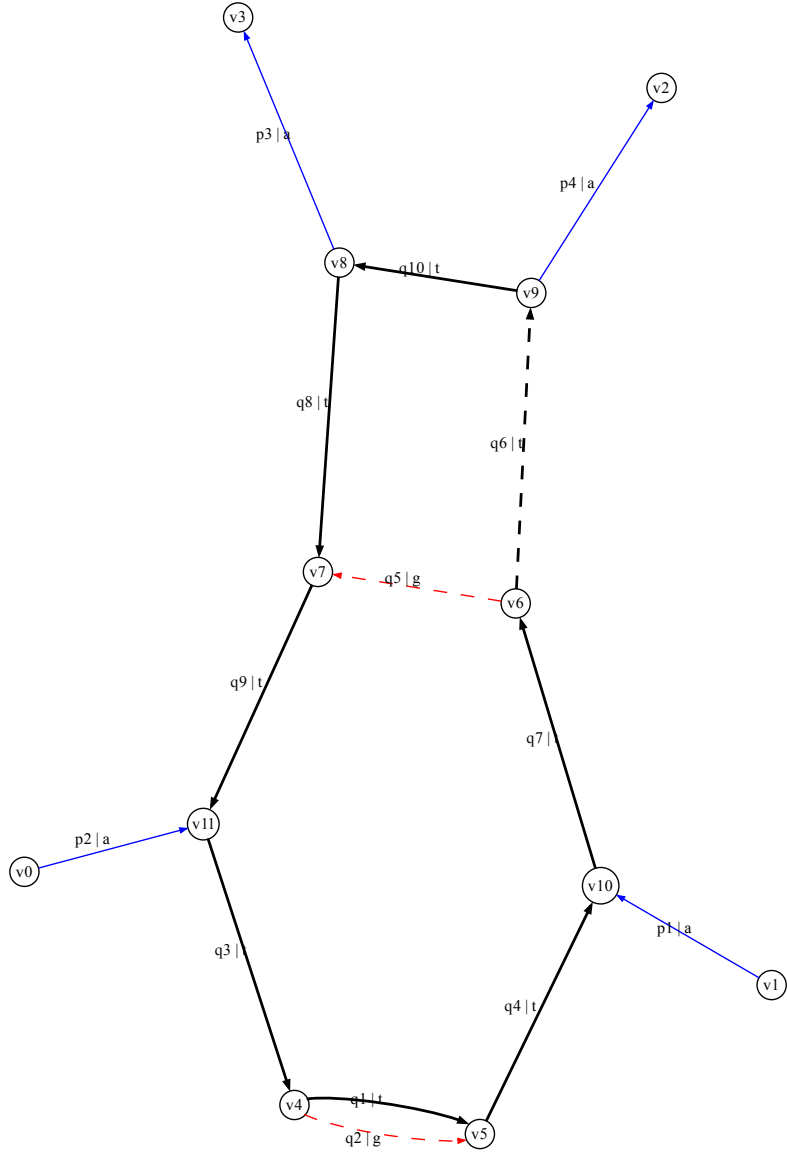

FSG GL44 #21 x (-4 )

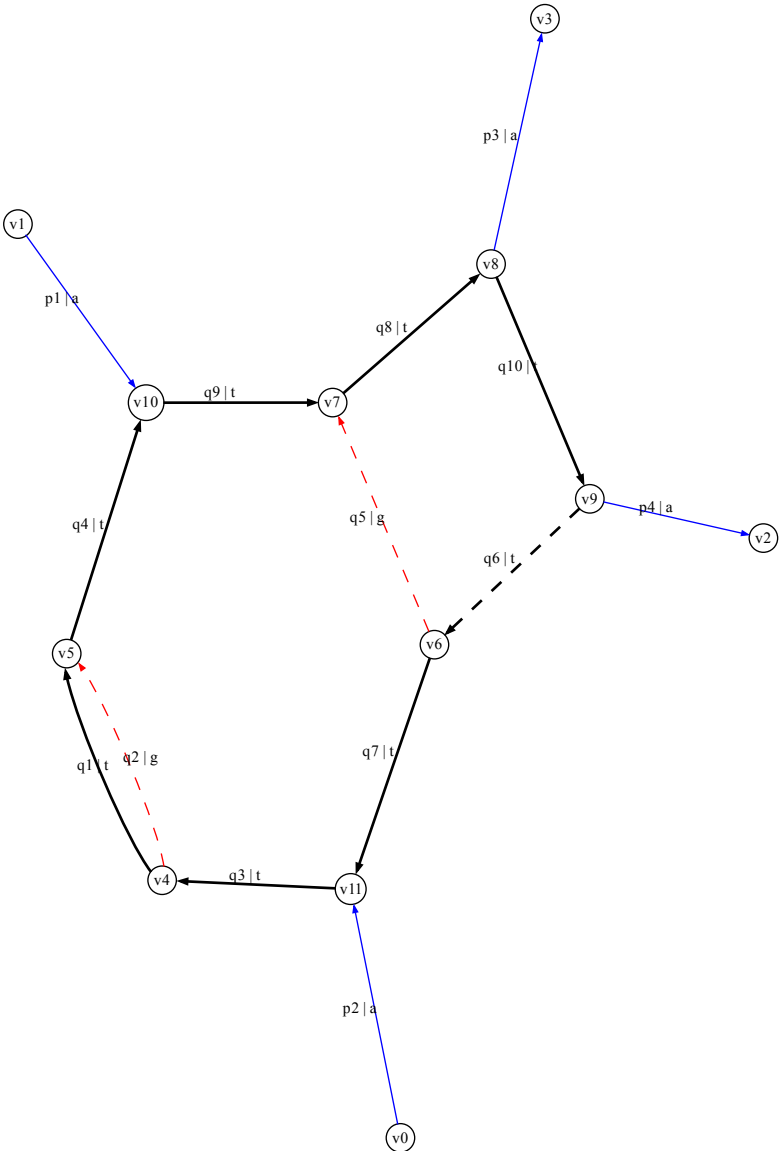

FSG GL46 #22 x (-4 )

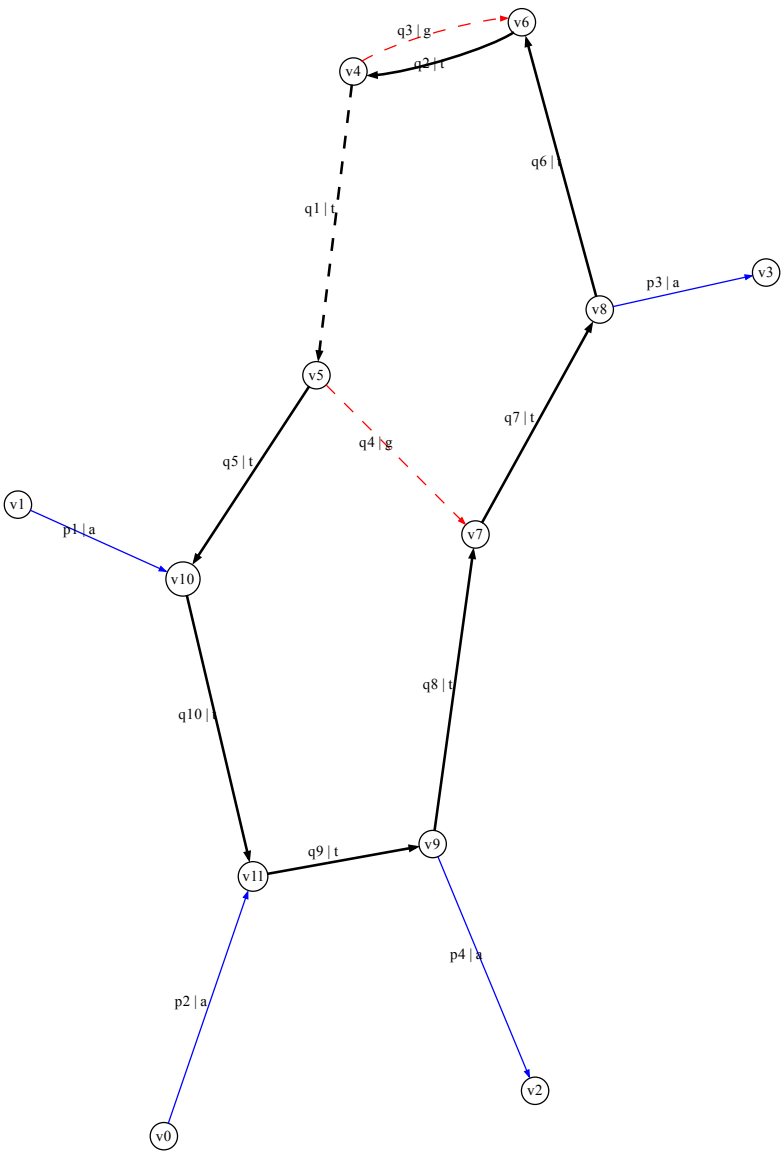

FSG GL80 #23 x (-8 )

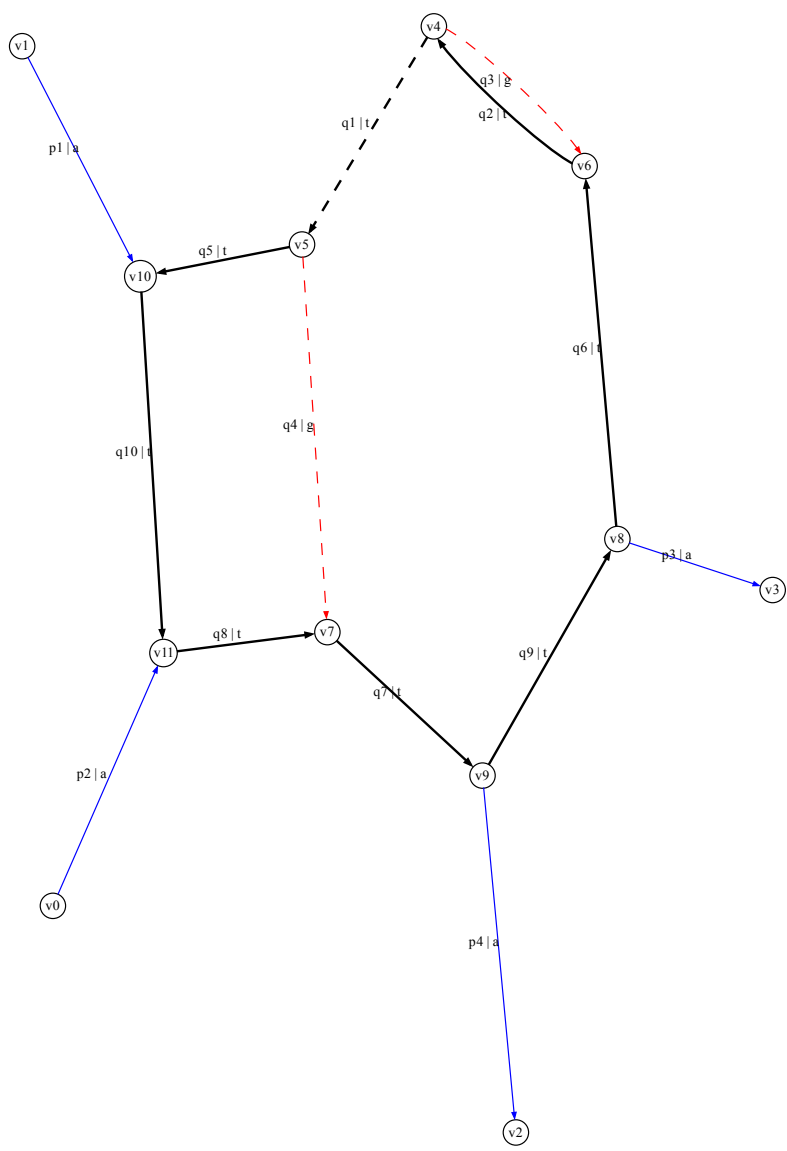

FSG GL82 #24 x (-8 )

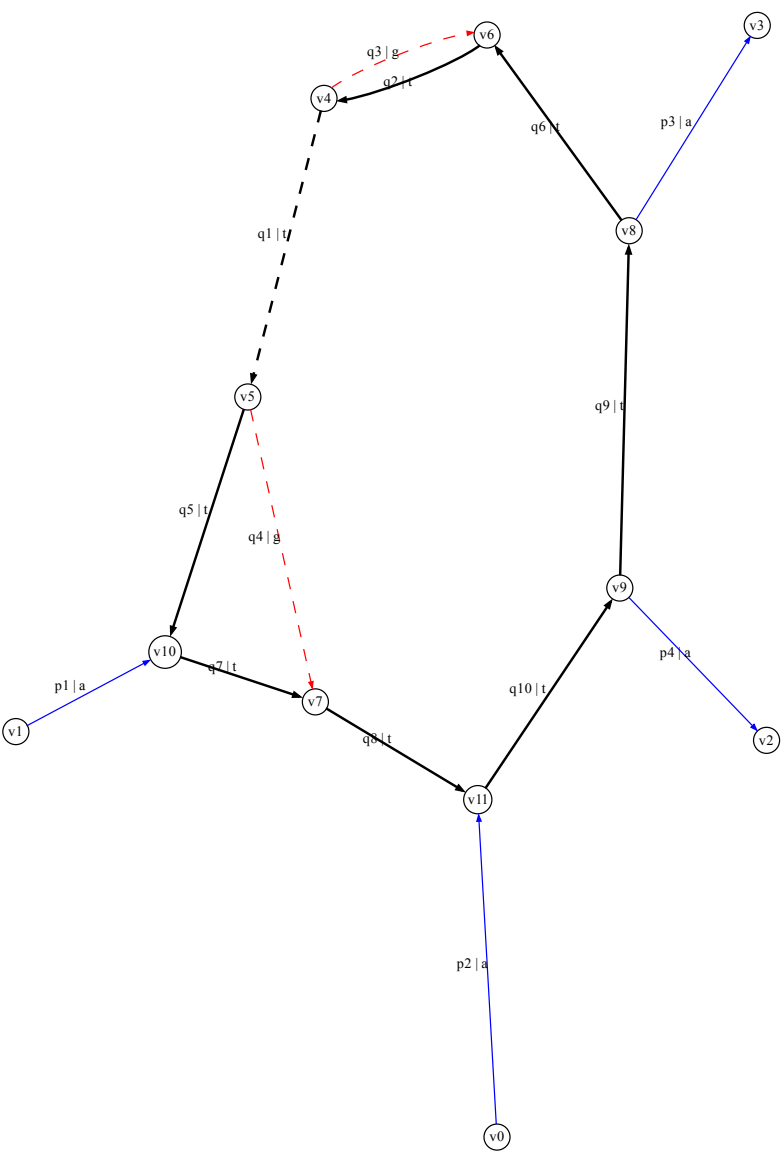

FSG GL84 #25 x (-8 )

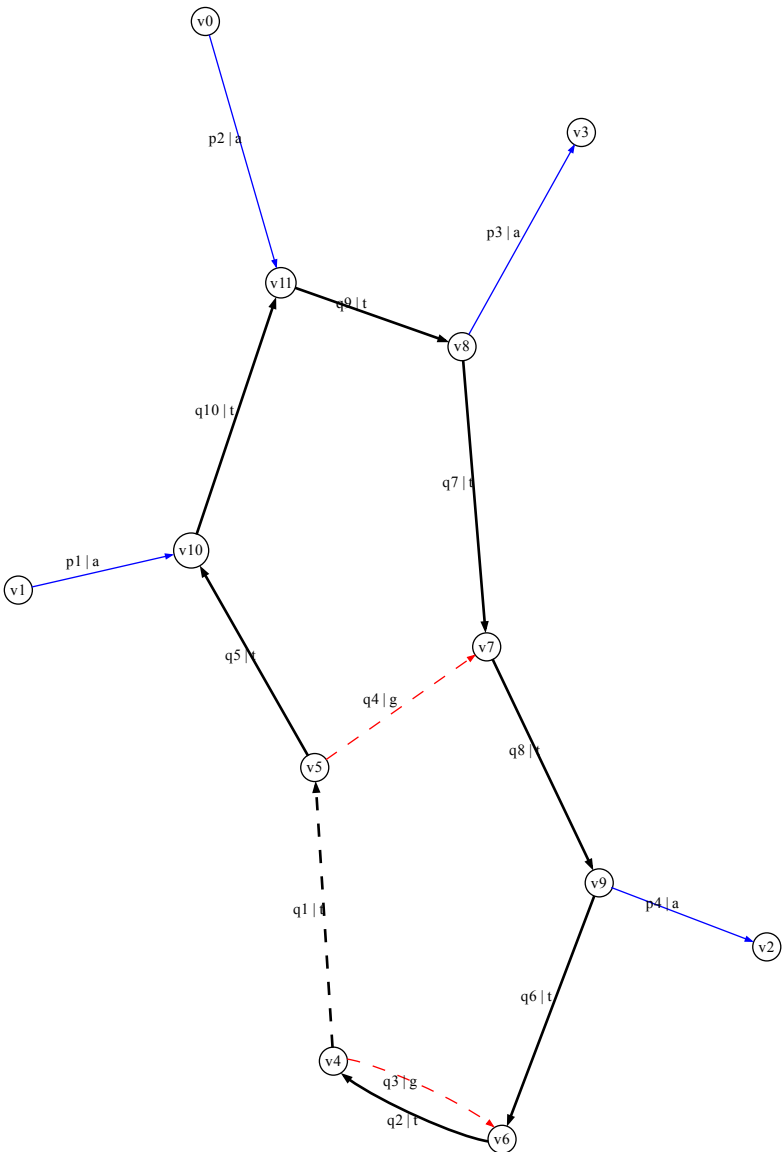

FSG GL86 #26 x (-8 )

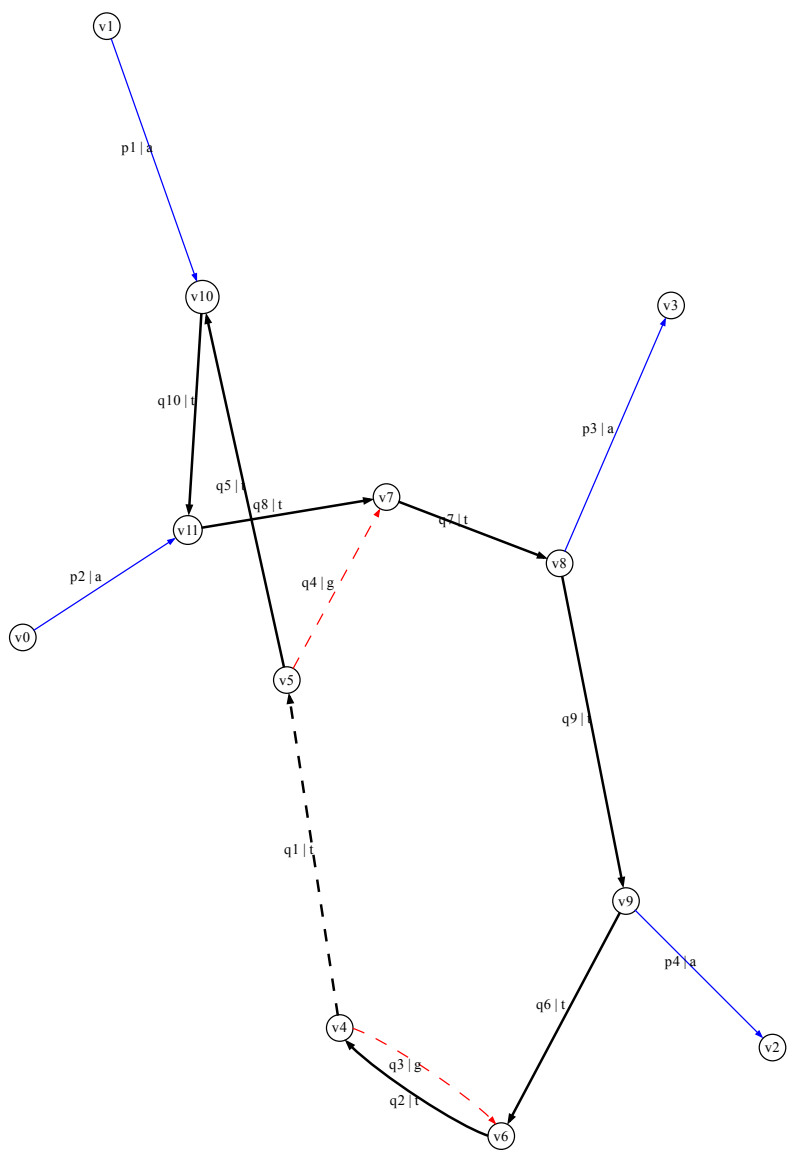

FSG GL88 #27 x (-8 )

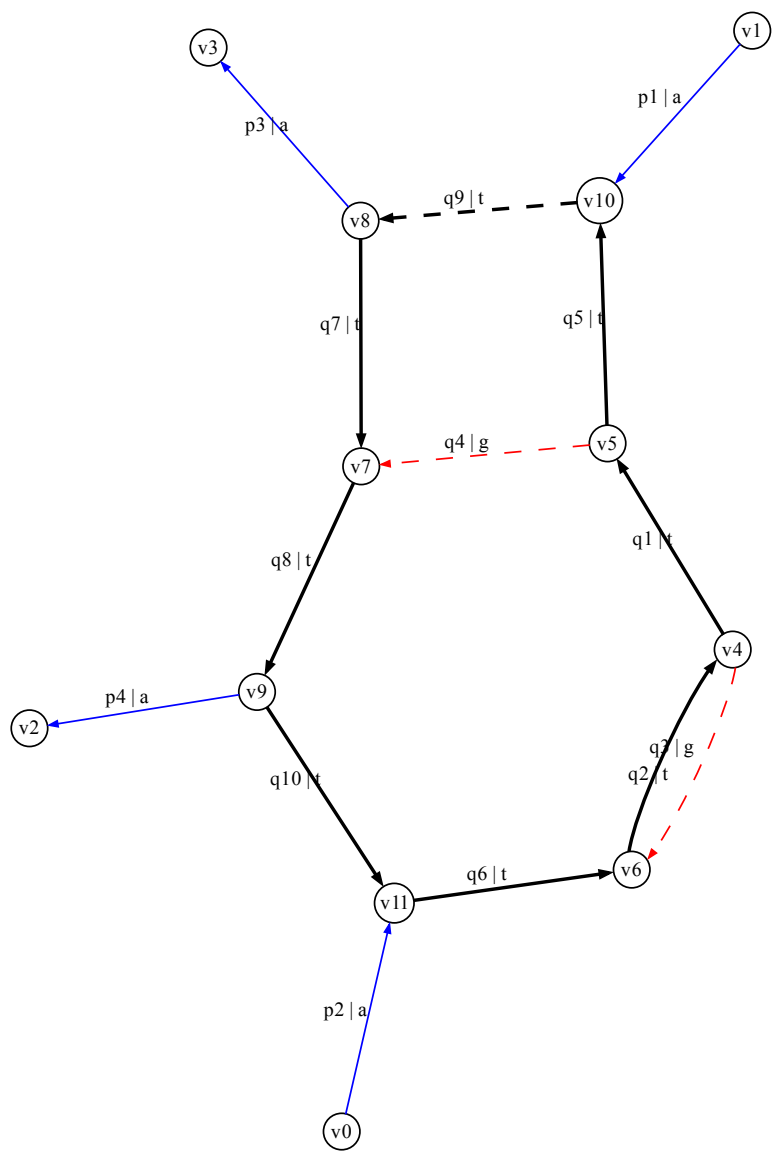

FSG GL94 #28 x (-8)

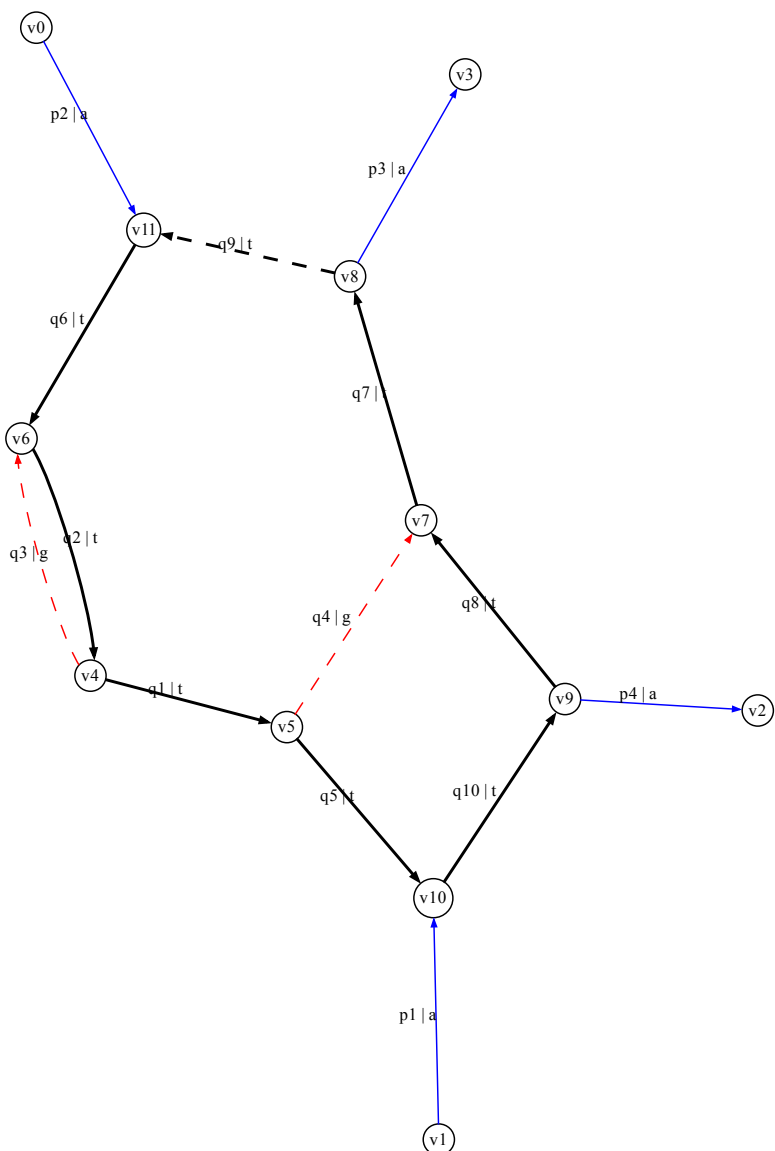

FSG GL96 #29 x (-8)

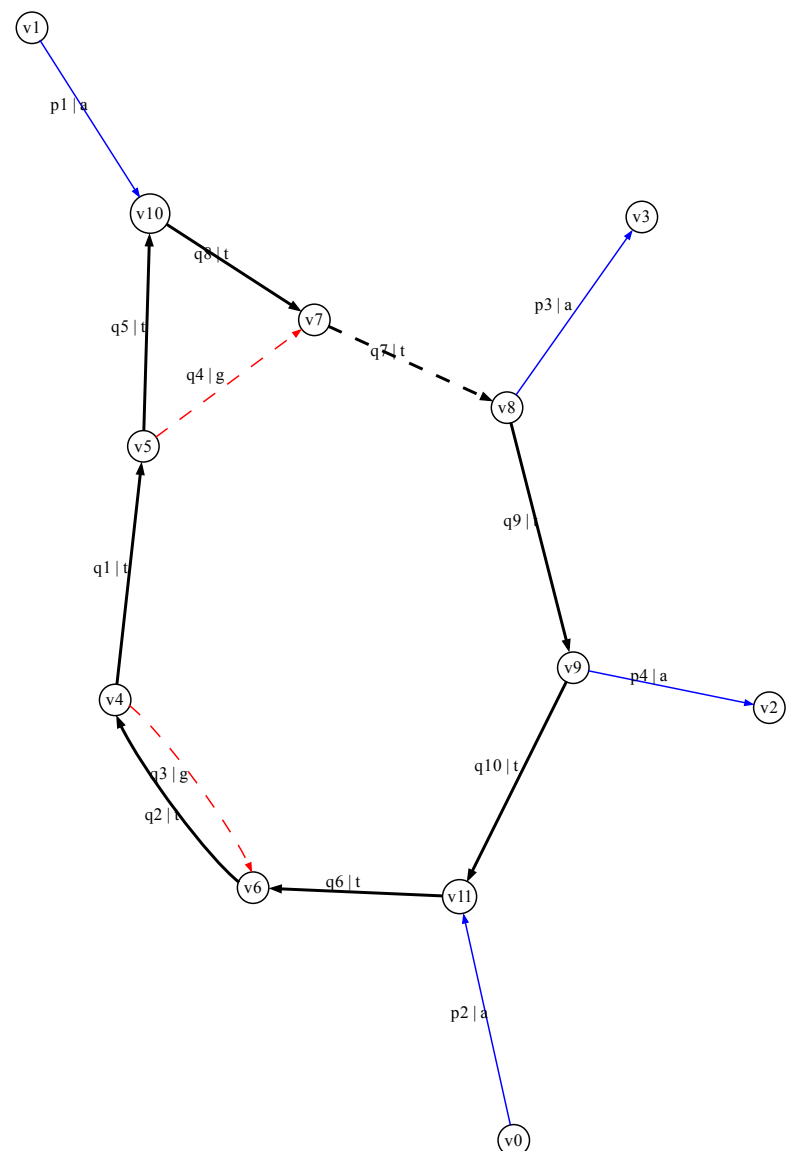

FSG GL98 #30 x (-8)

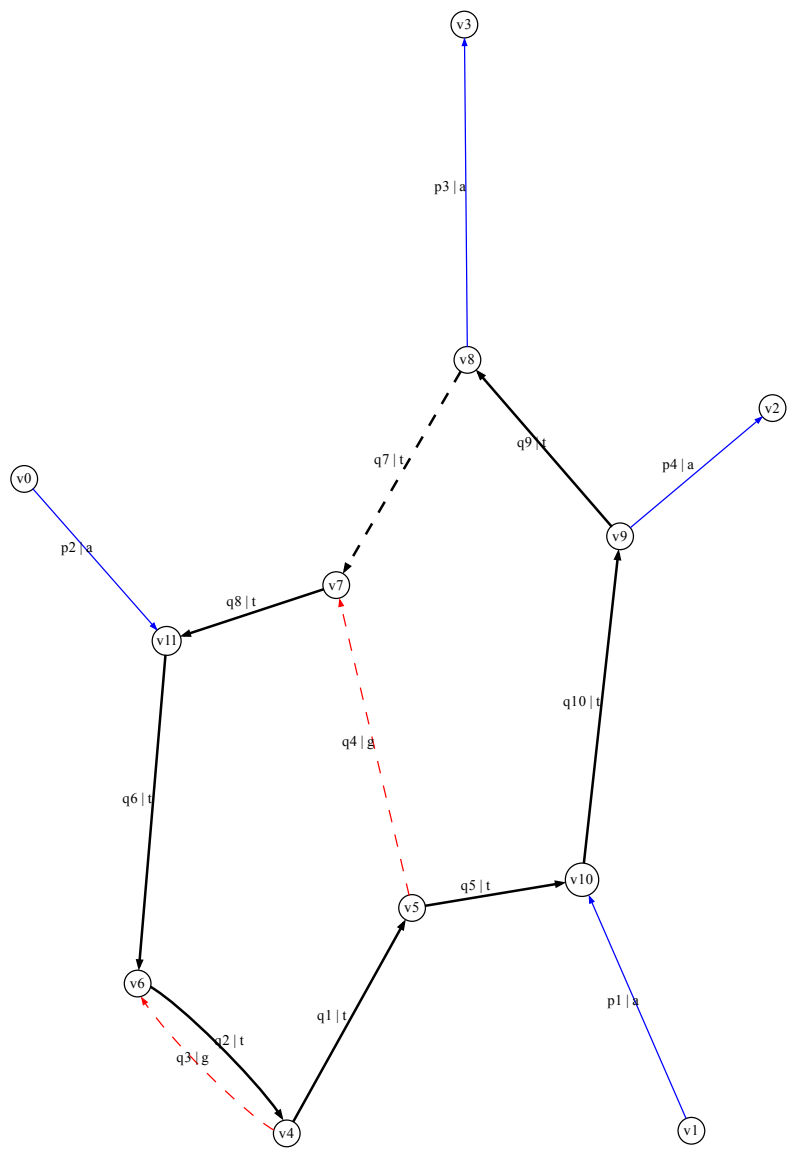

FSG GL100 #31 x (-8)

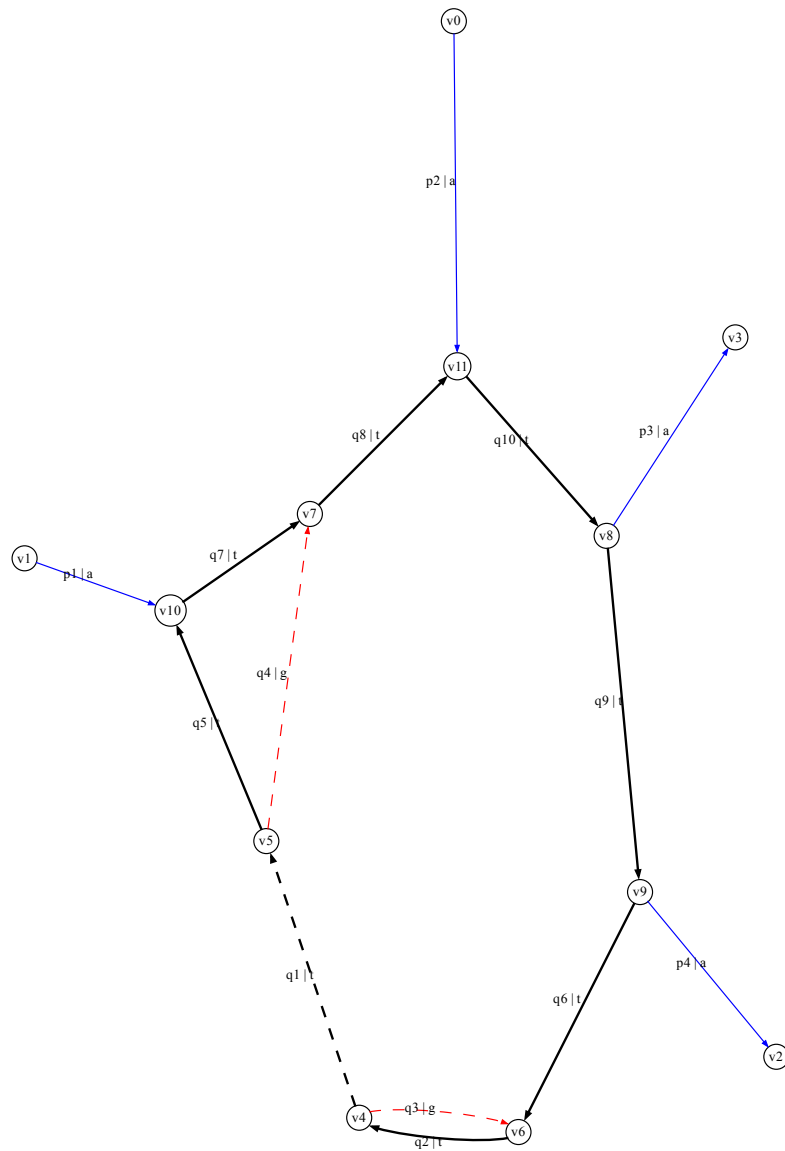

FSG GL102 #32 x (-8)

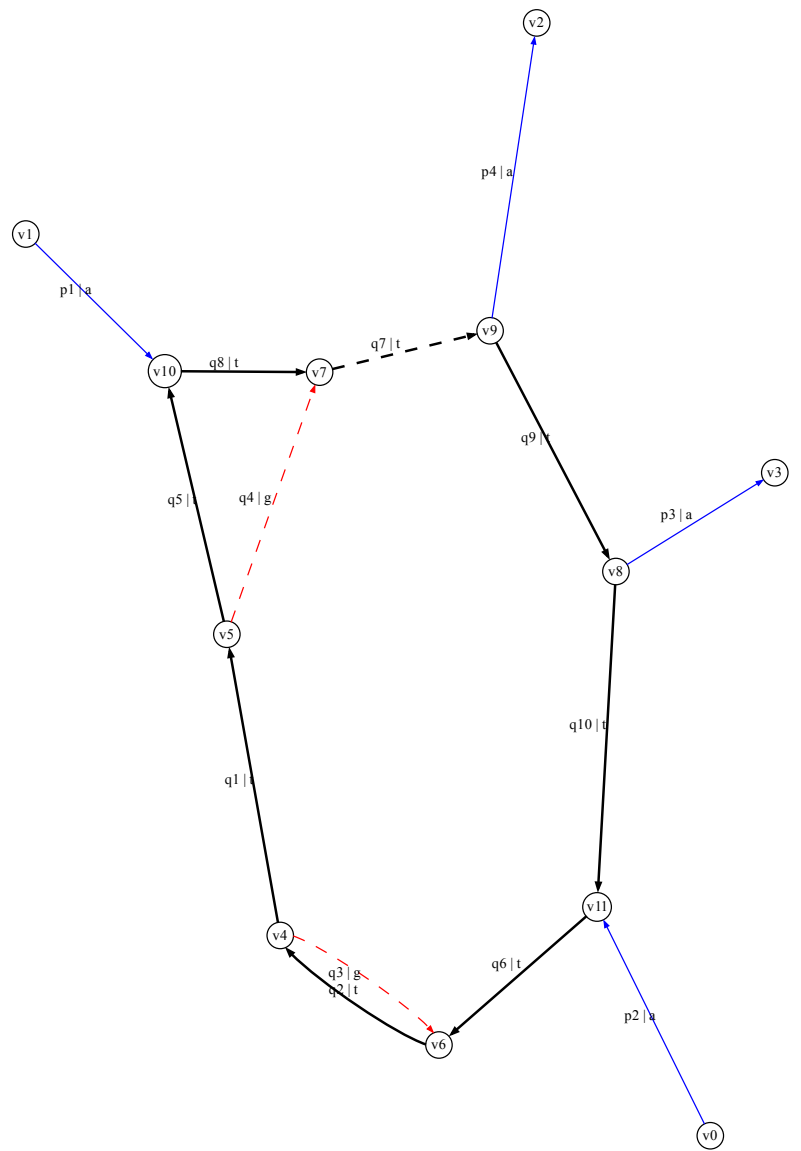

FSG GL104 #33 x (-8)

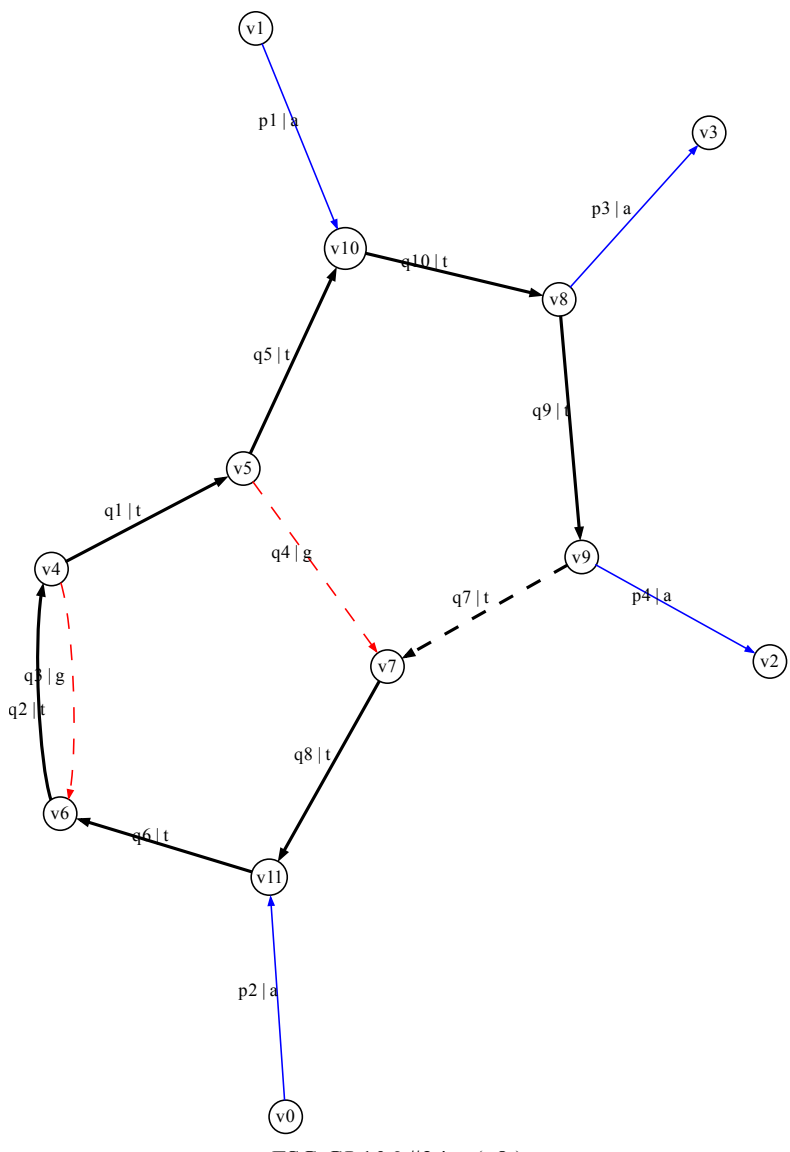

FSG GL106 #34 x (-8)

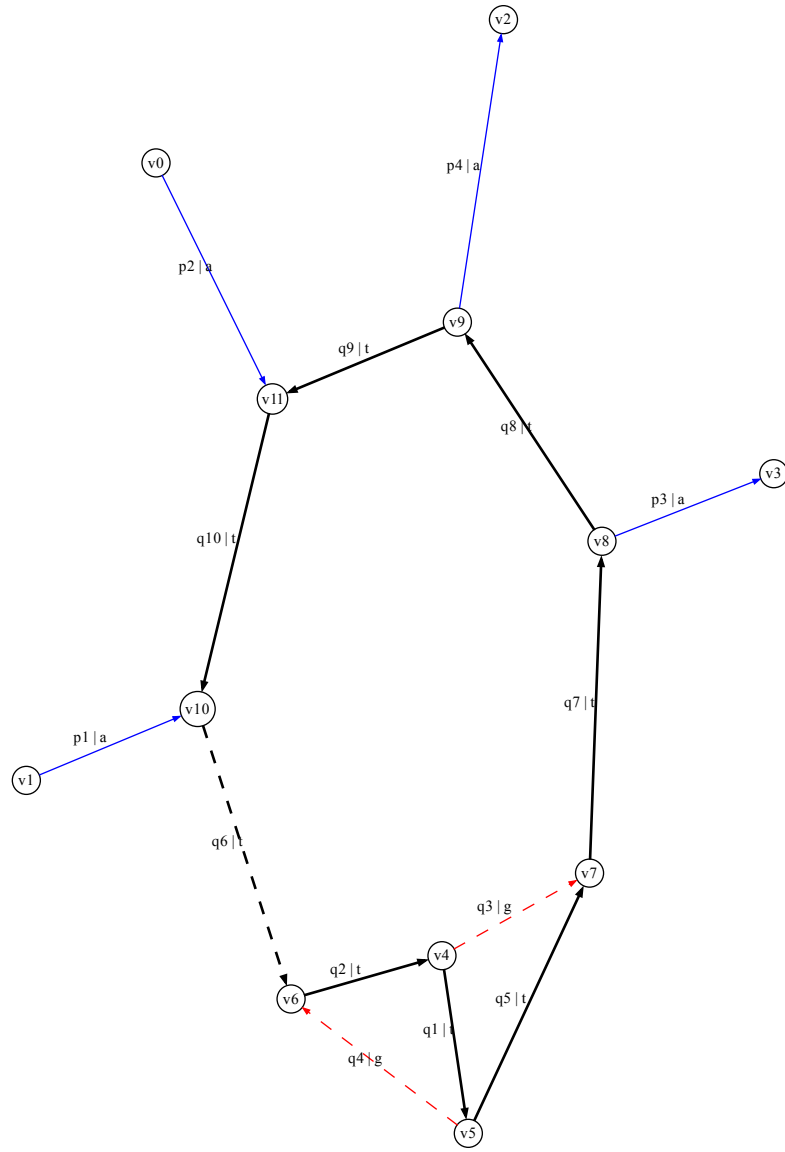

FSG GL112 #35 x (-4)

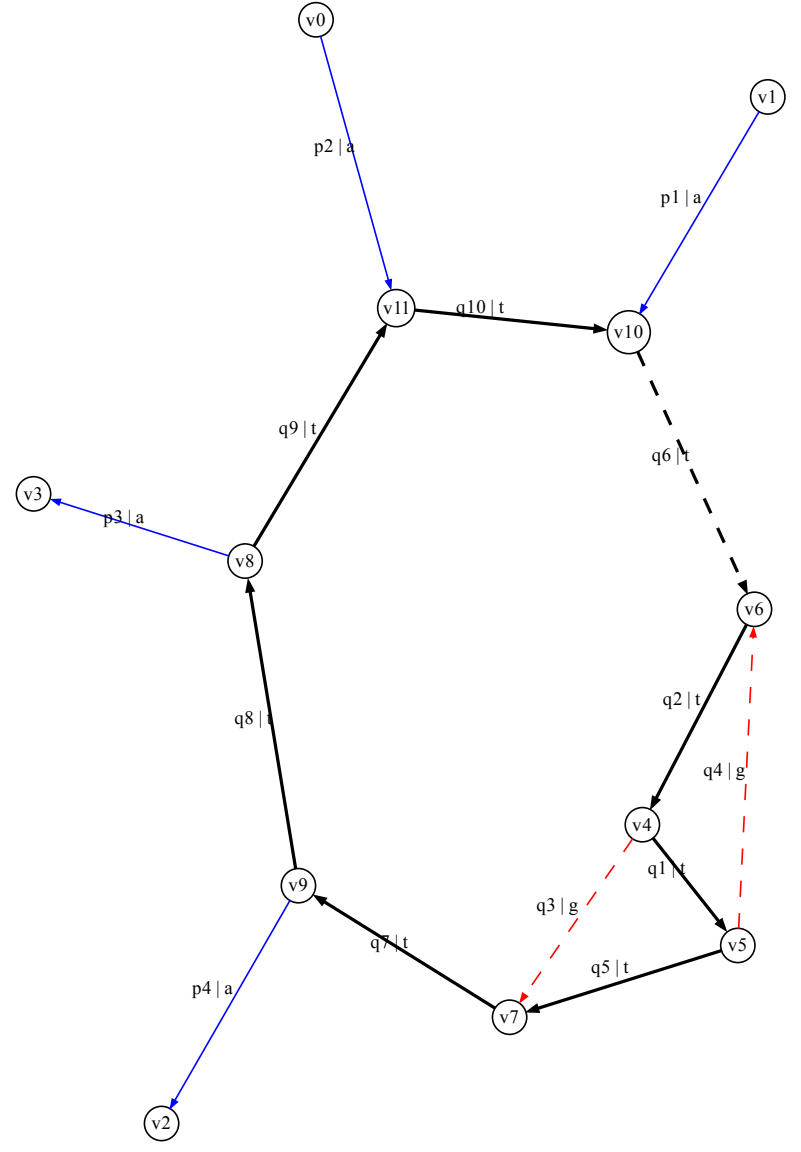

FSG GL114 #36 x (-4)

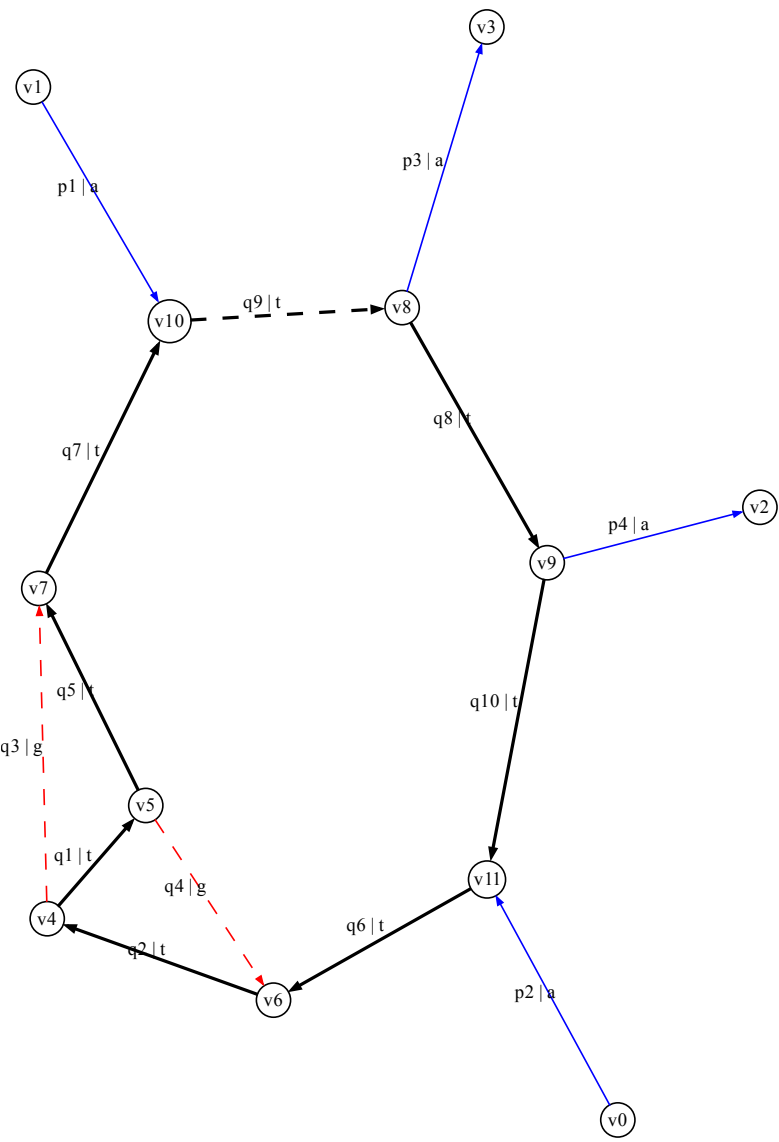

FSG GL116 #37 x (-4)

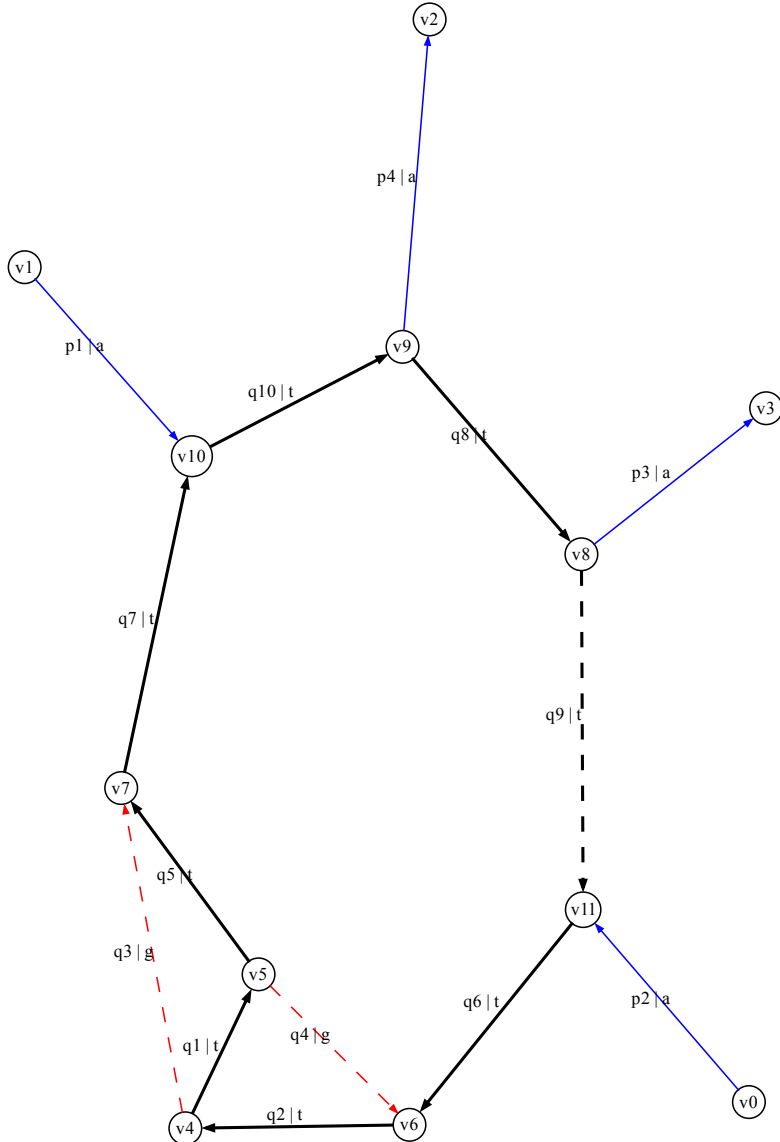

FSG GL118 #38 x (-4)

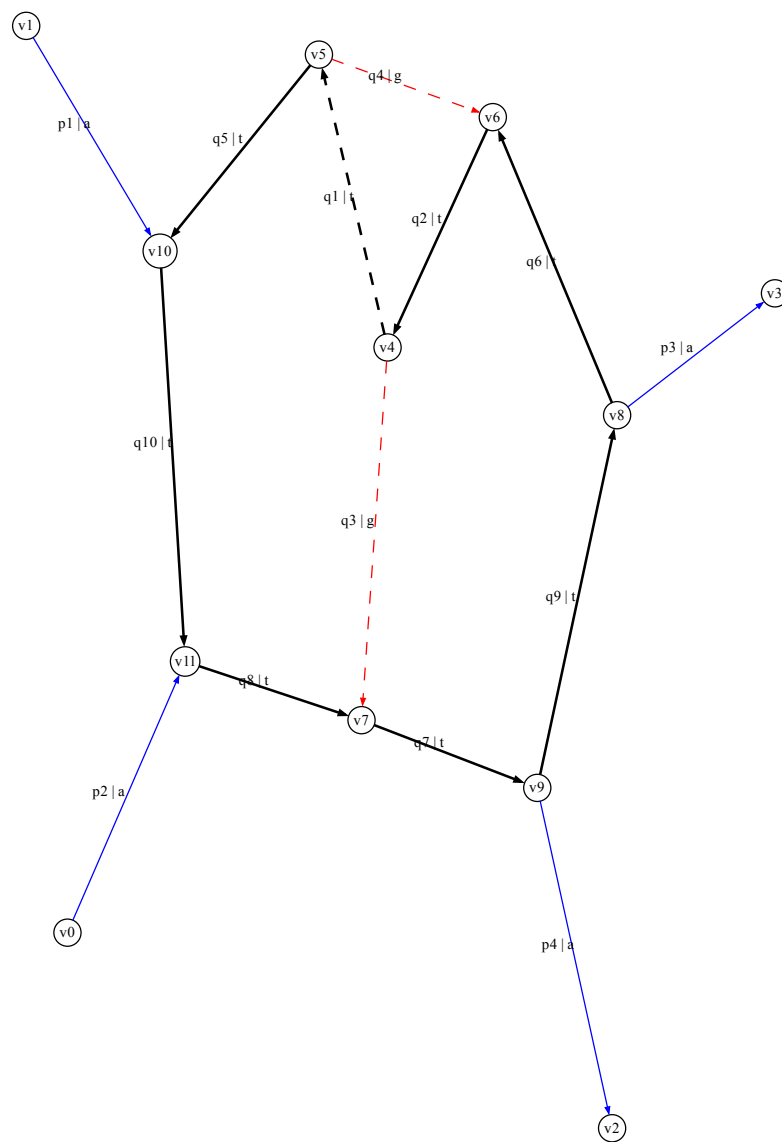

FSG GL120 #39 x (-4)

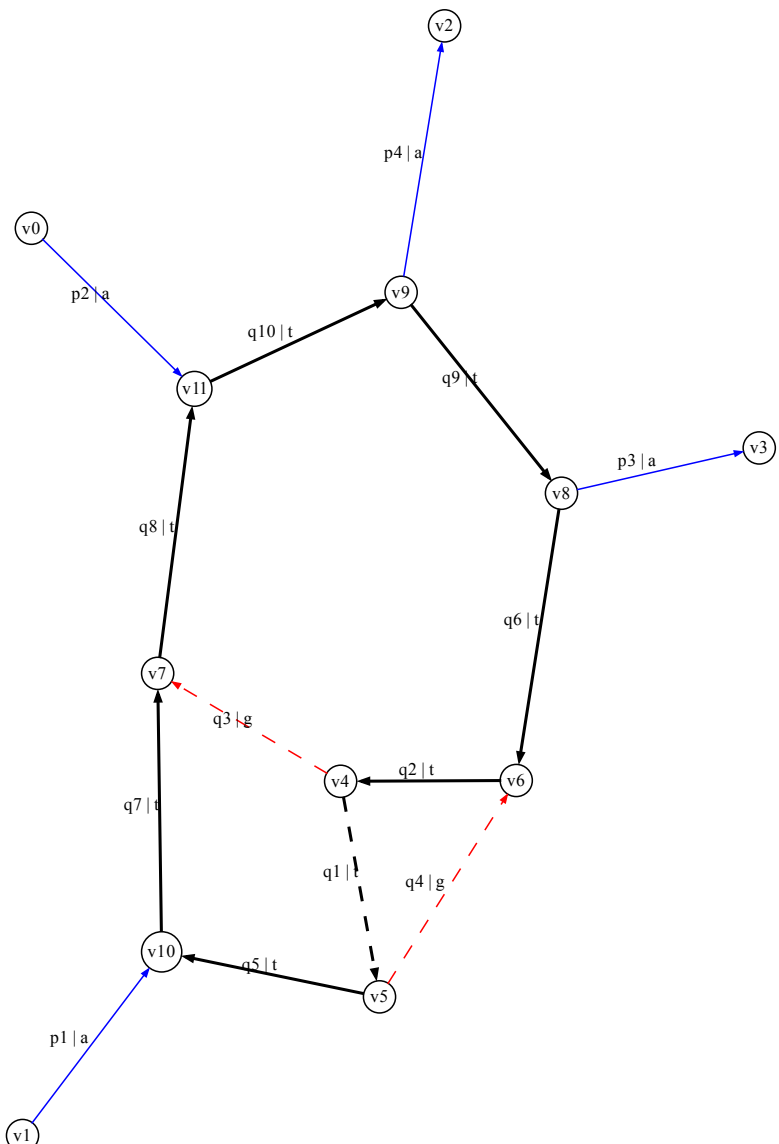

FSG GL122 #40 x (-8)

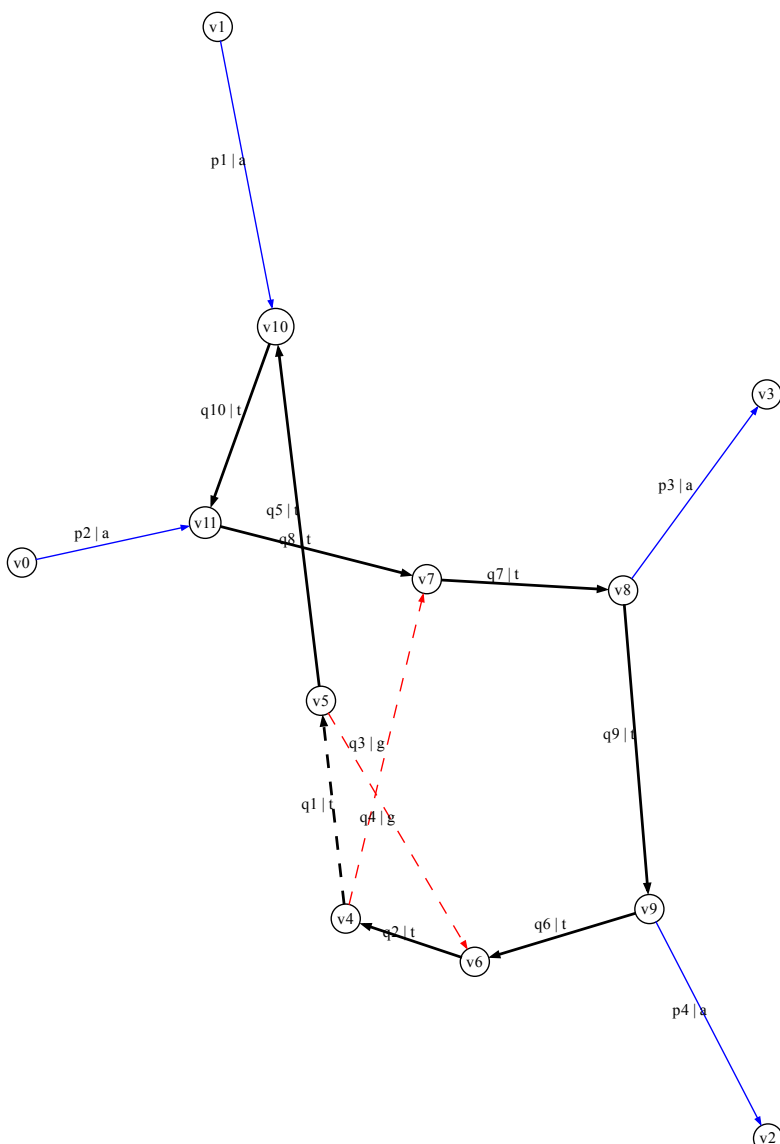

FSG GL124 #41 x (-4)

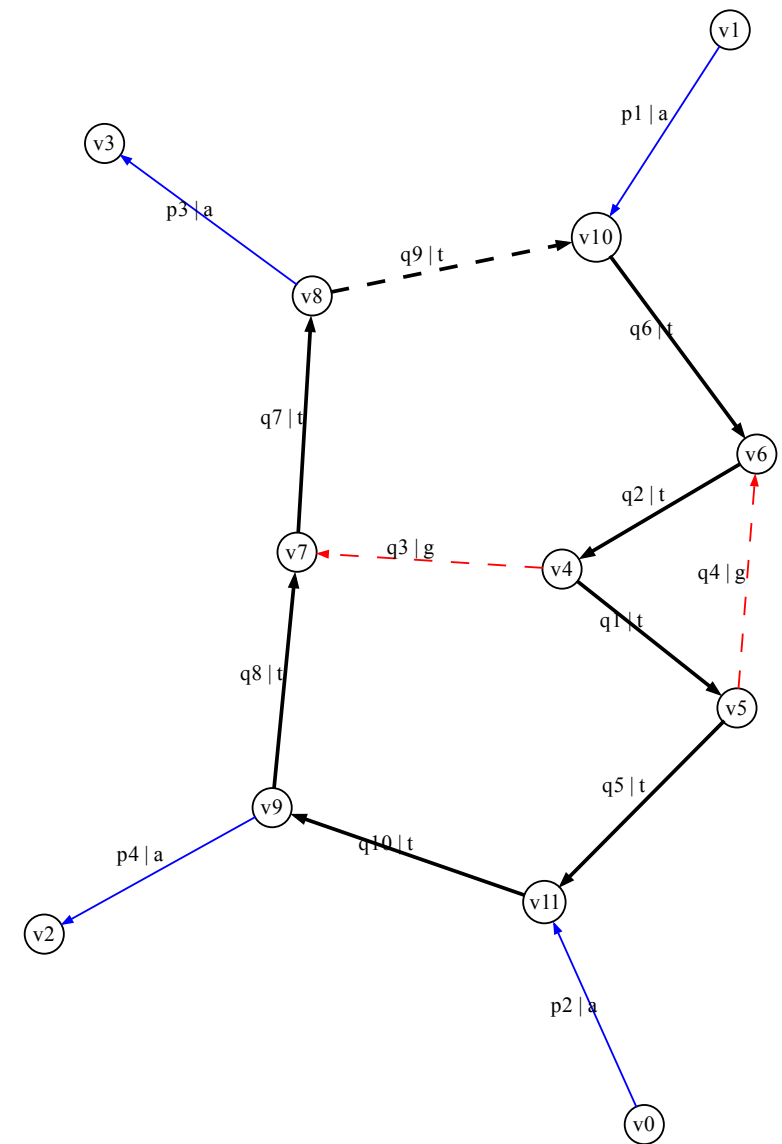

FSG GL130 #42 x (-4)

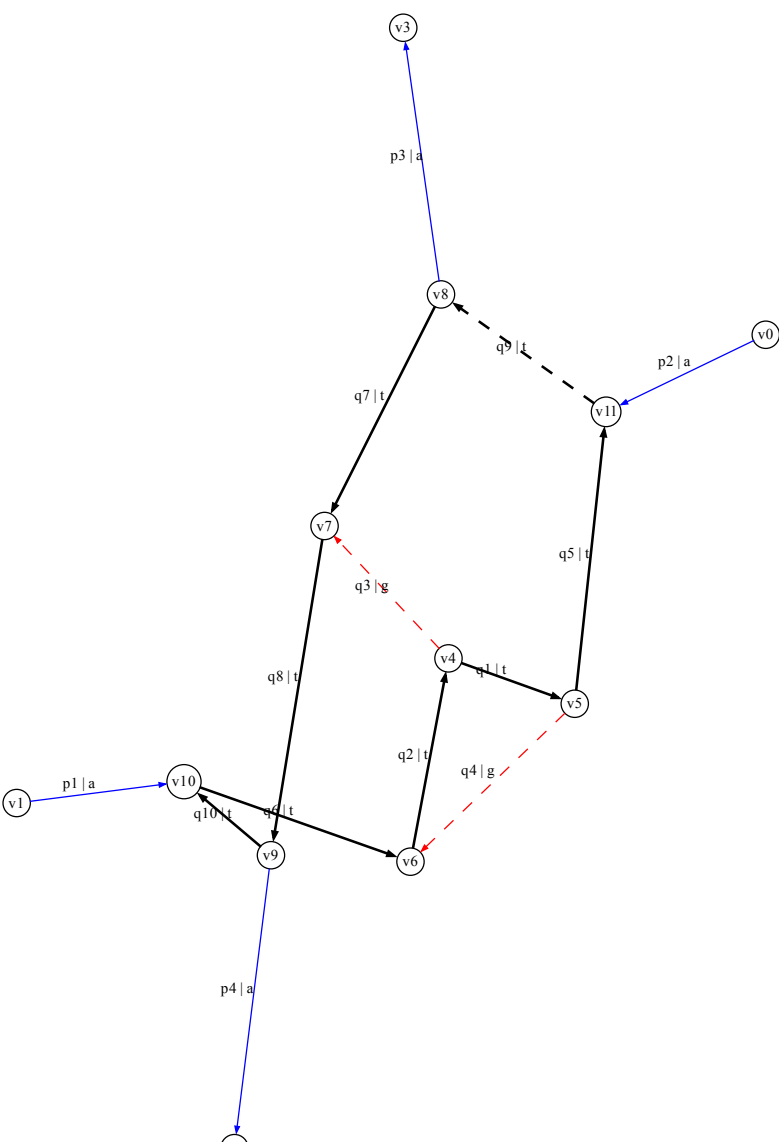

FSG GL132 #43 x (-4)

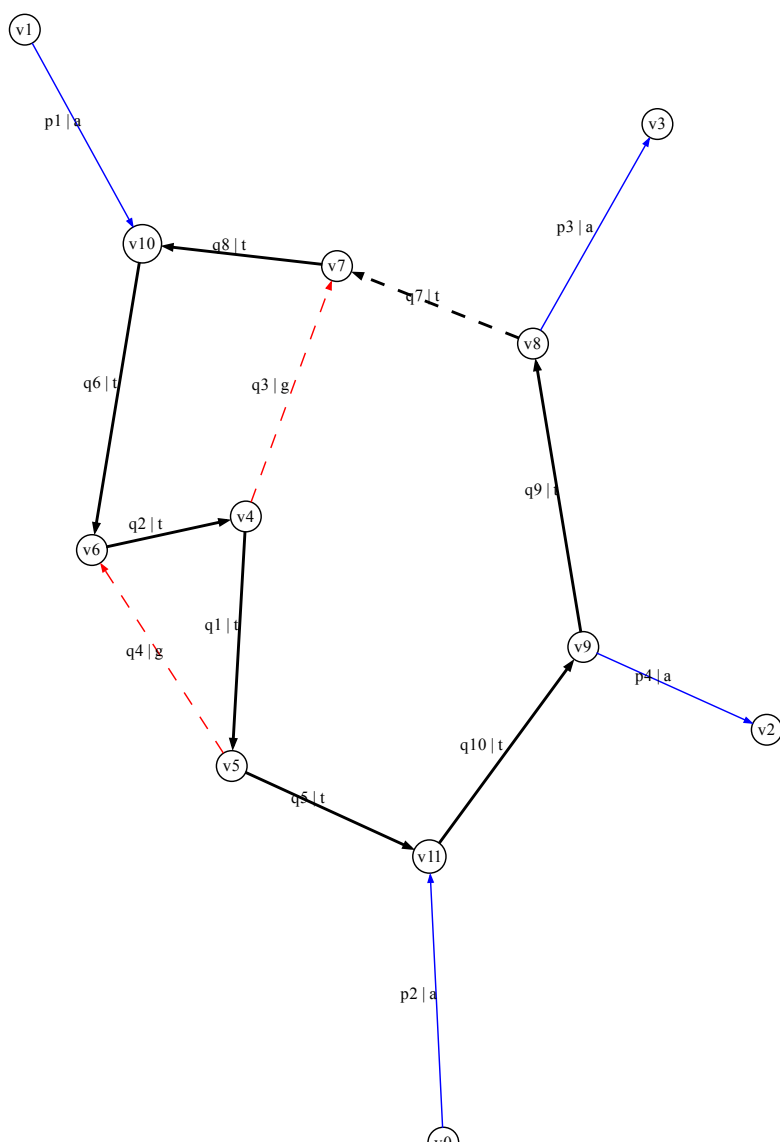

FSG GL134 #44 x (-8)

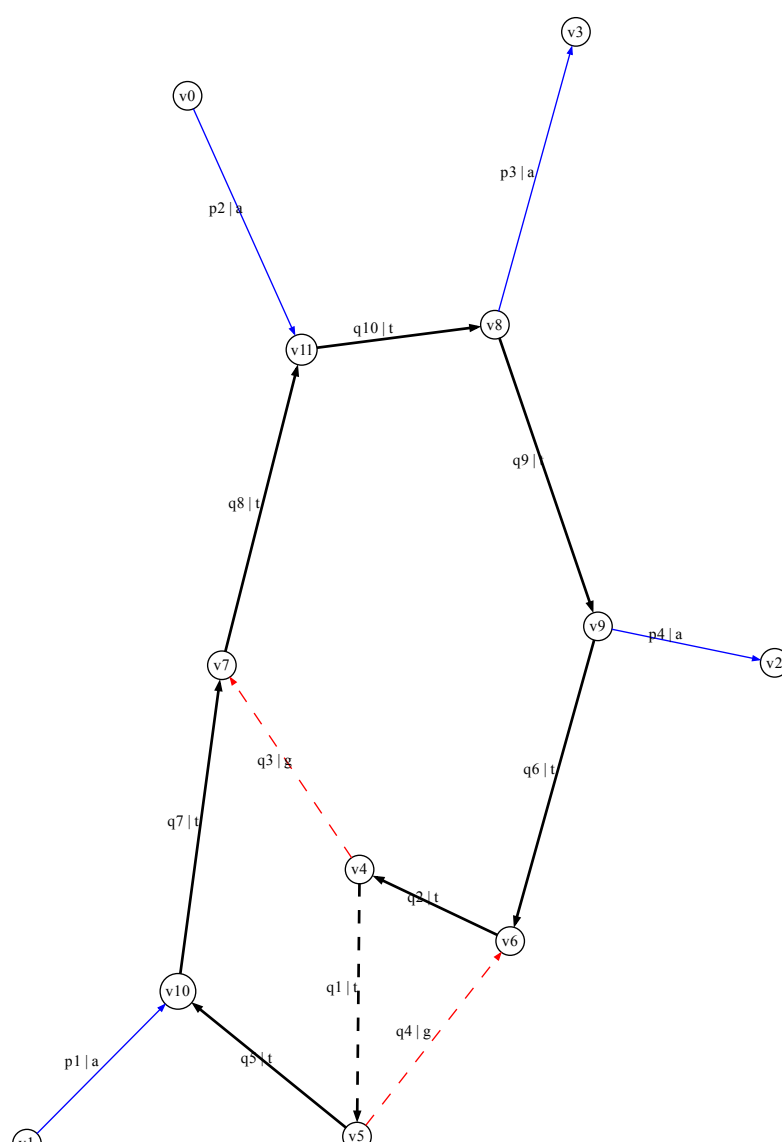

FSG GL136 #45 x (-8)

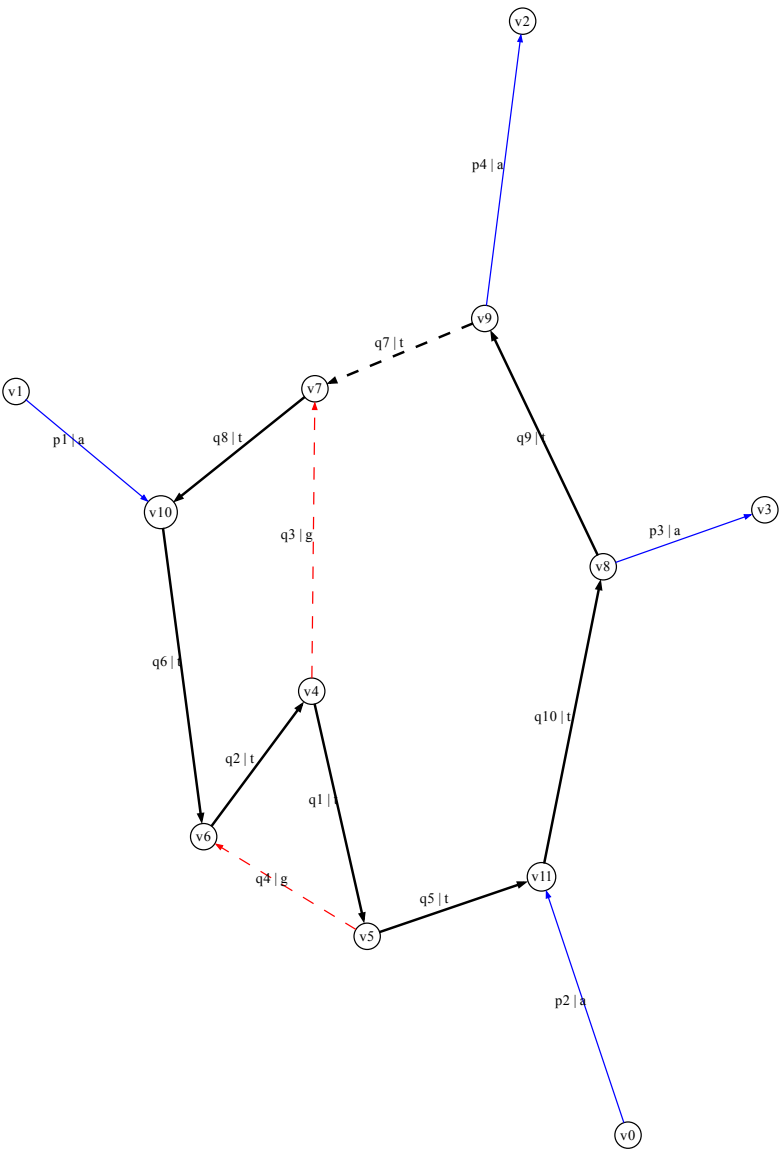

FSG GL138 #46 x (-8)

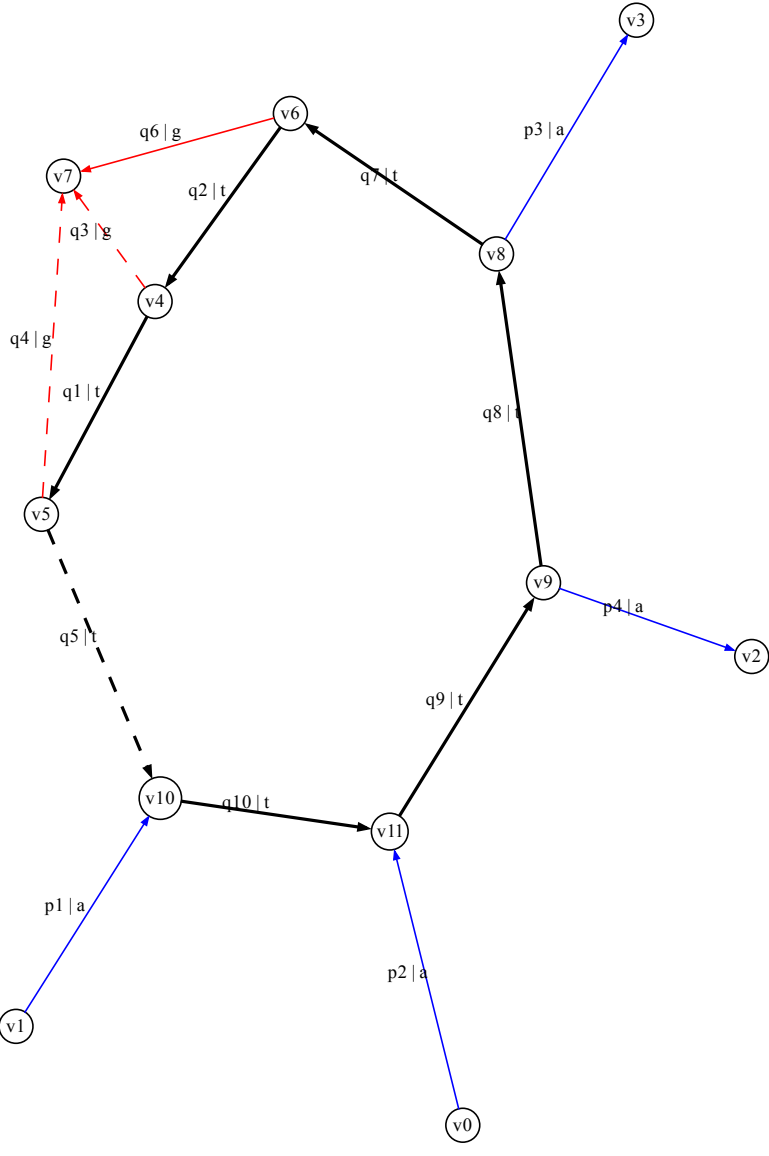

FSG GL144 #47 x (-4)

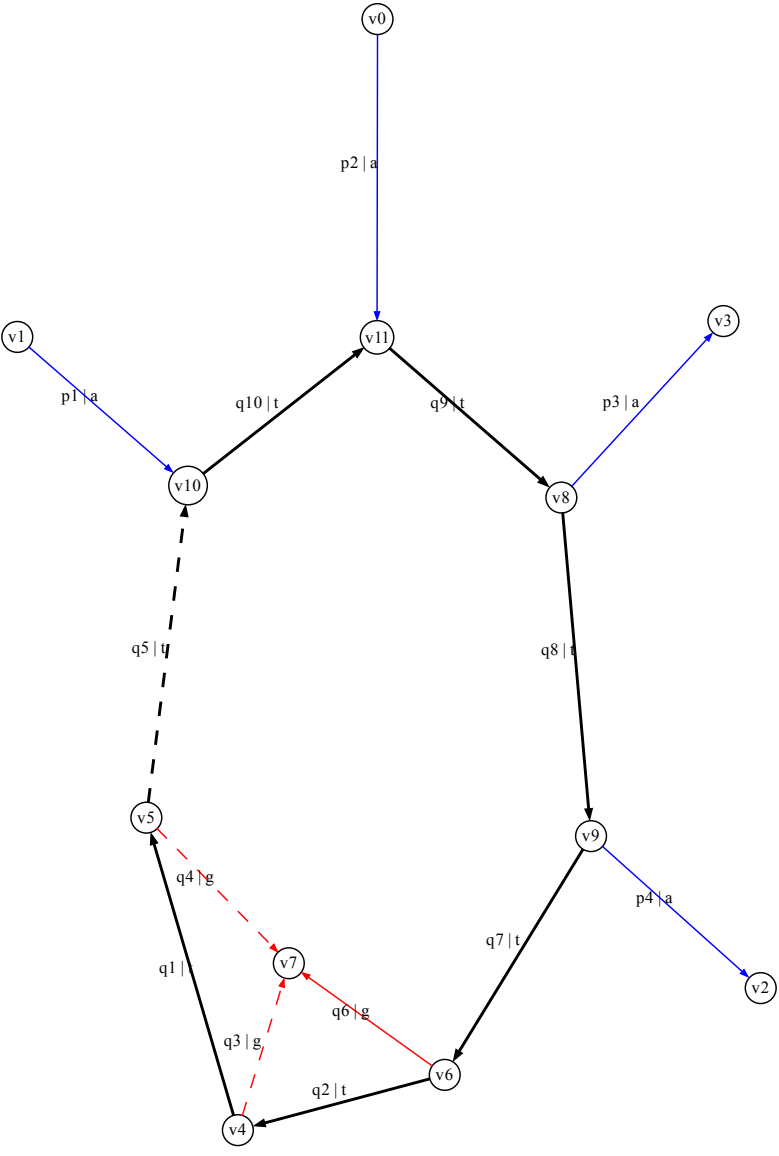

FSG GL146 #48 x (-4)

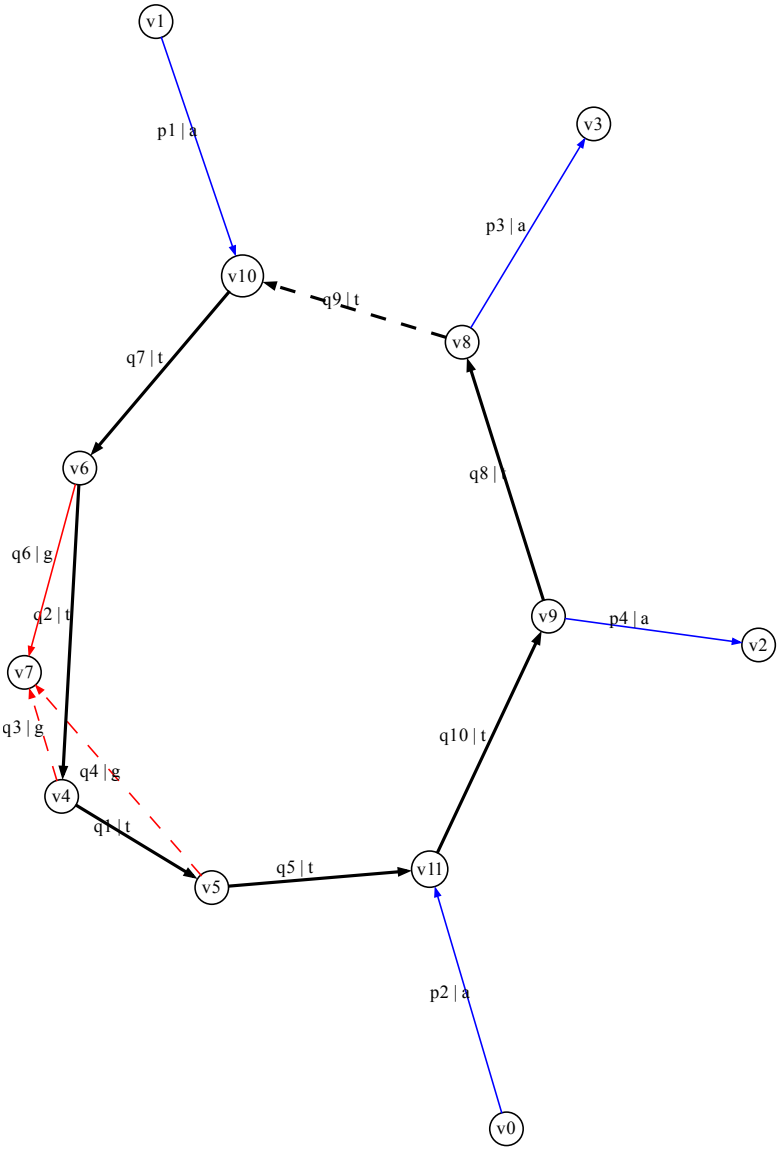

FSG GL148 #49 x (-4)

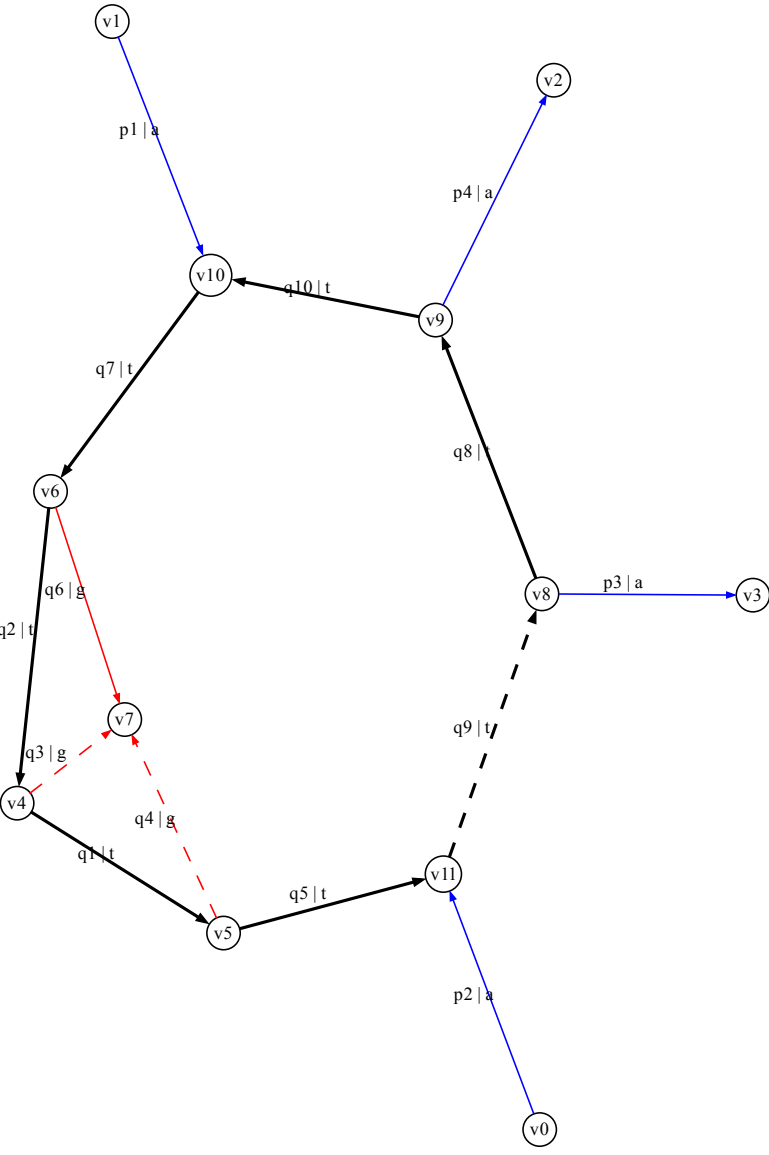

FSG GL150 #50 x (-4)

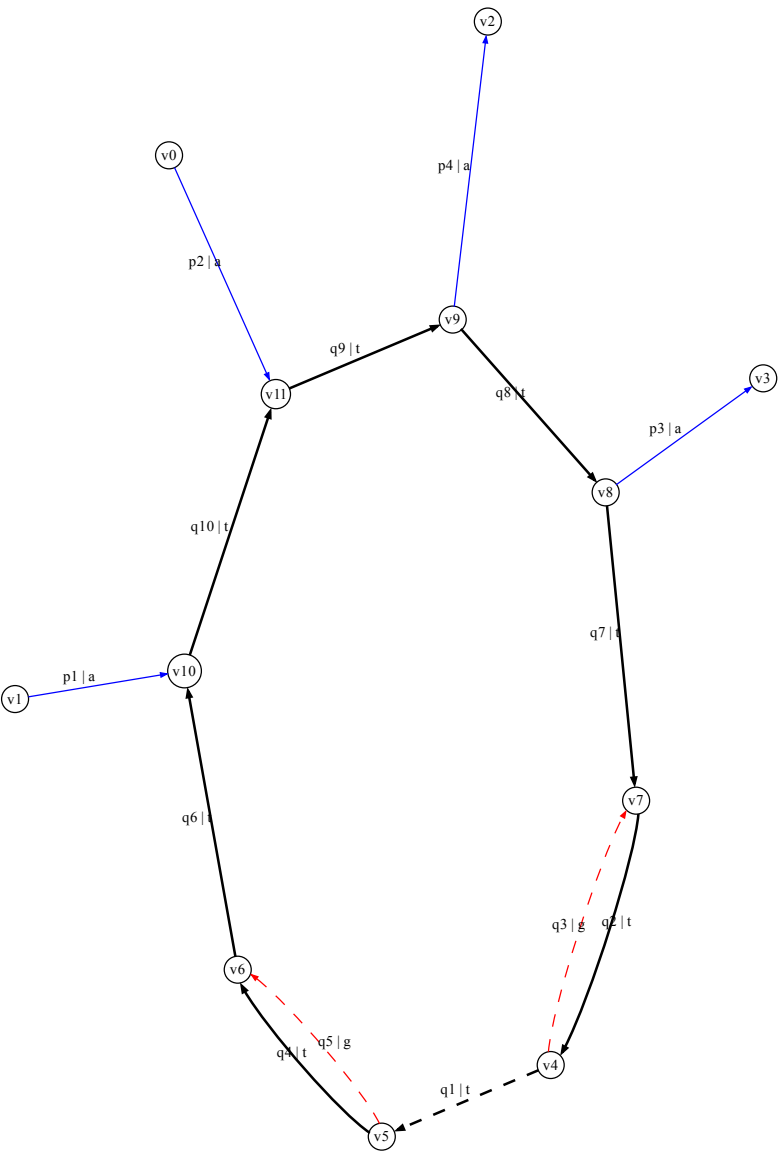

FSG GL152 #51 x (-4)

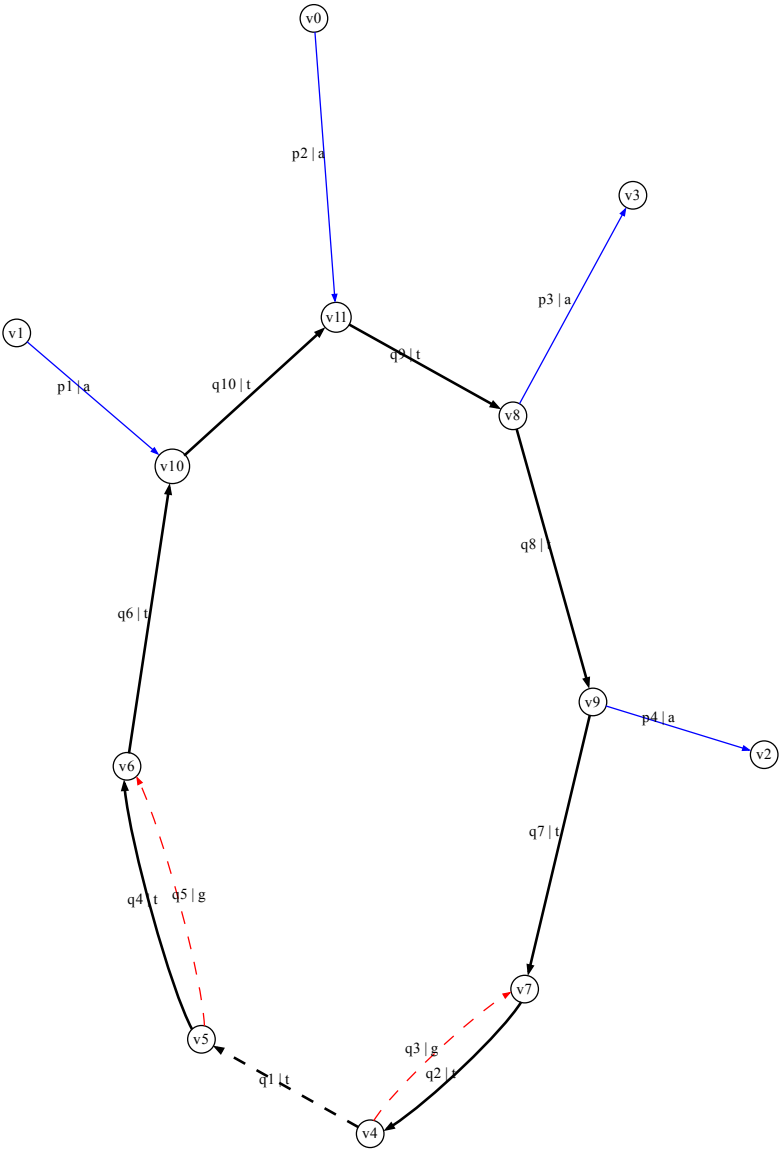

FSG GL154 #52 x (-4)

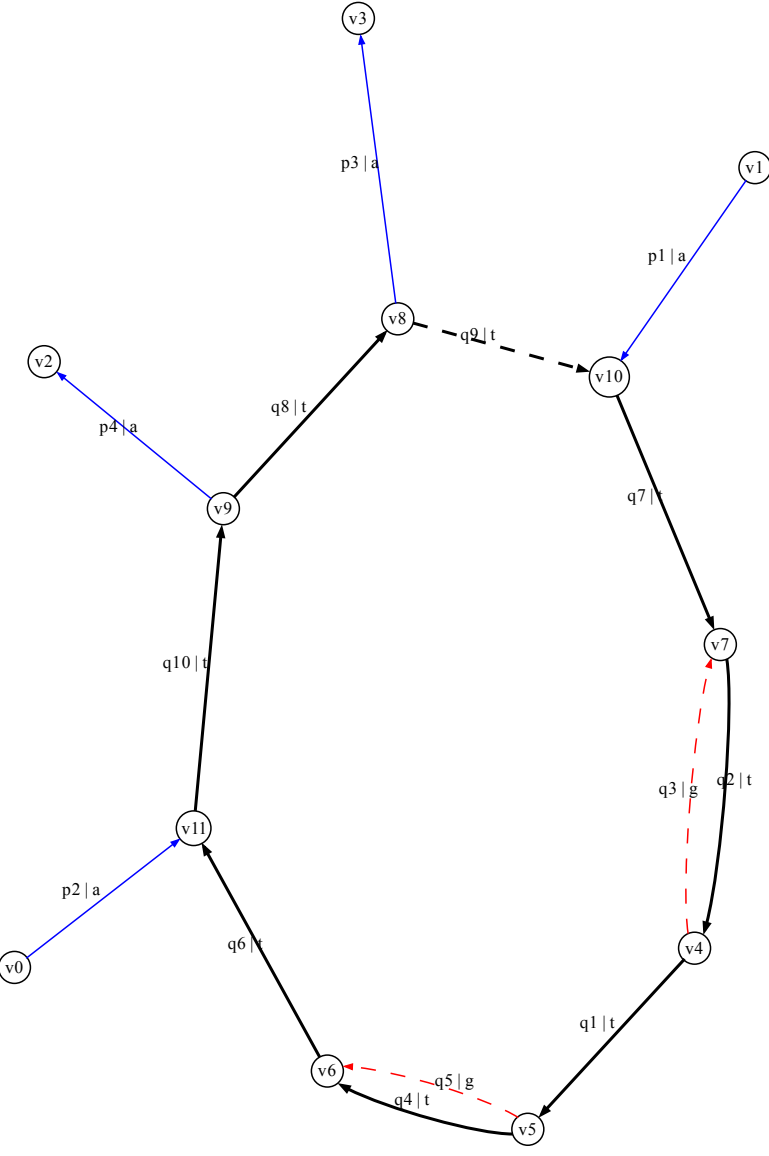

FSG GL156 #53 x (-4)

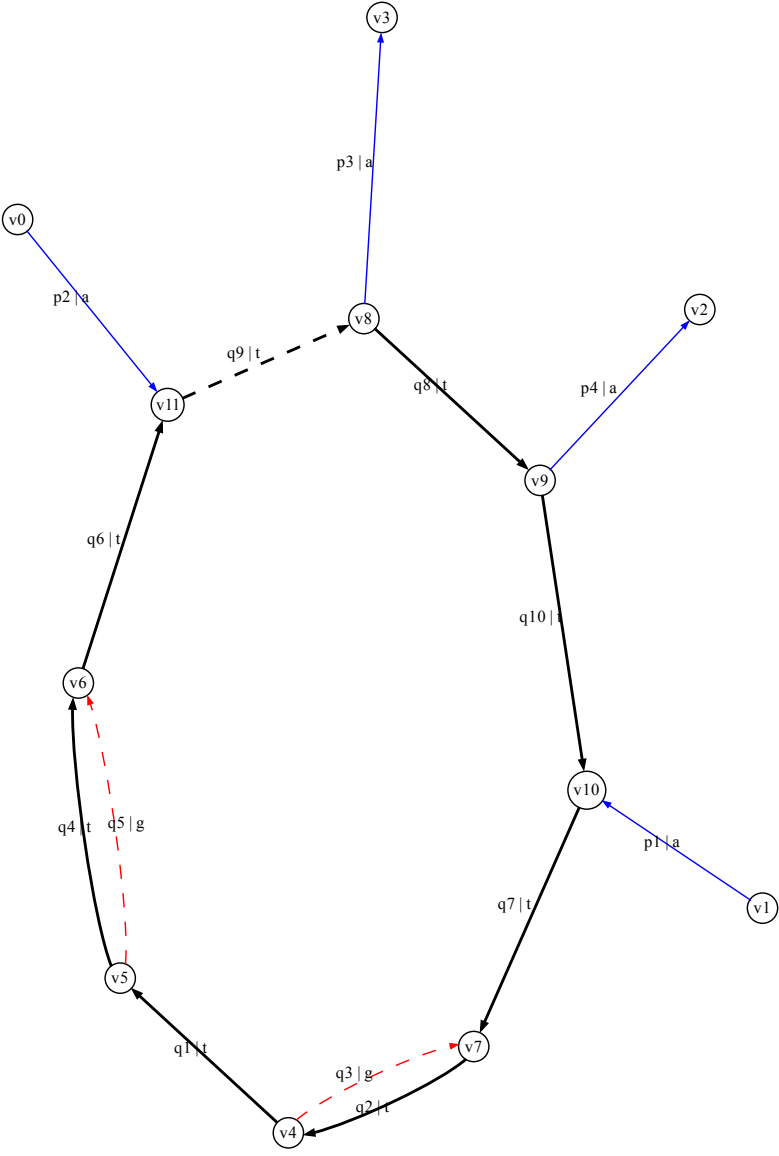

FSG GL158 #54 x (-4)

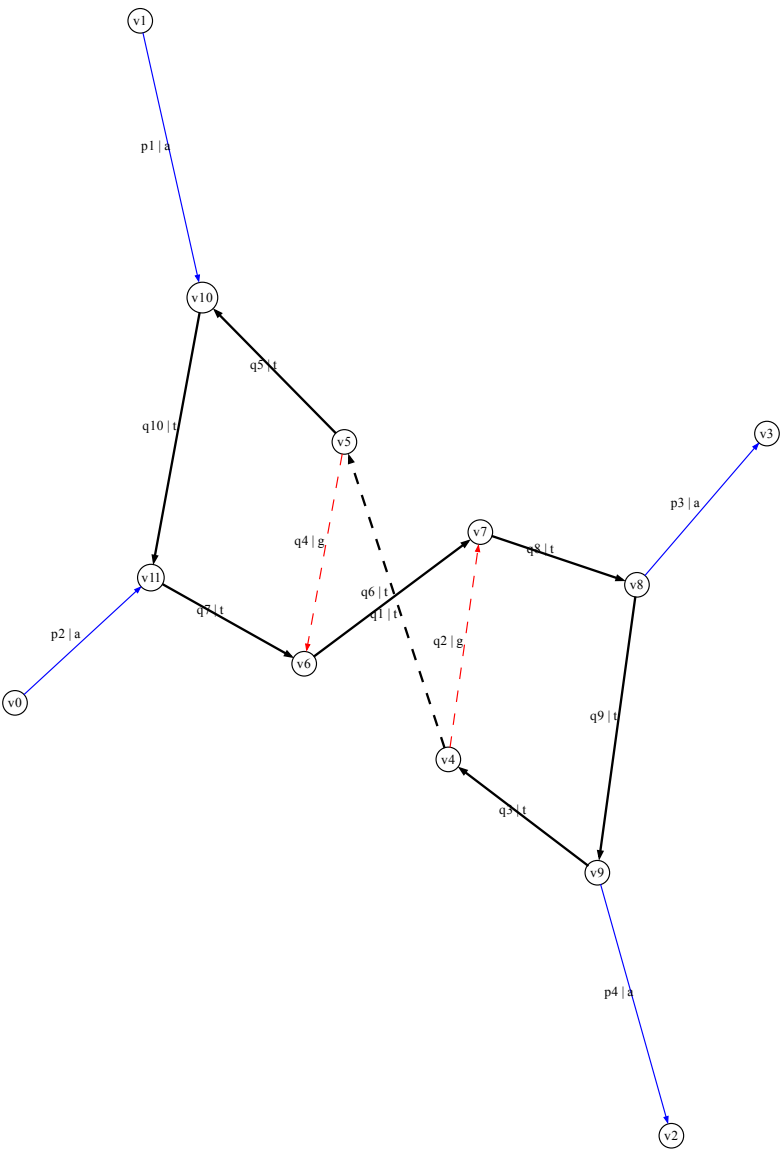

FSG GL160 #55 x (-2)

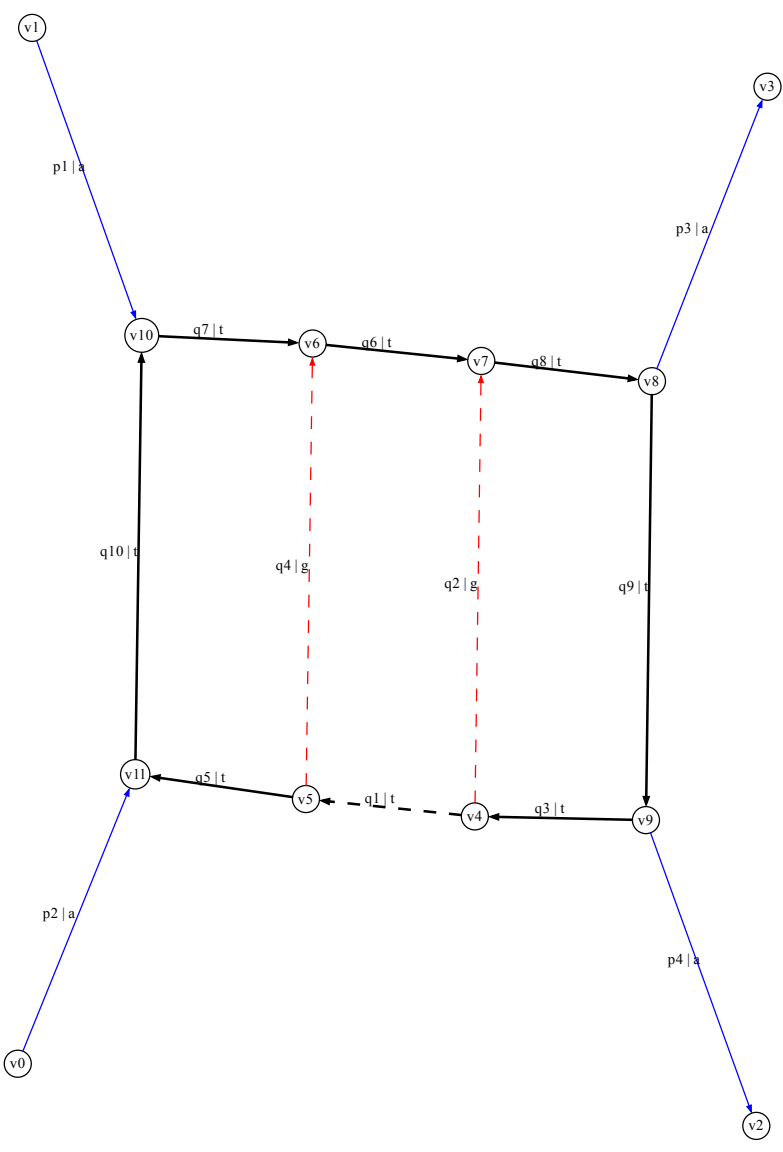

FSG GL162 #56 x (-2)

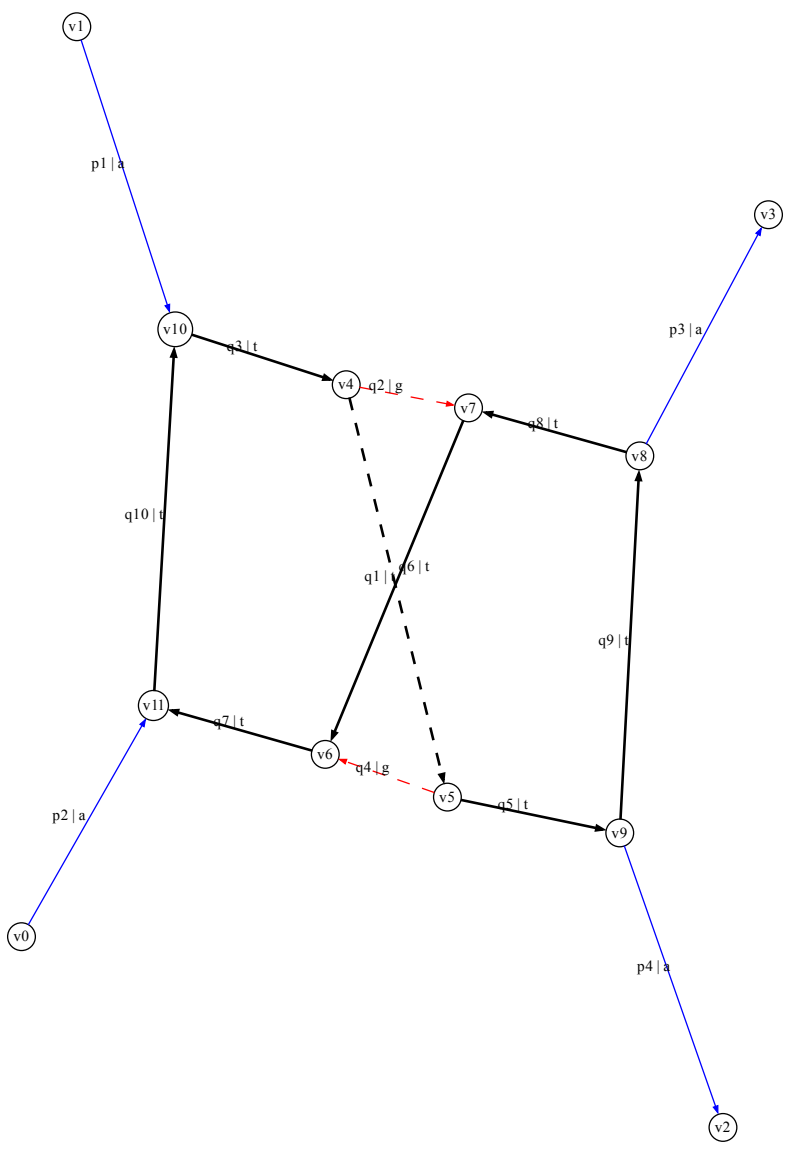

FSG GL164 #57 x (-2)

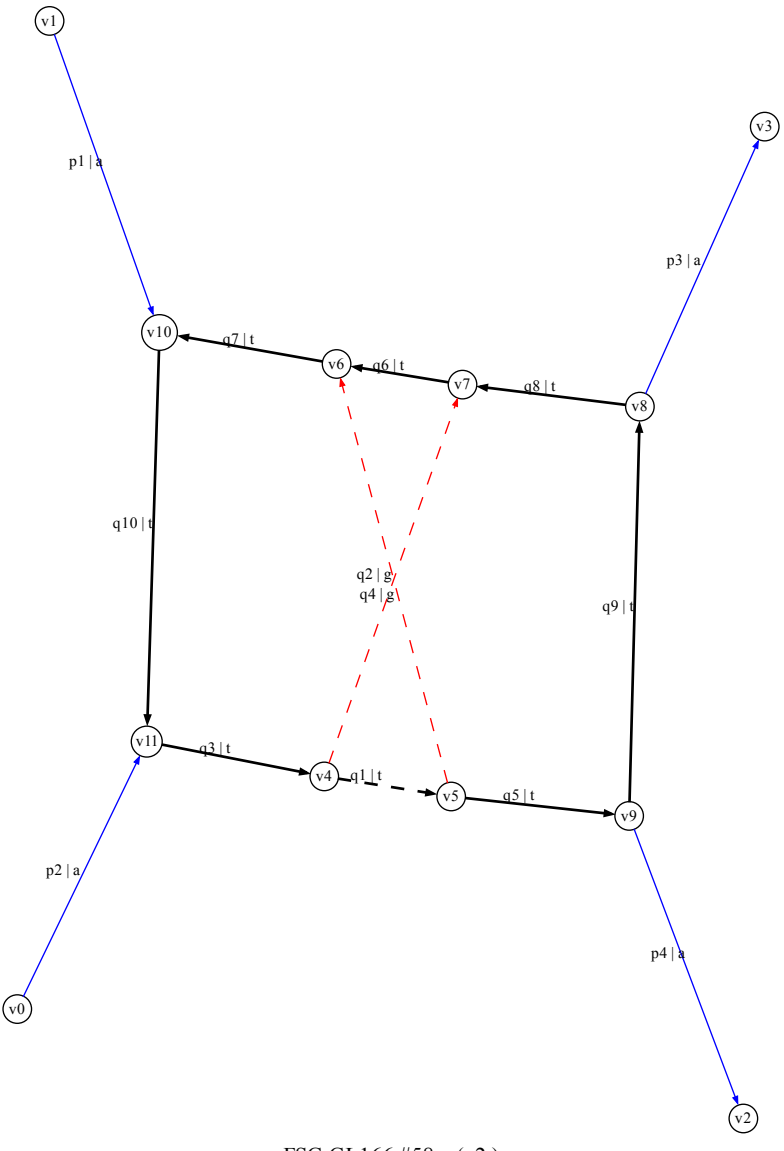

FSG GL166 #58 x (-2)

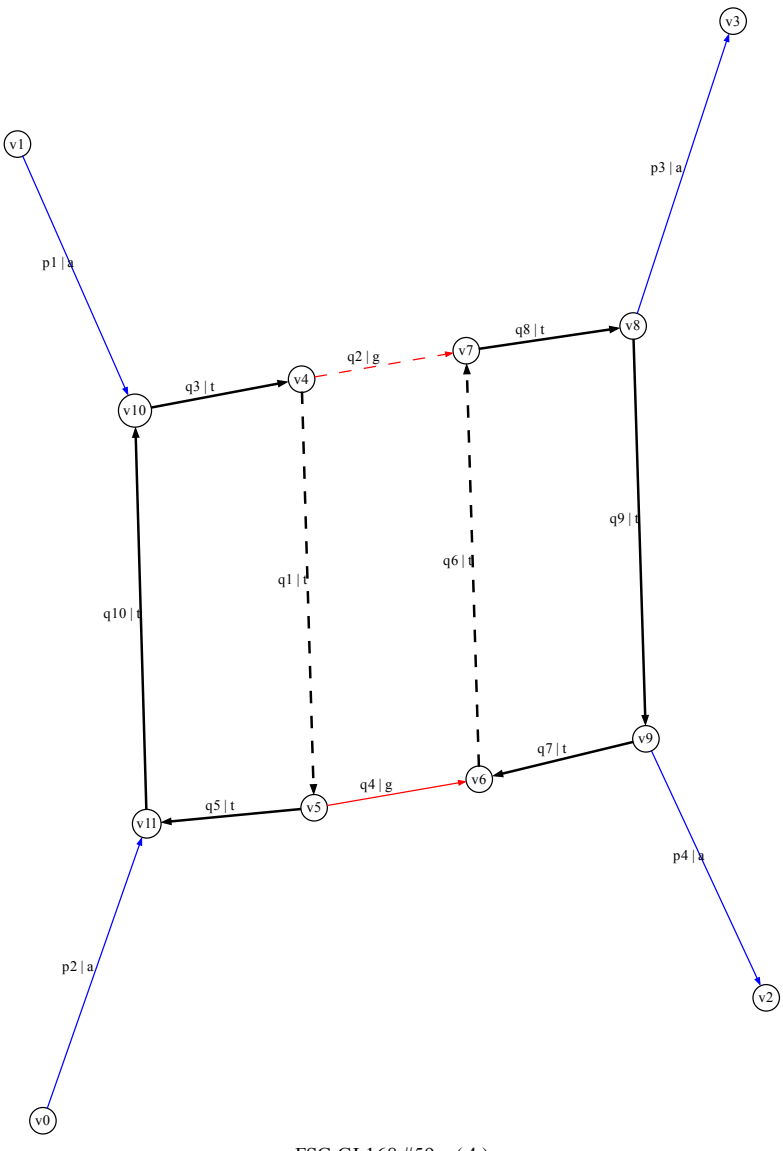

FSG GL168 #59 x (4)

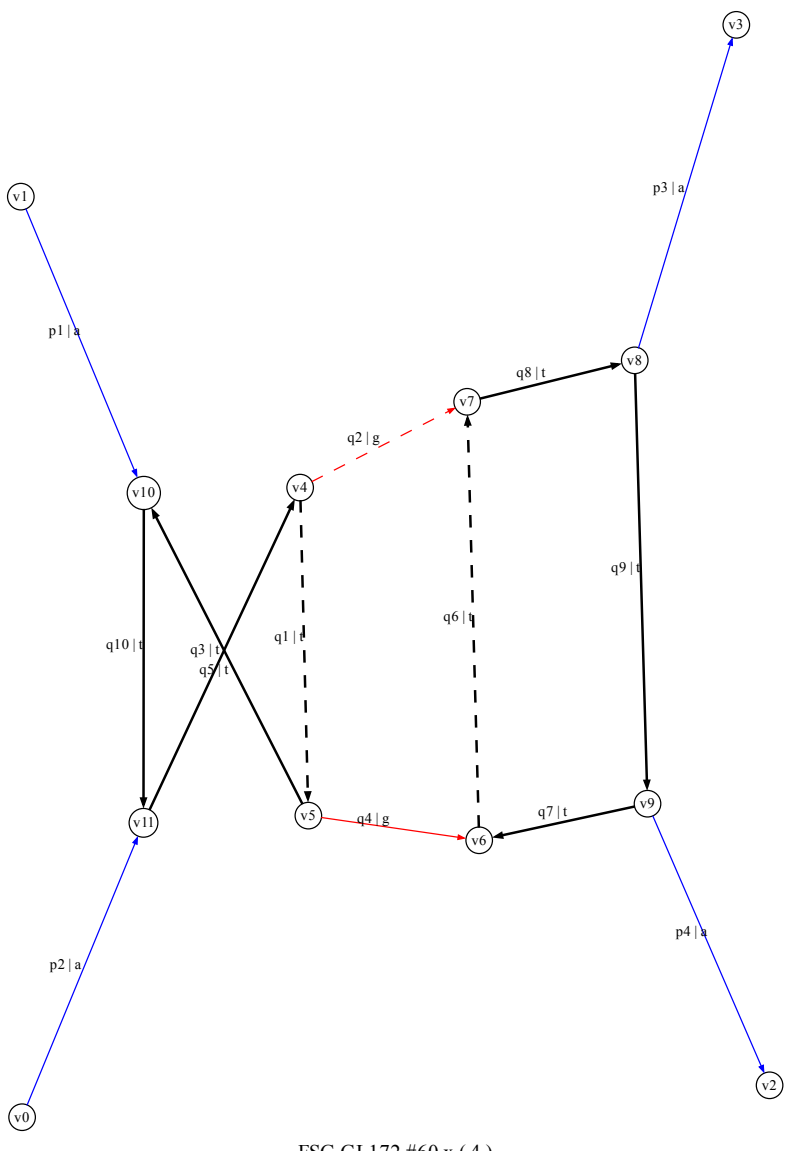

FSG GL172 #60 x (4)

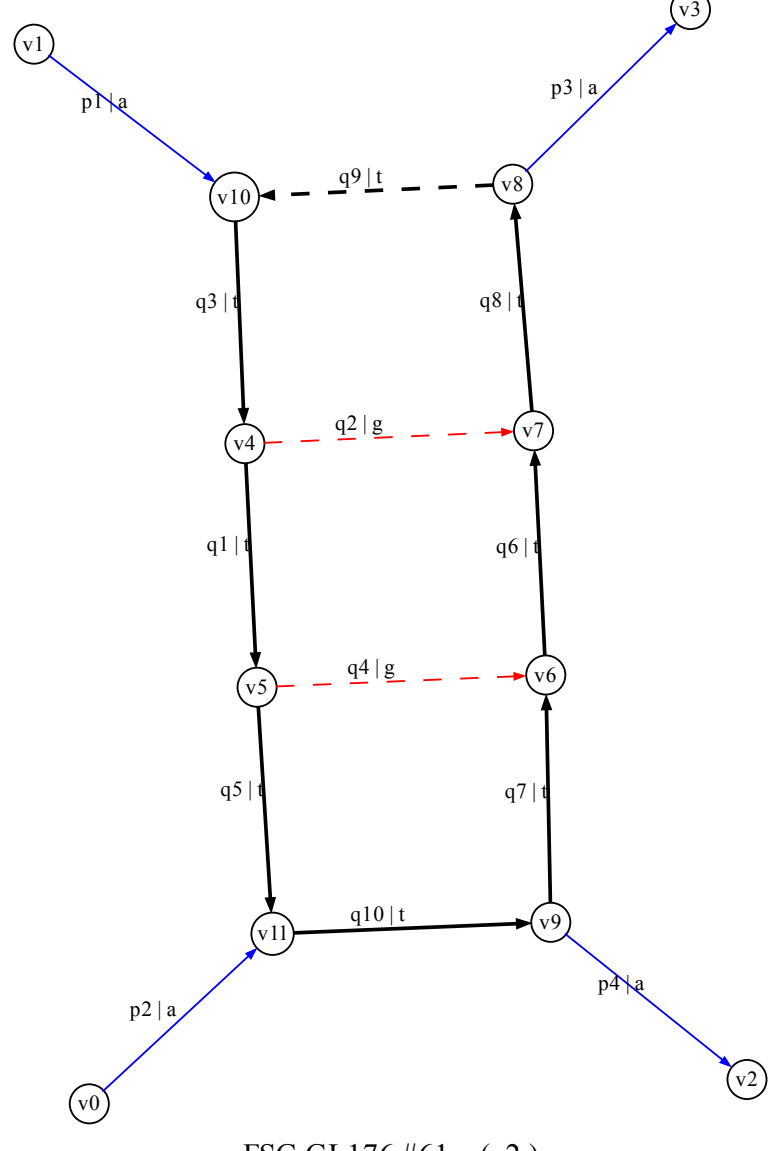

FSG GL176 #61 x (-2)

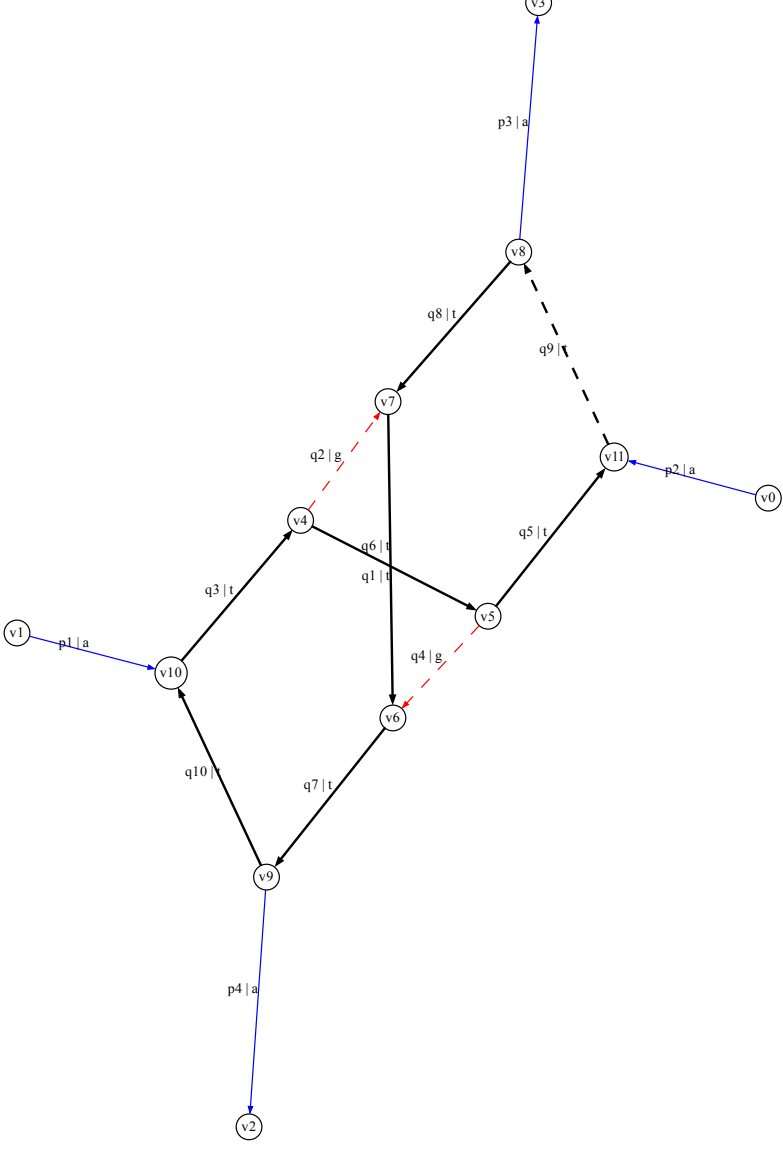

FSG GL178 #62 x (-2)

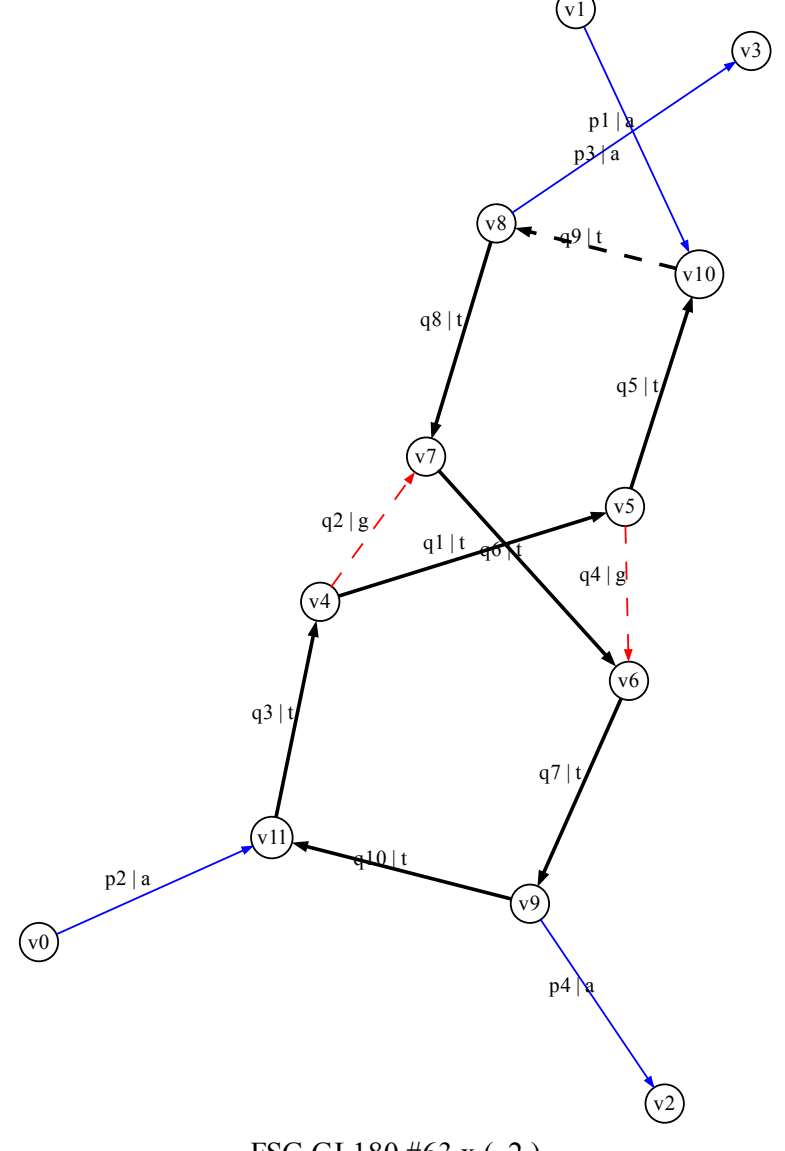

FSG GL180 #63 x (-2)

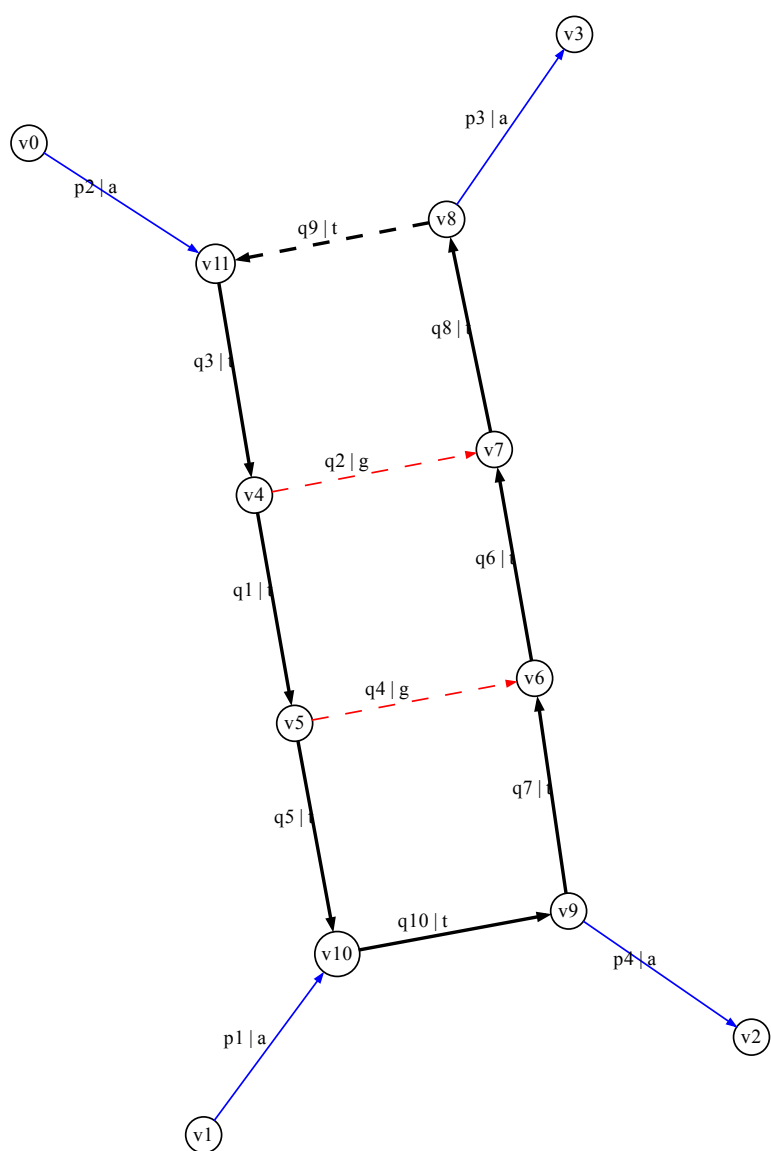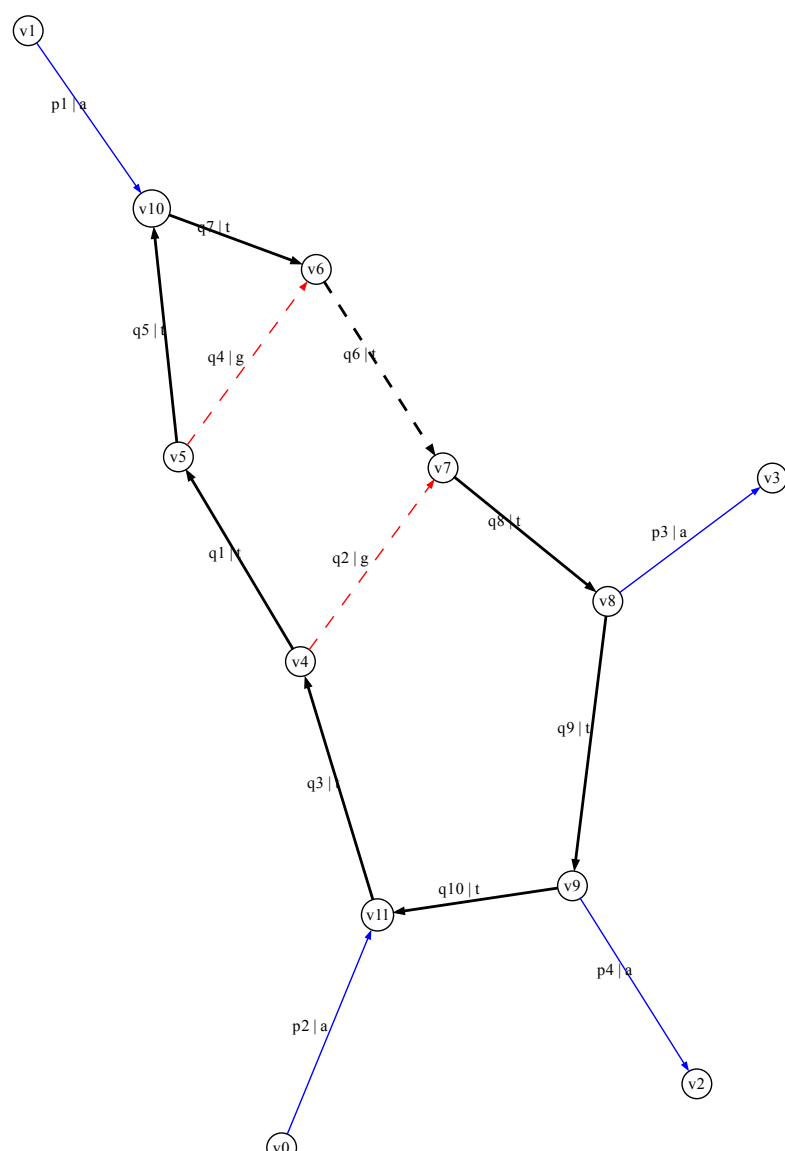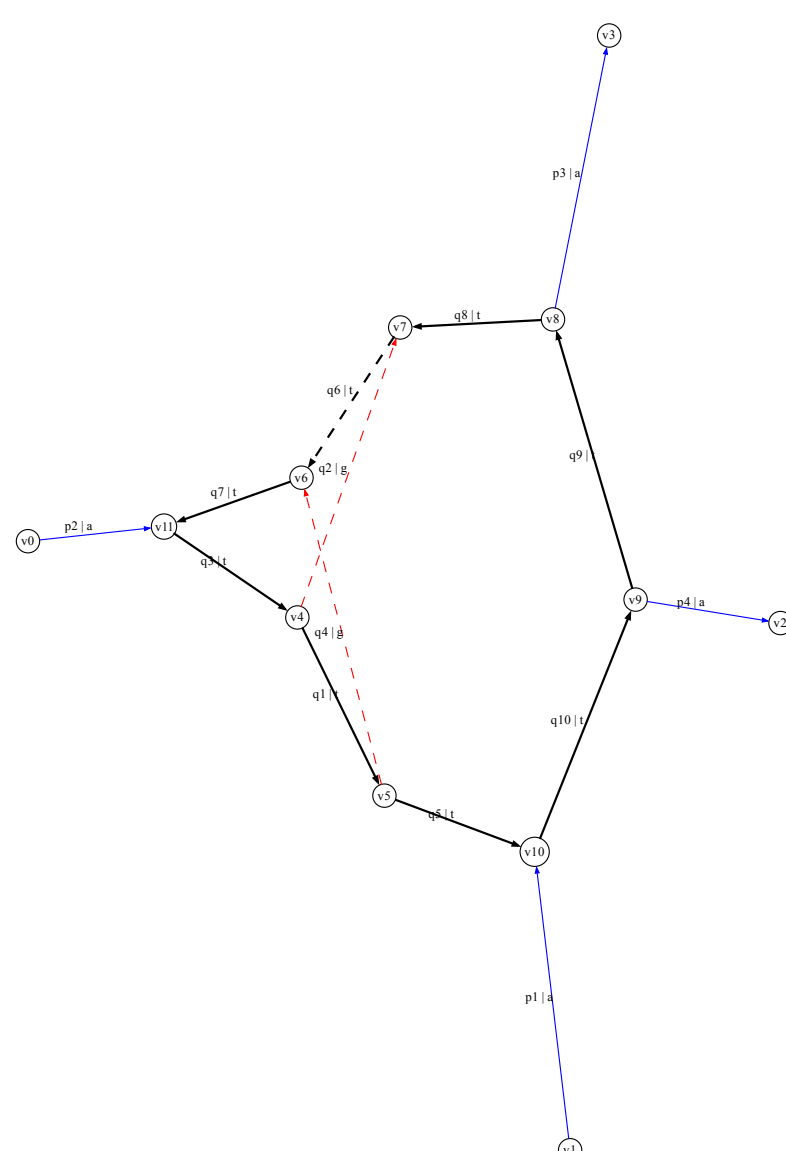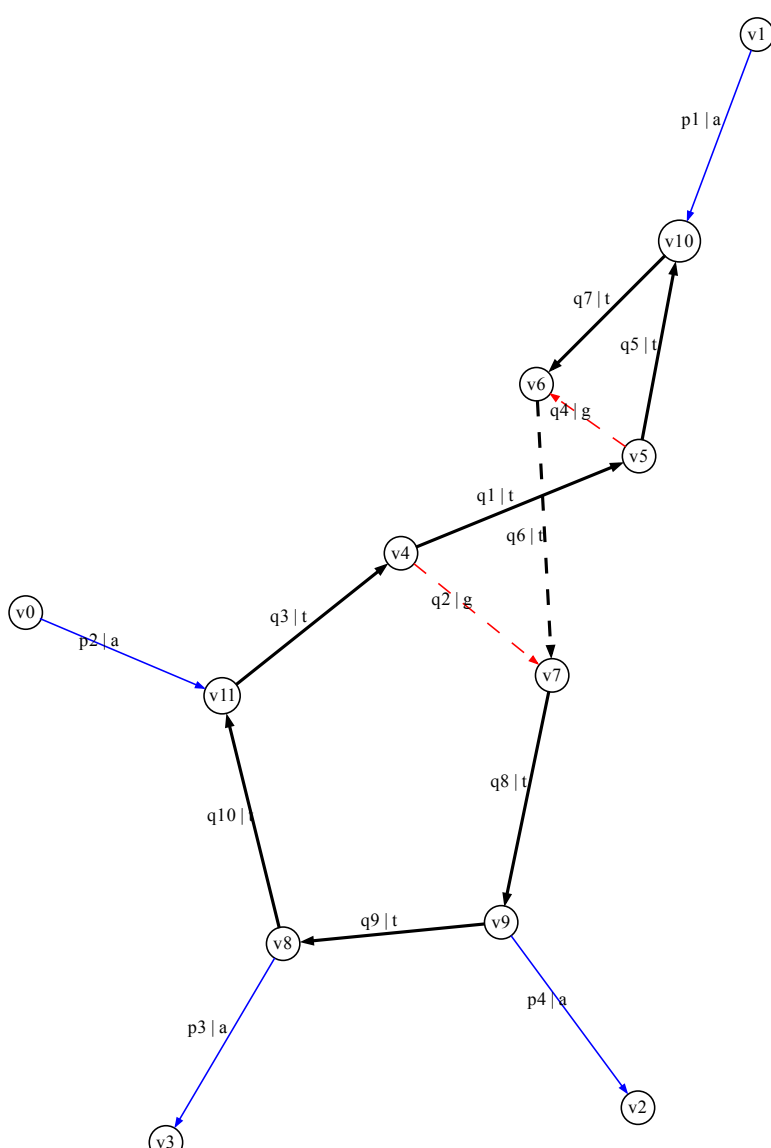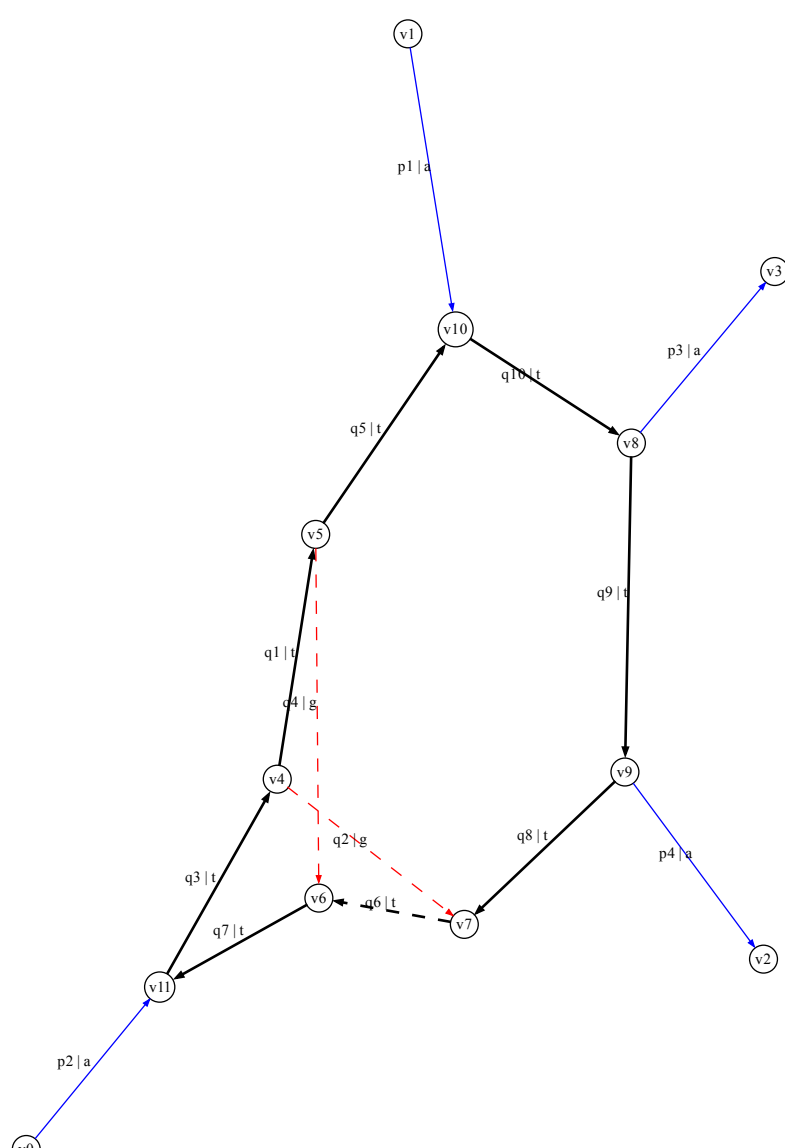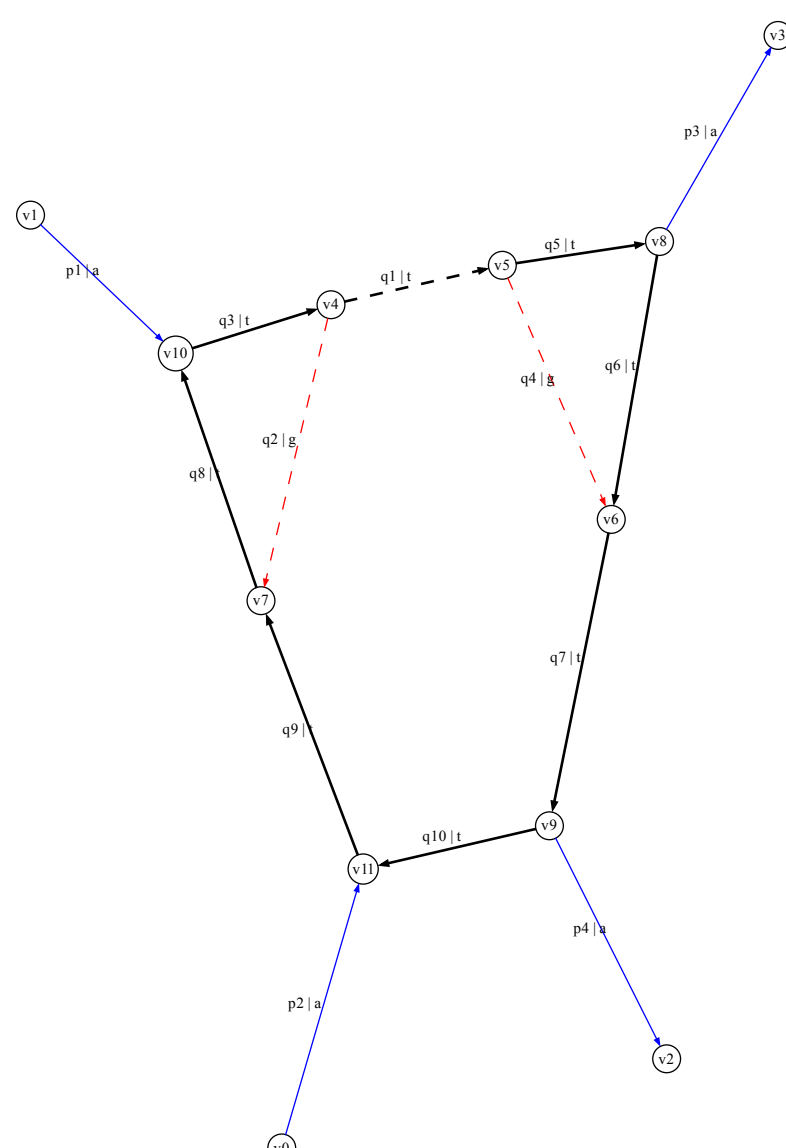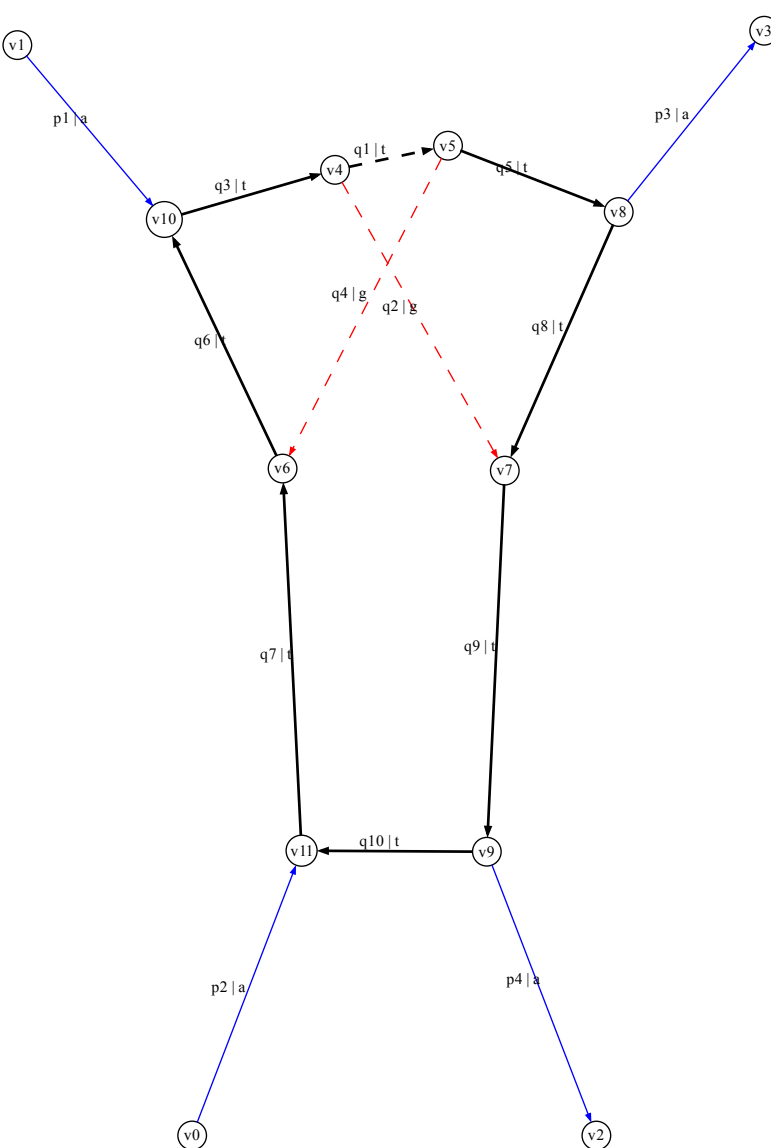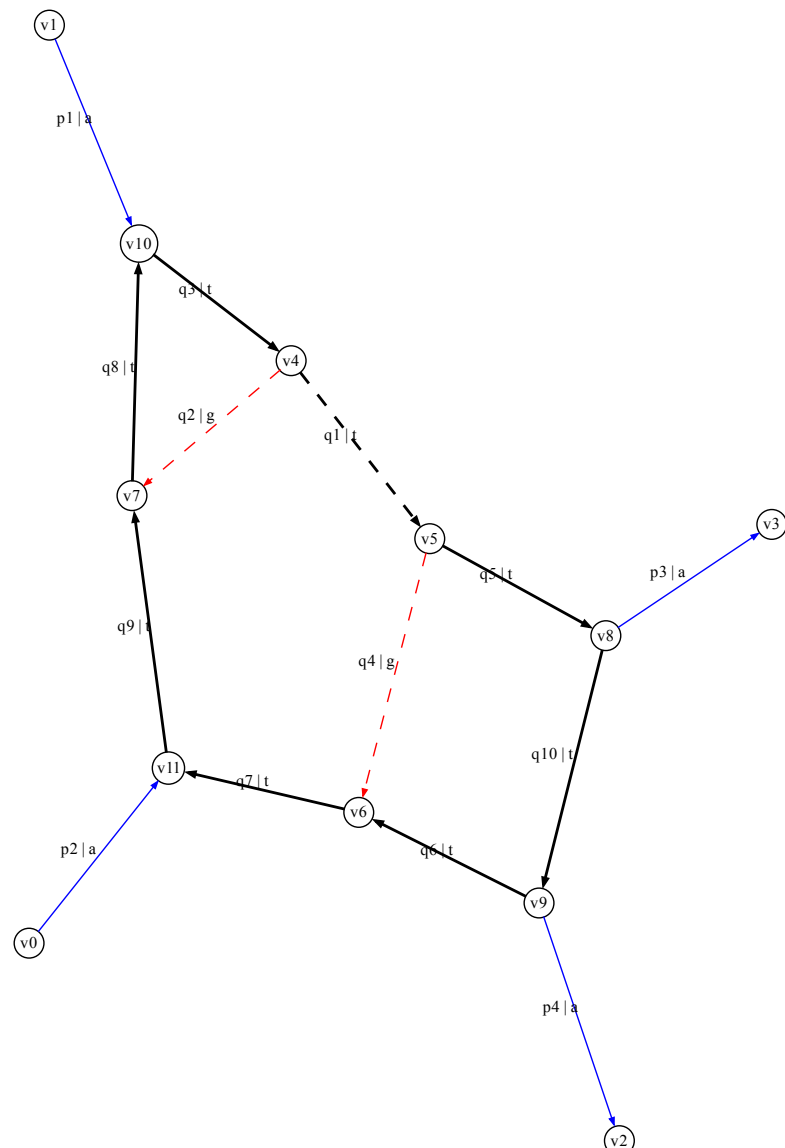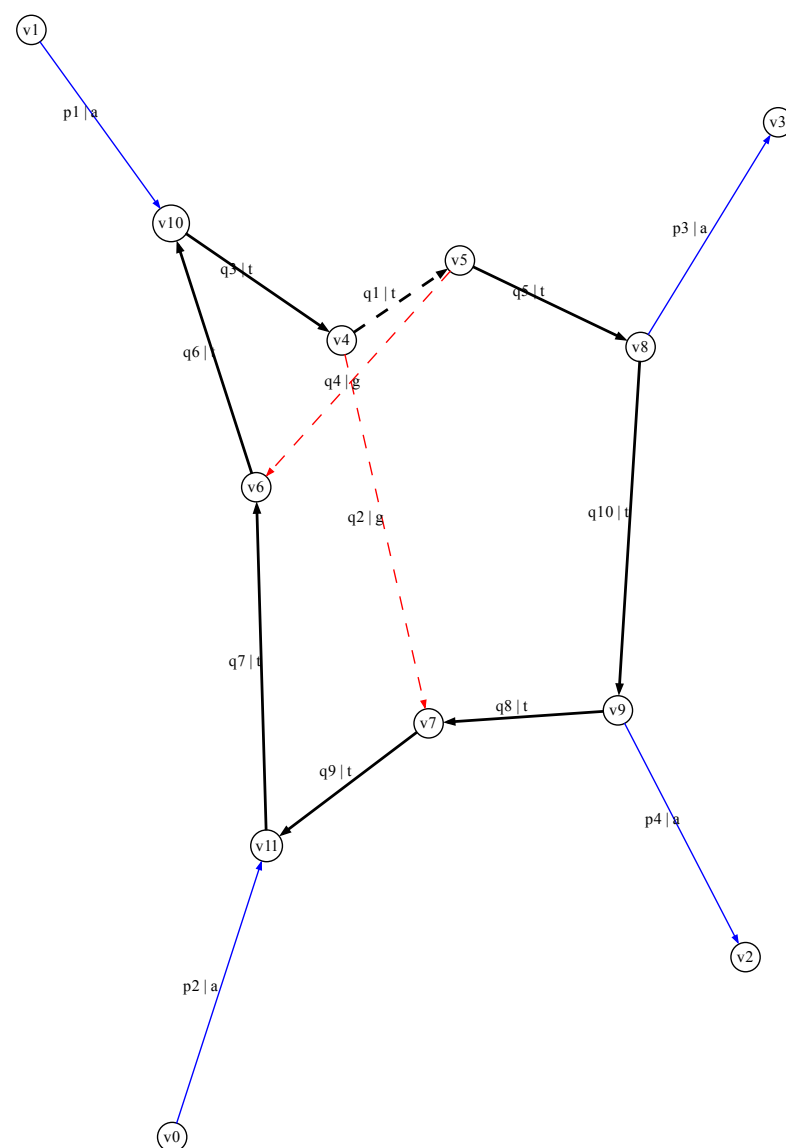

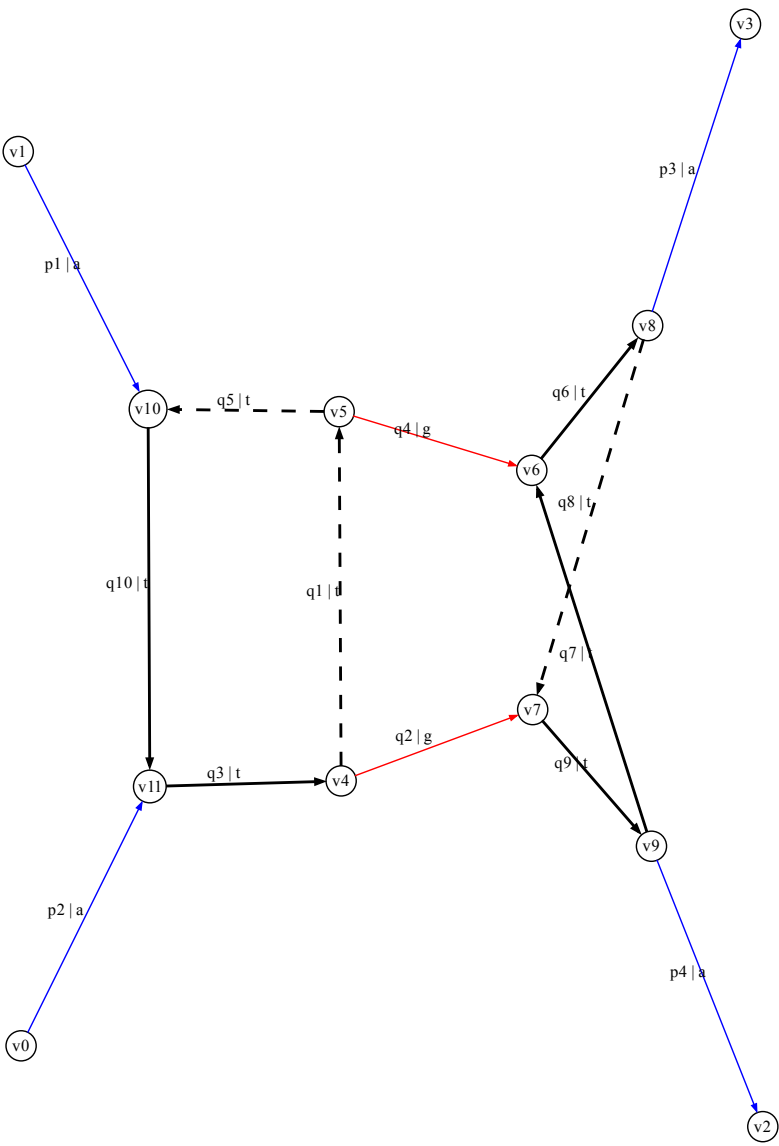

FSG GL208 #73 x ( 8 )

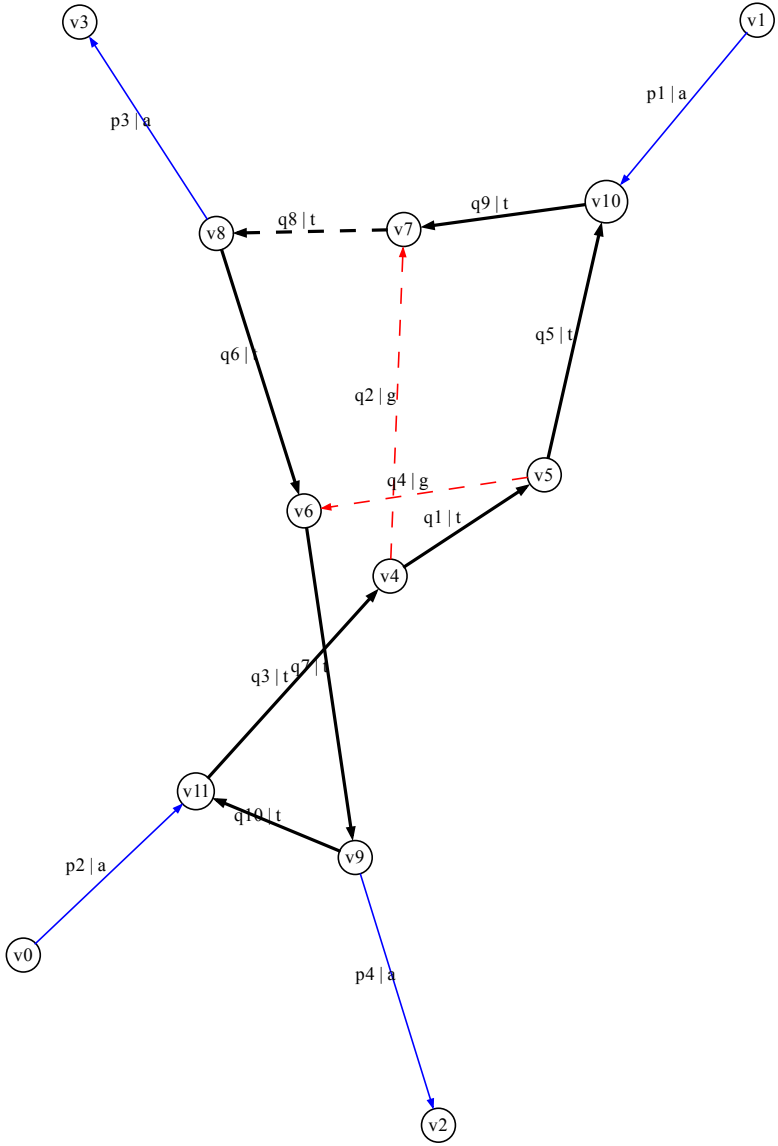

FSG GL212 #74 x ( -8 )

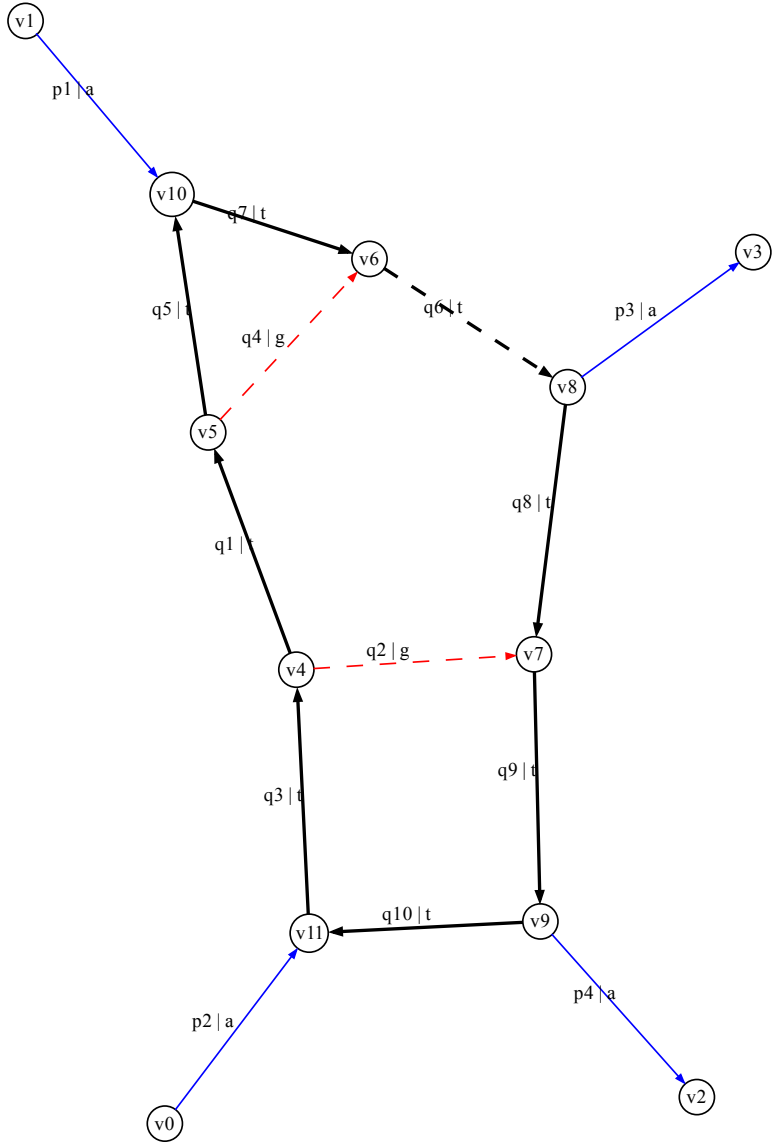

FSG GL218 #75 x ( -8 )

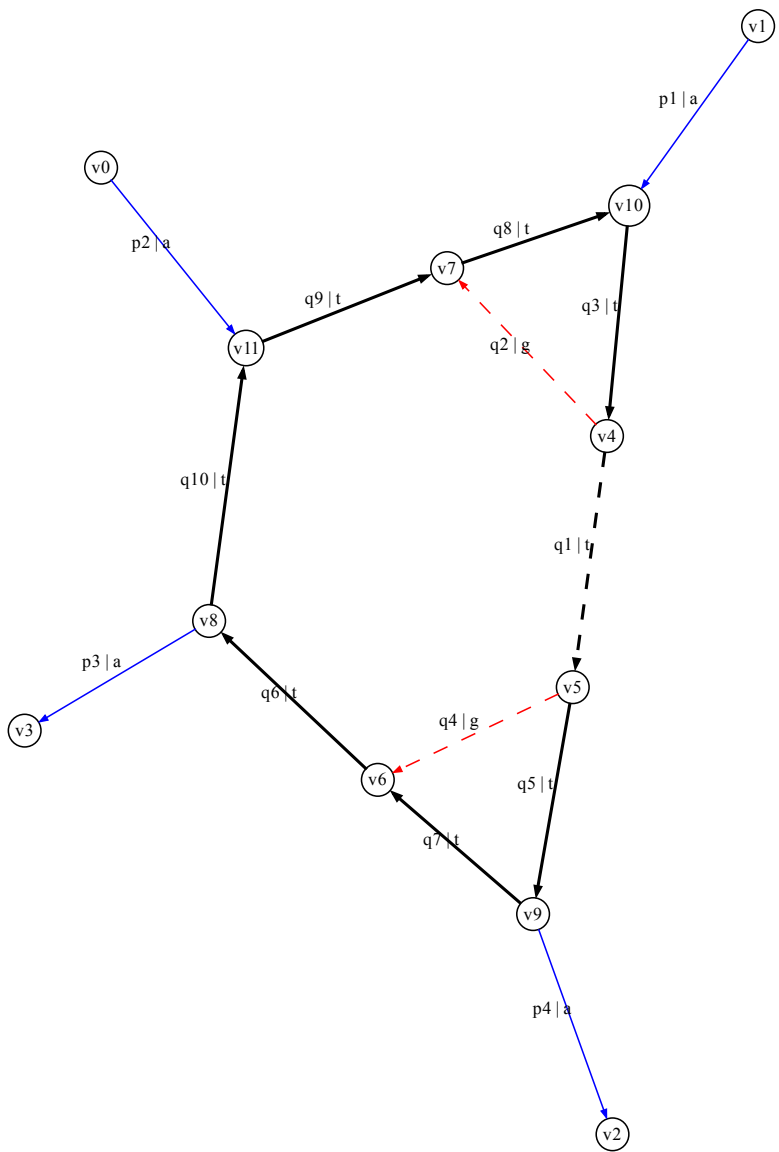

FSG GL220 #76 x ( -4 )

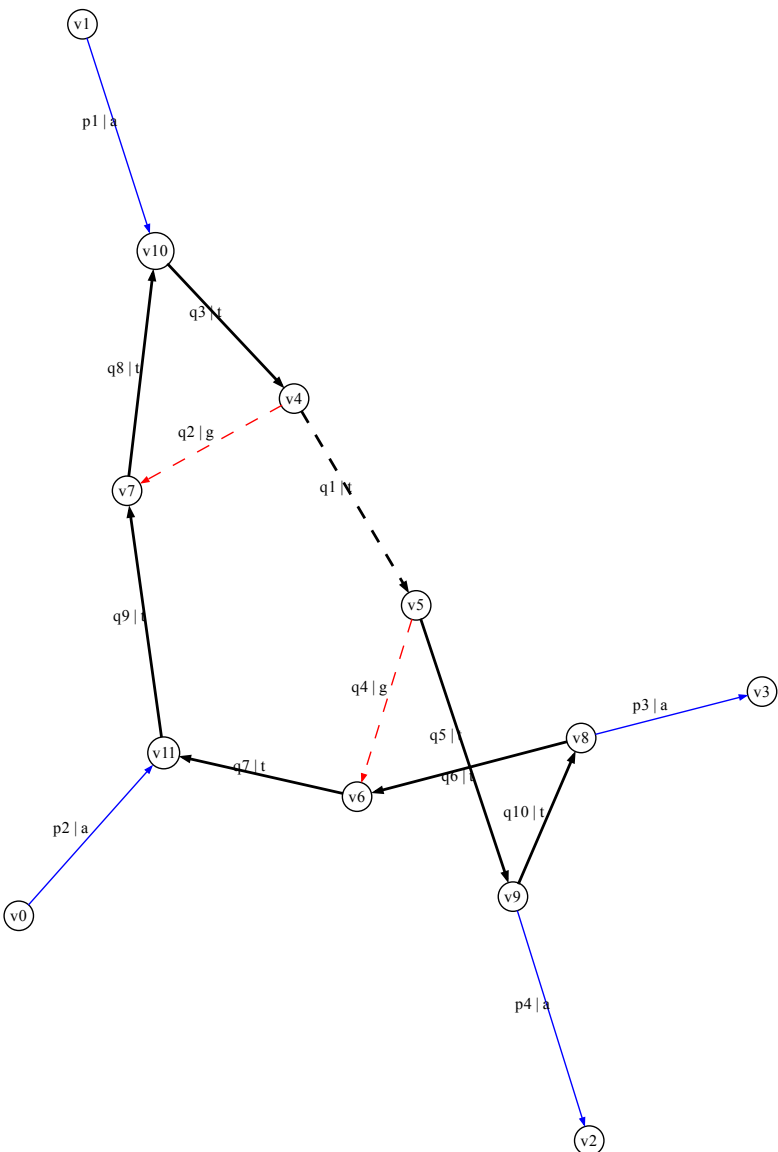

FSG GL222 #77 x ( -8 )

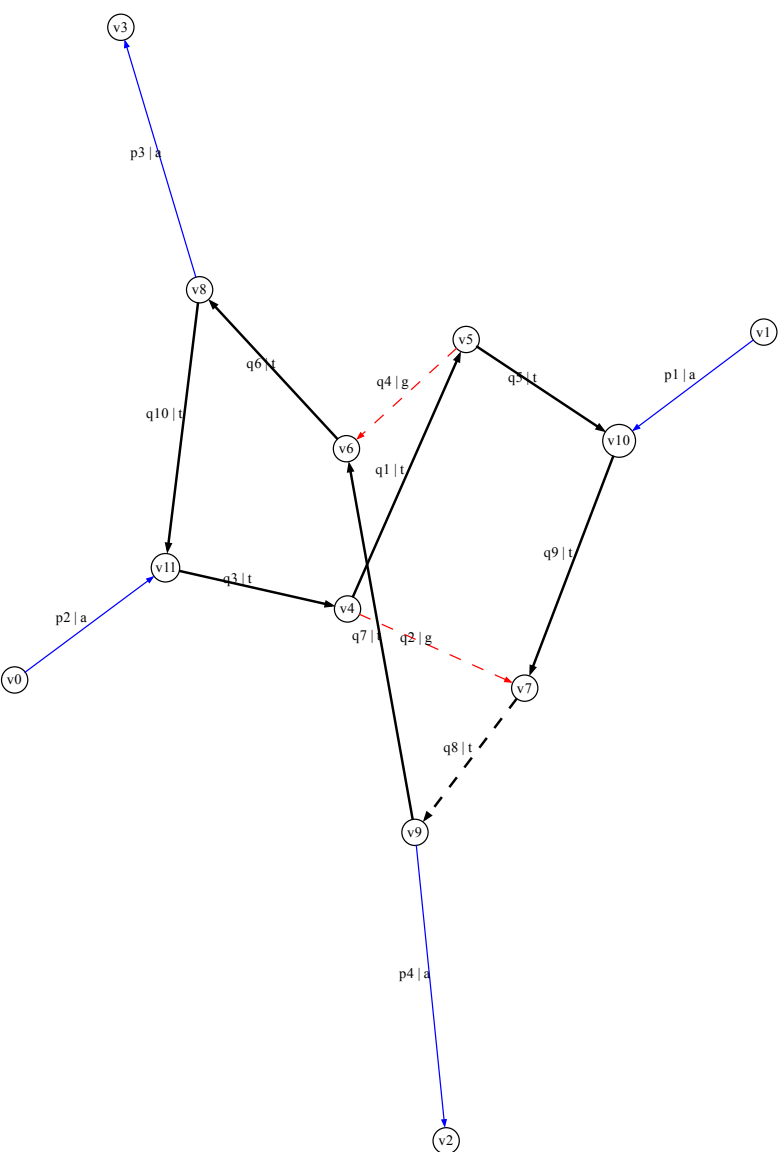

FSG GL224 #78 x ( -8 )

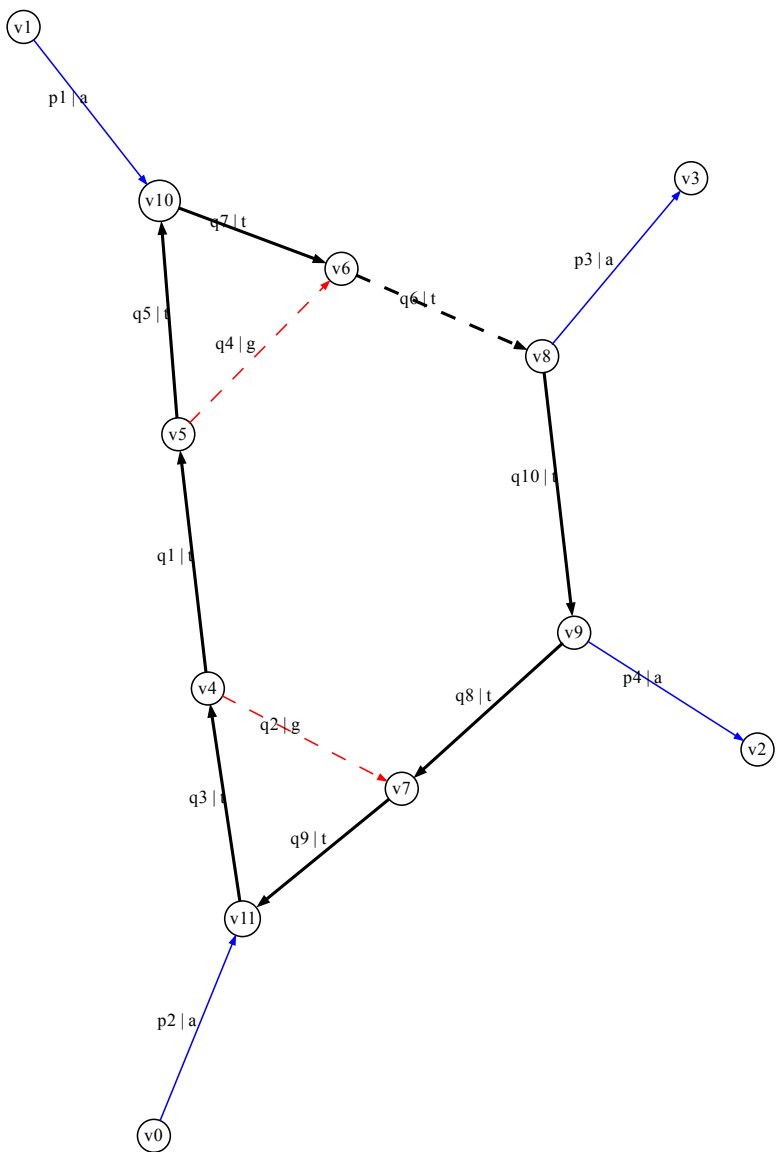

FSG GL226 #79 x ( -4 )

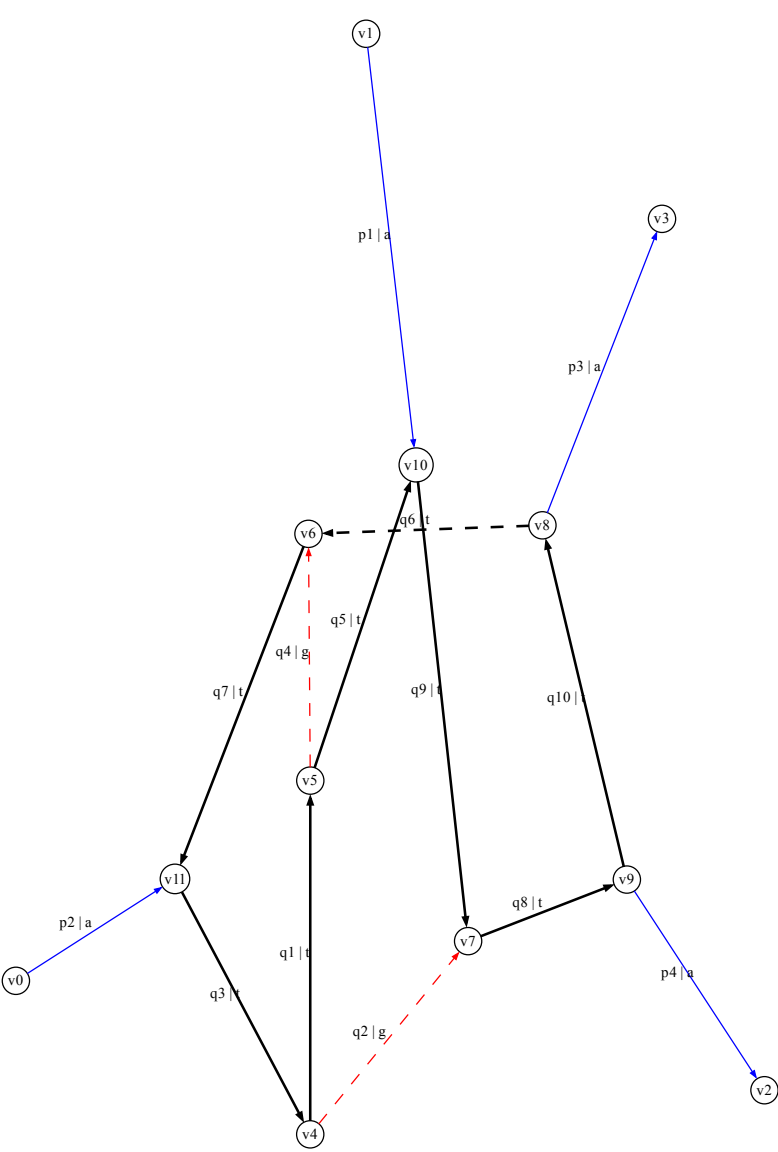

FSG GL228 #80 x ( -4 )

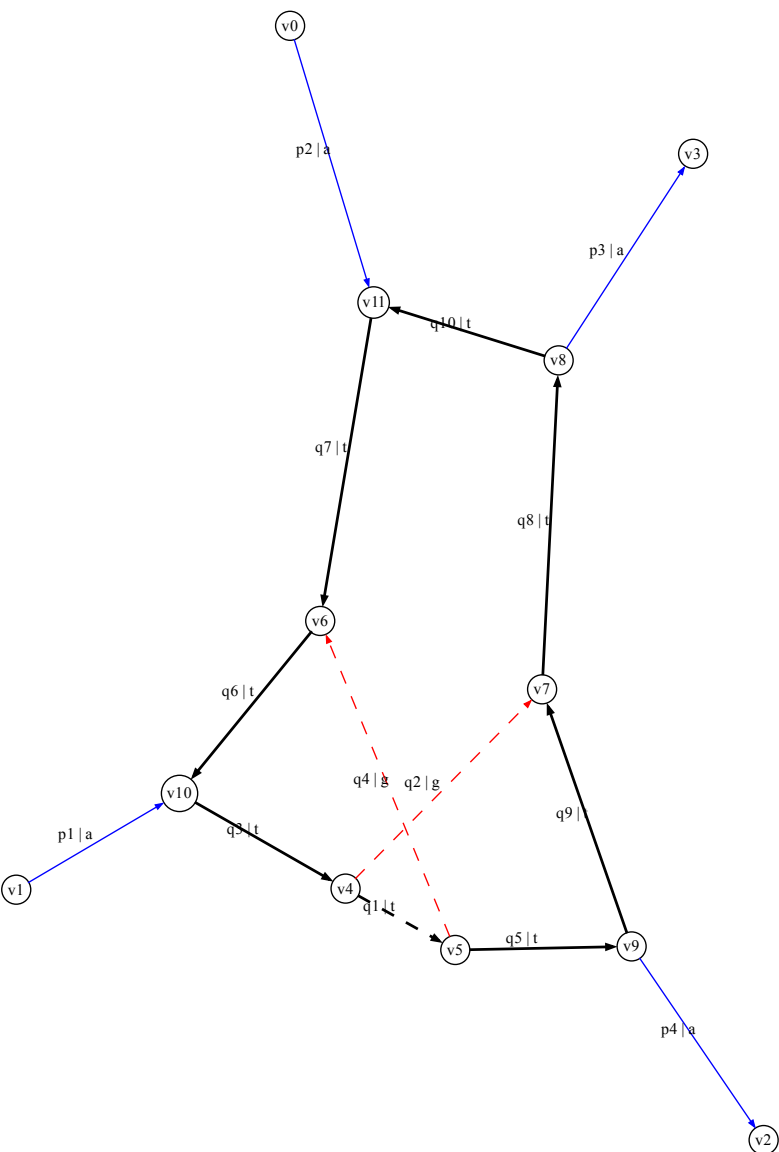

FSG GL230 #81 x ( -4 )

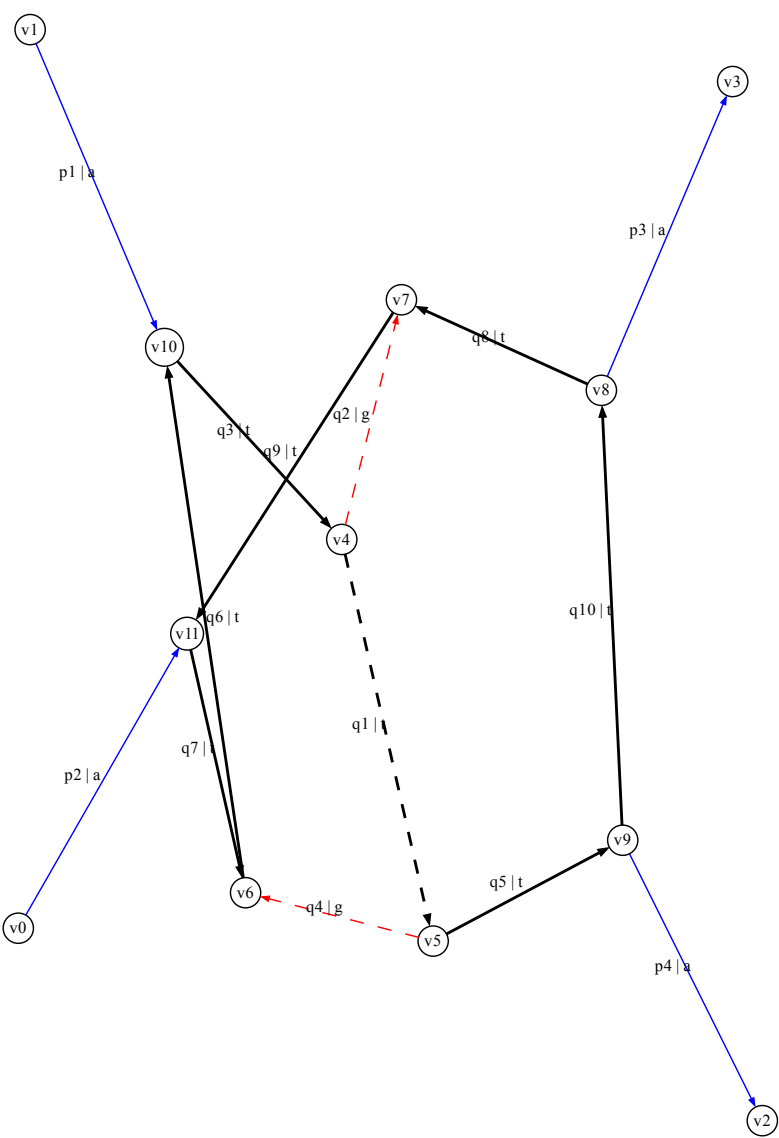

FSG GL232 #82 x (-8)

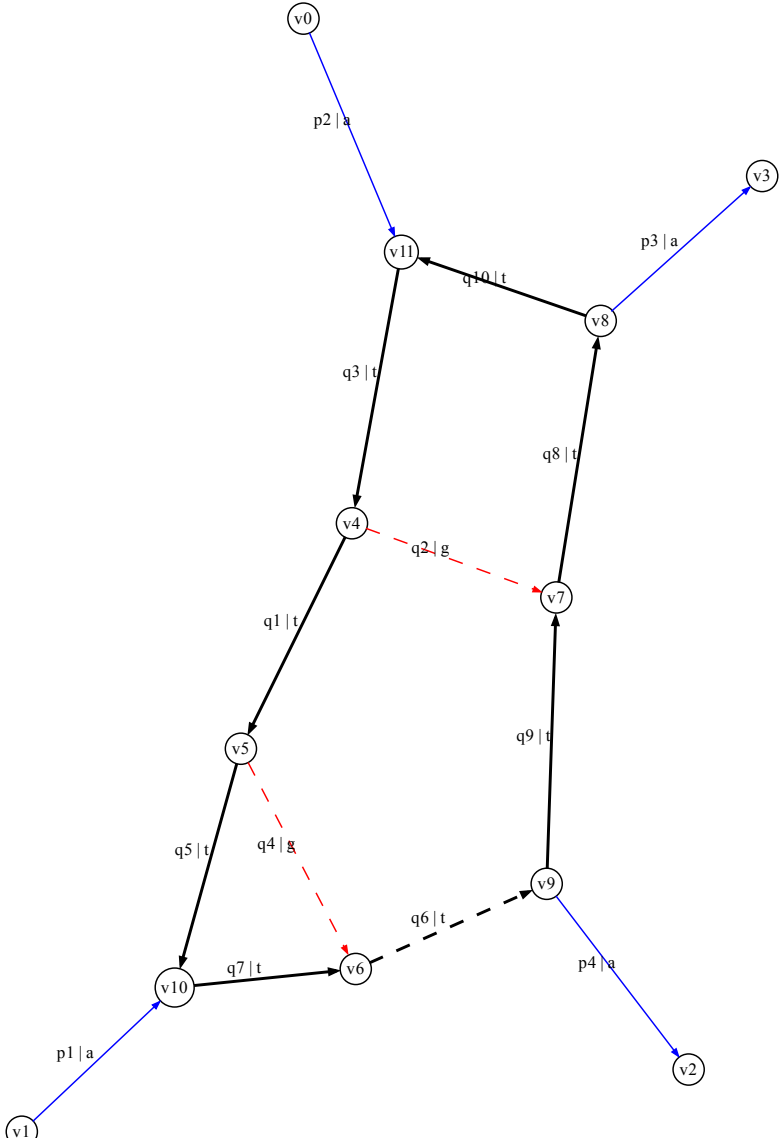

FSG GL238 #83 x (-8)

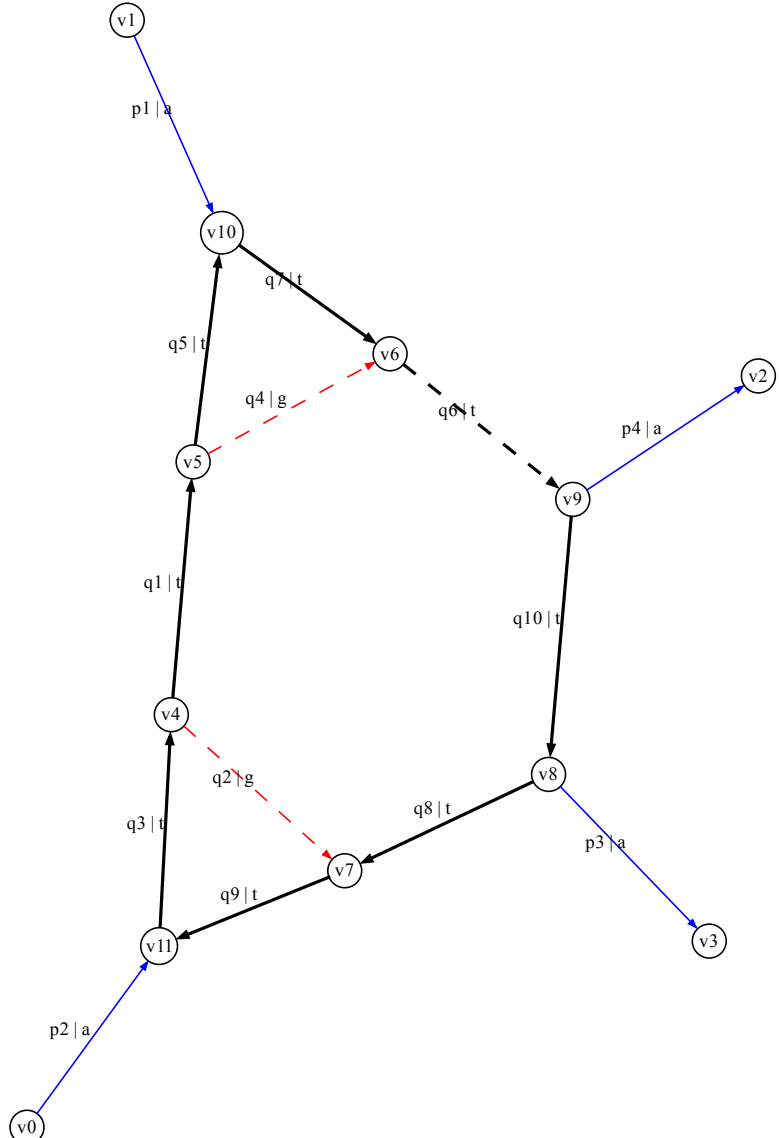

FSG GL244 #84 x (-4)

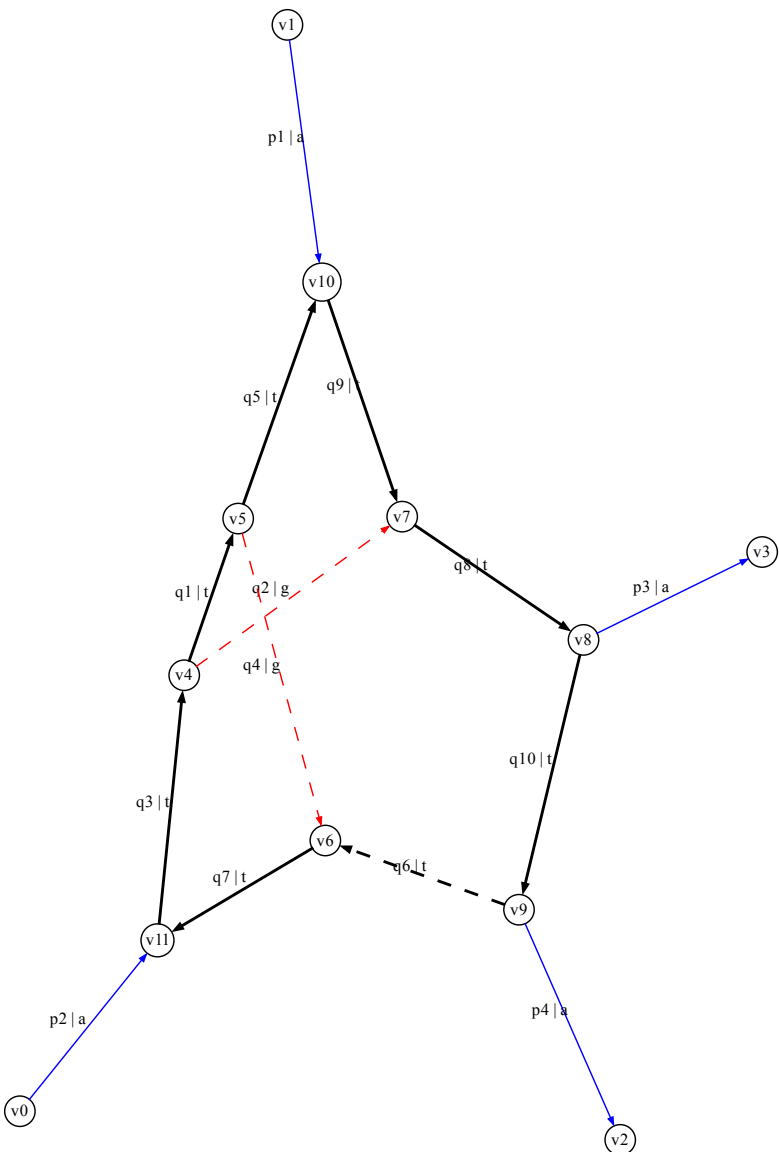

FSG GL246 #85 x (-4)

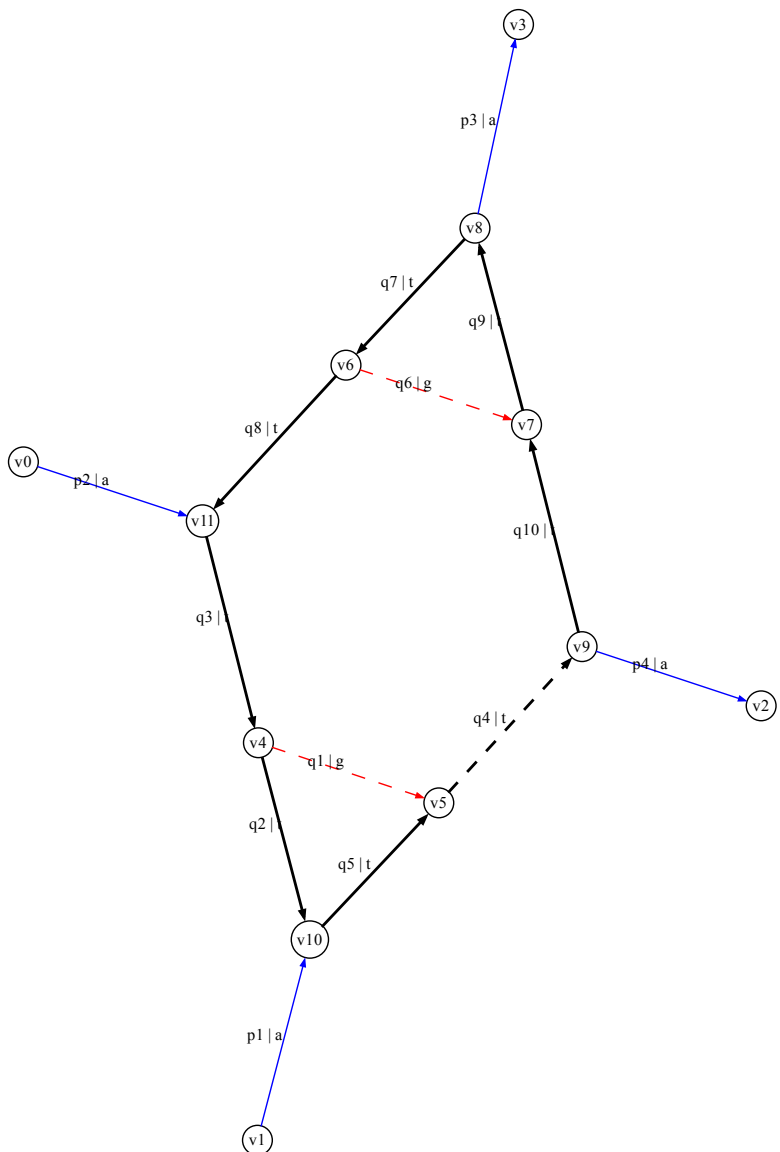

FSG GL256 #86 x (-4)

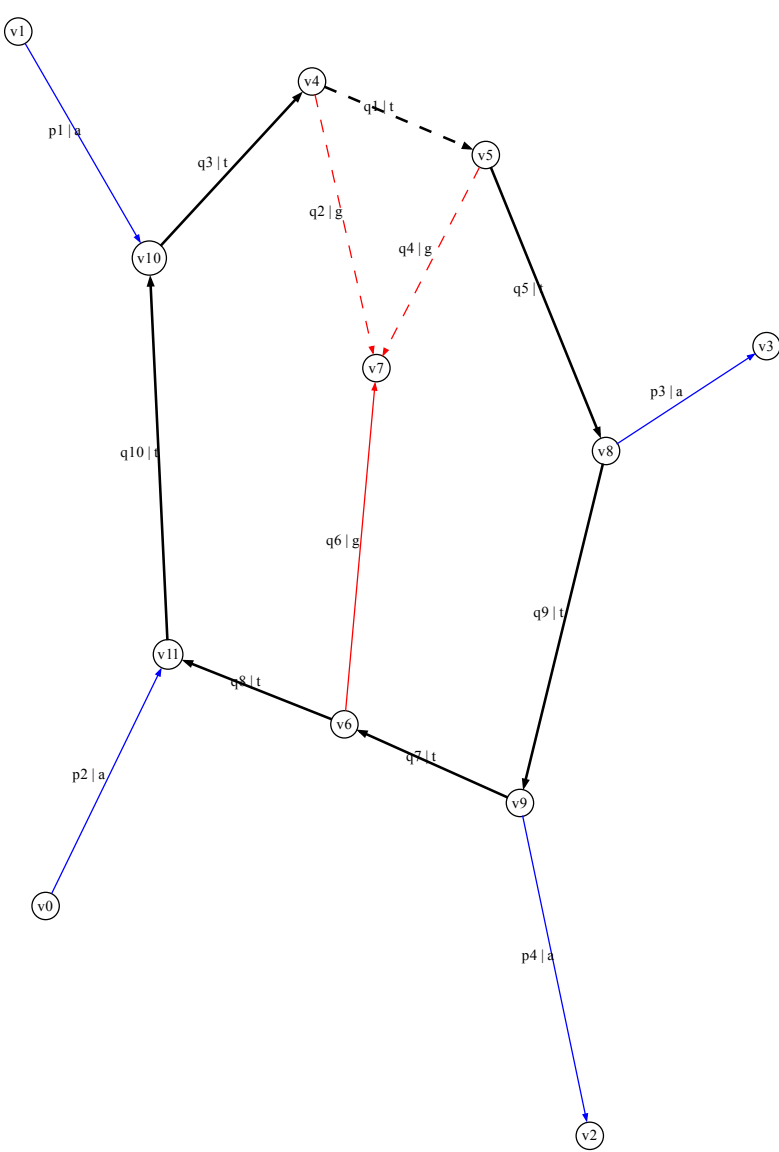

FSG GL258 #87 x (-4)

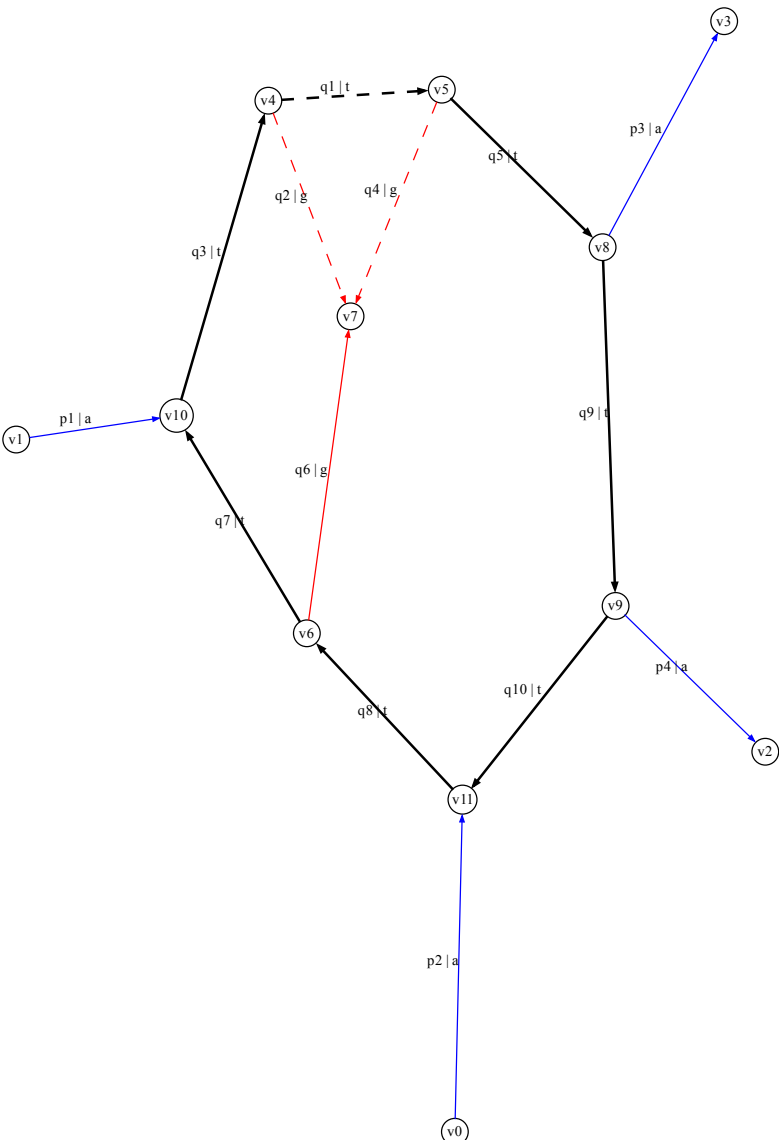

FSG GL260 #88 x (-8)

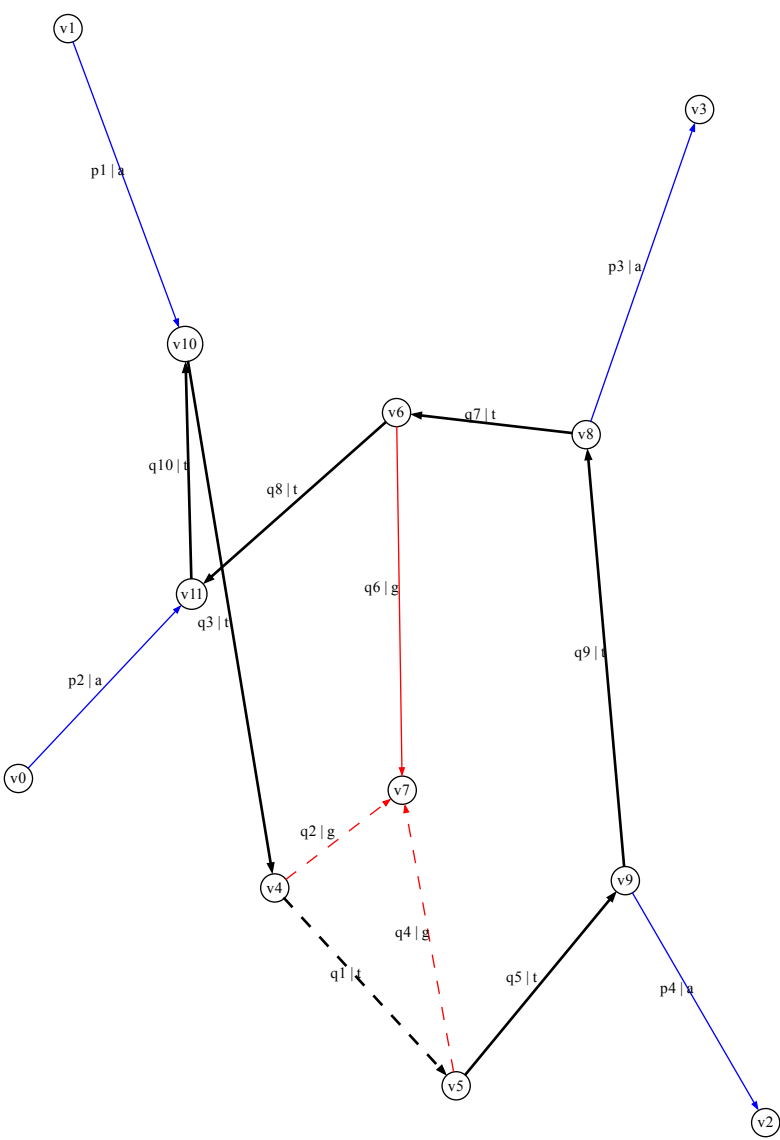

FSG GL262 #89 x (-4)

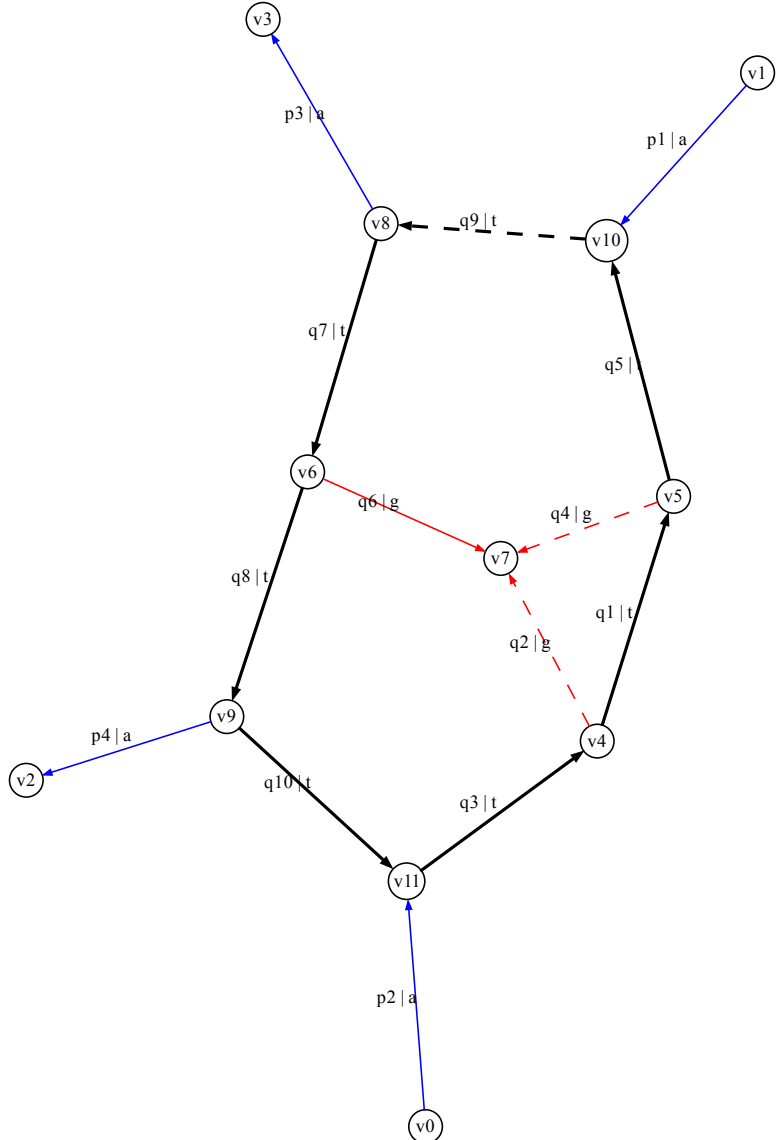

FSG GL268 #90 x (-4)

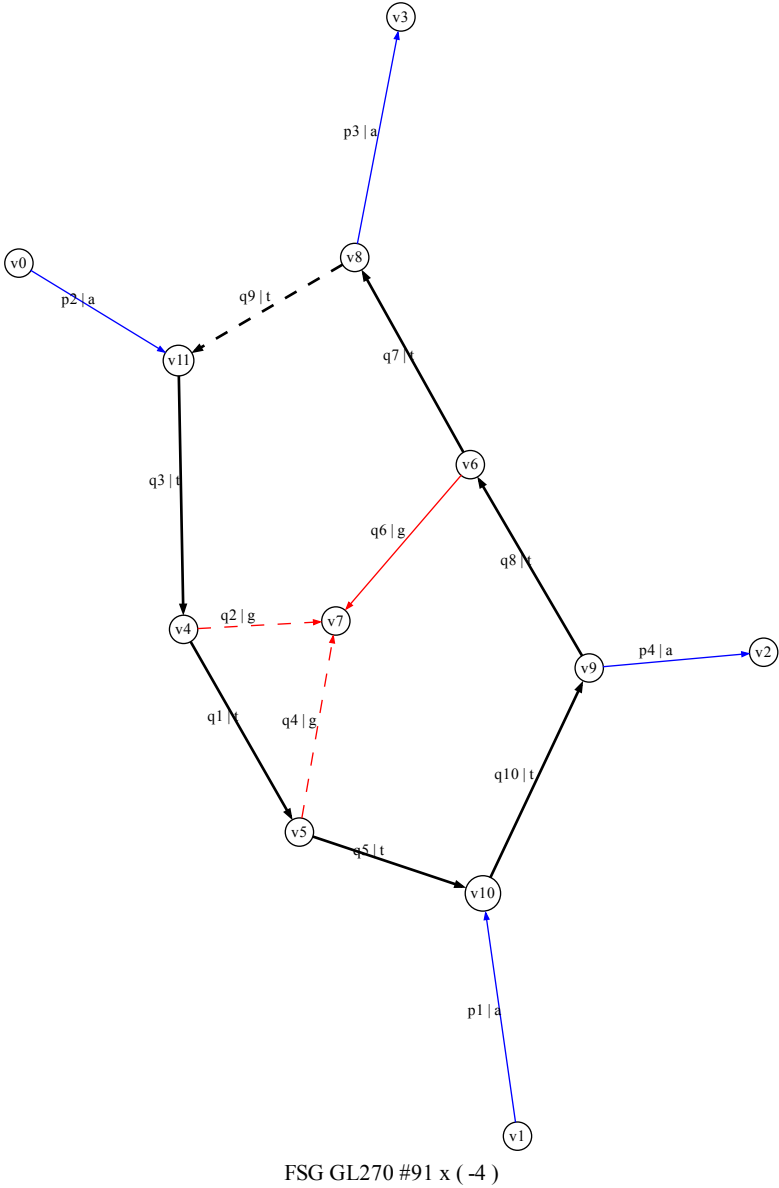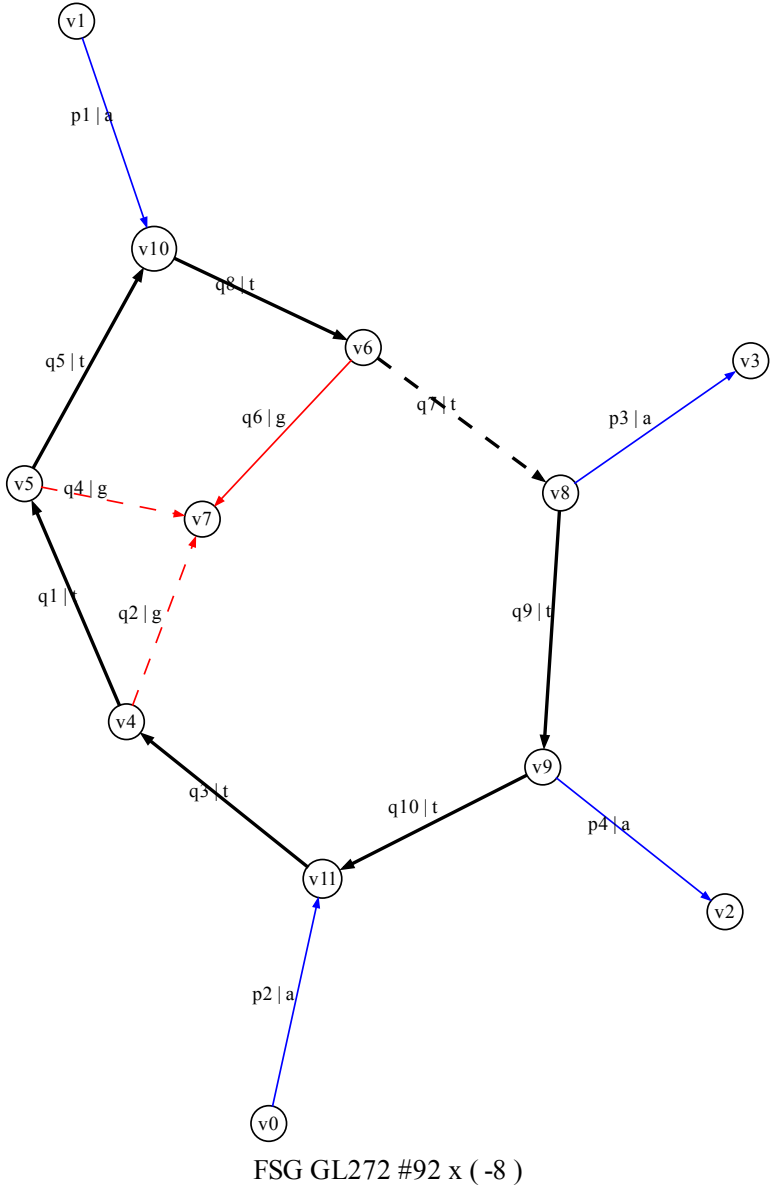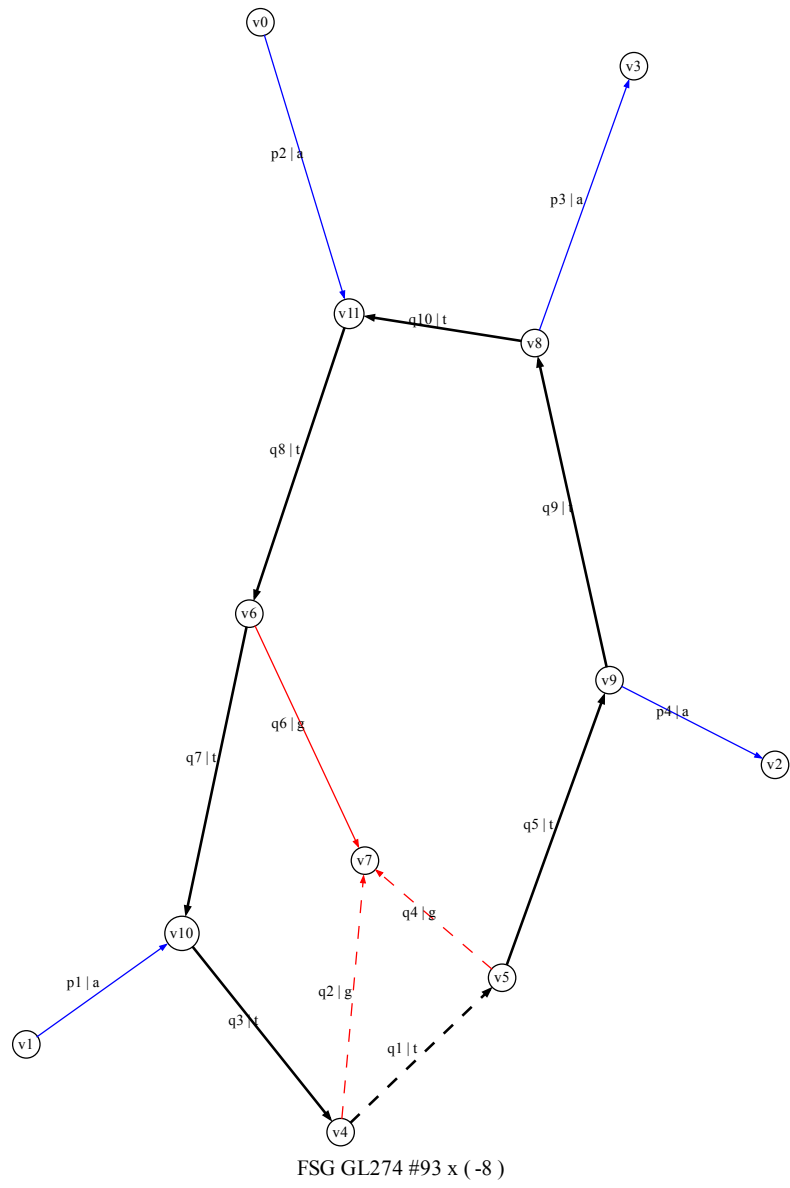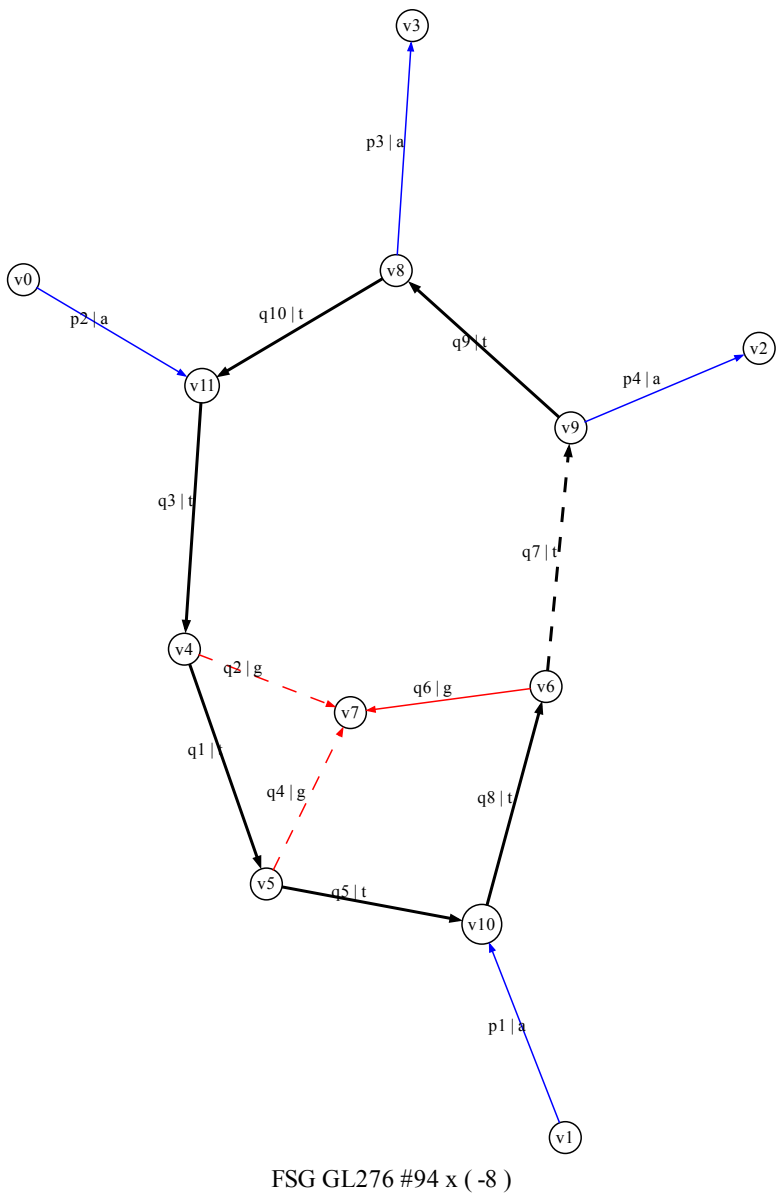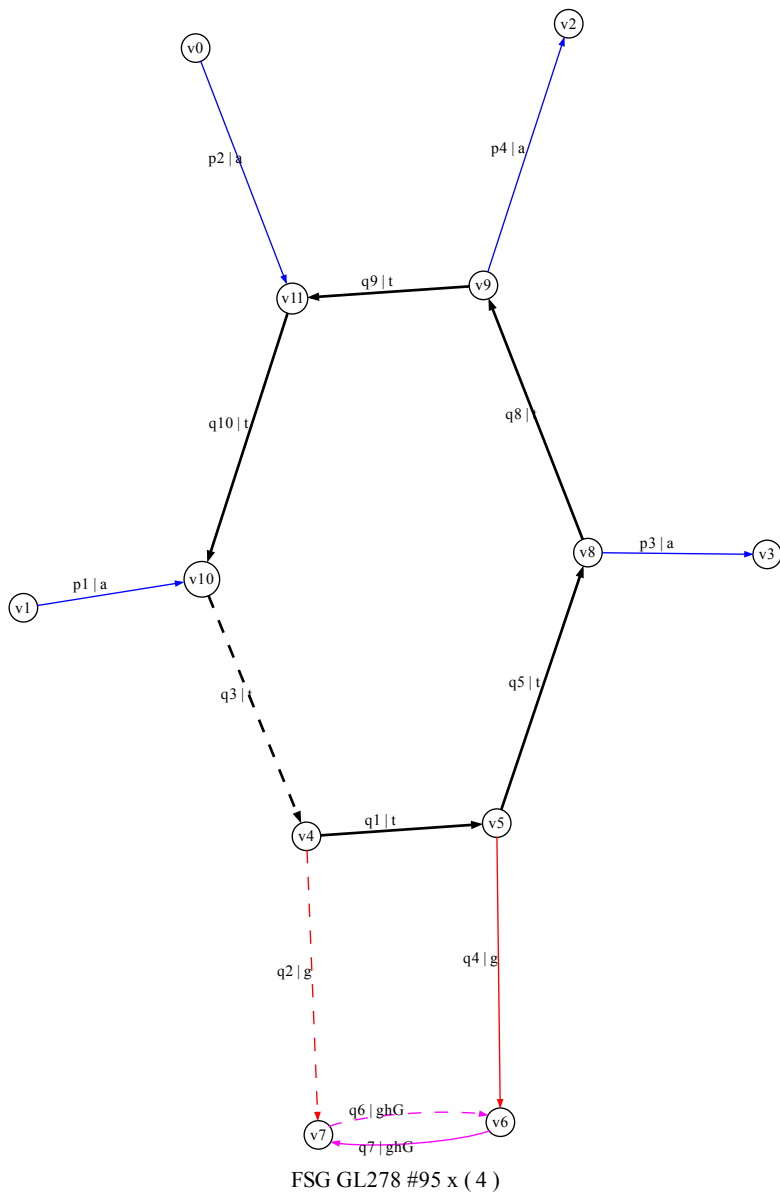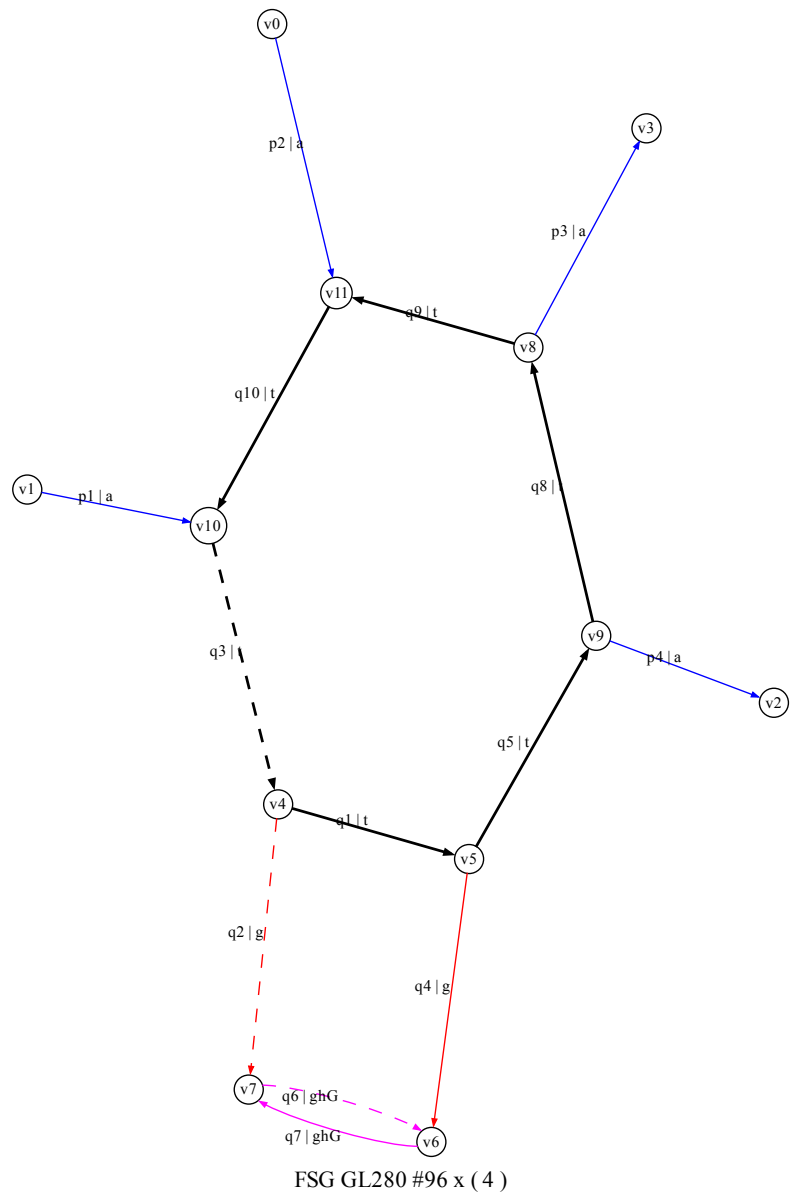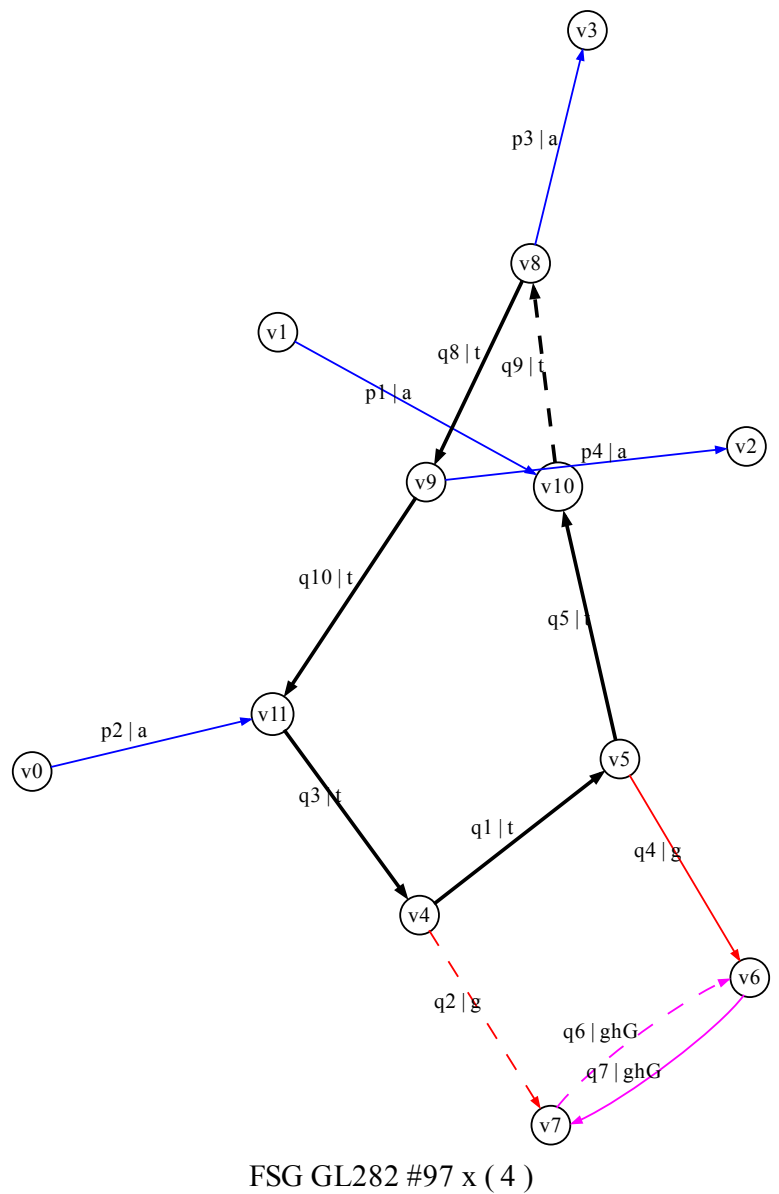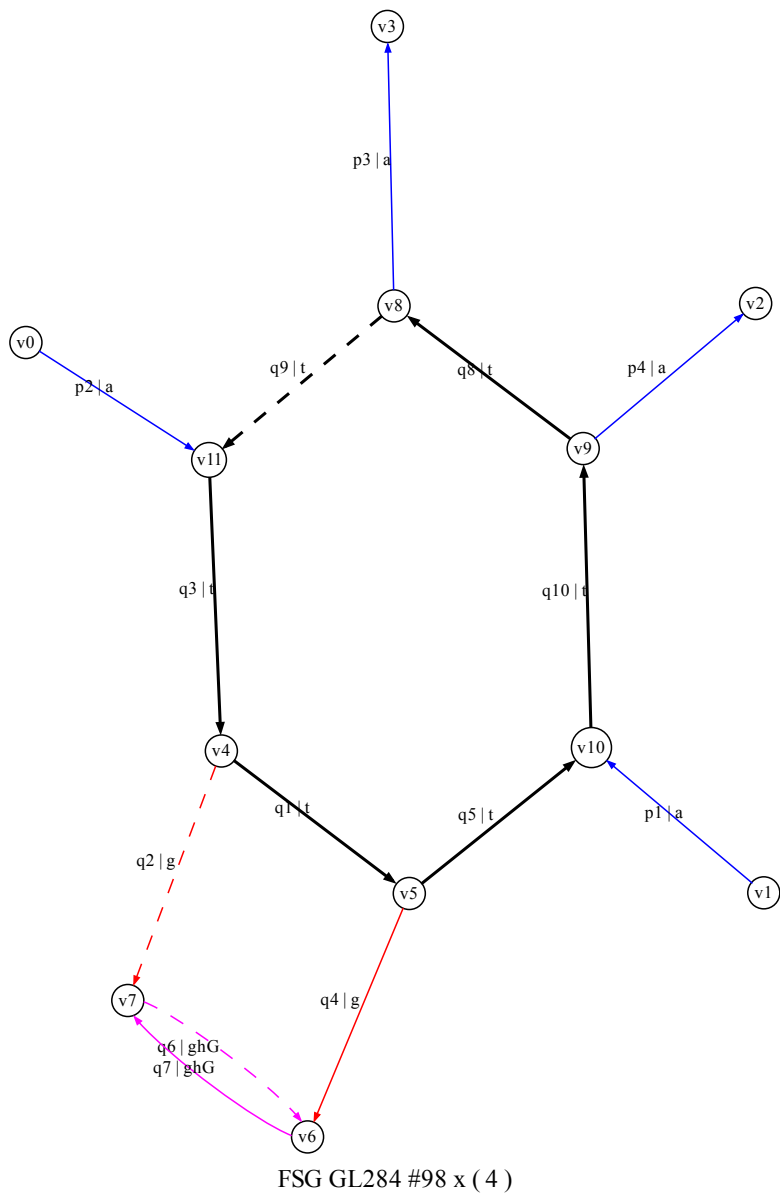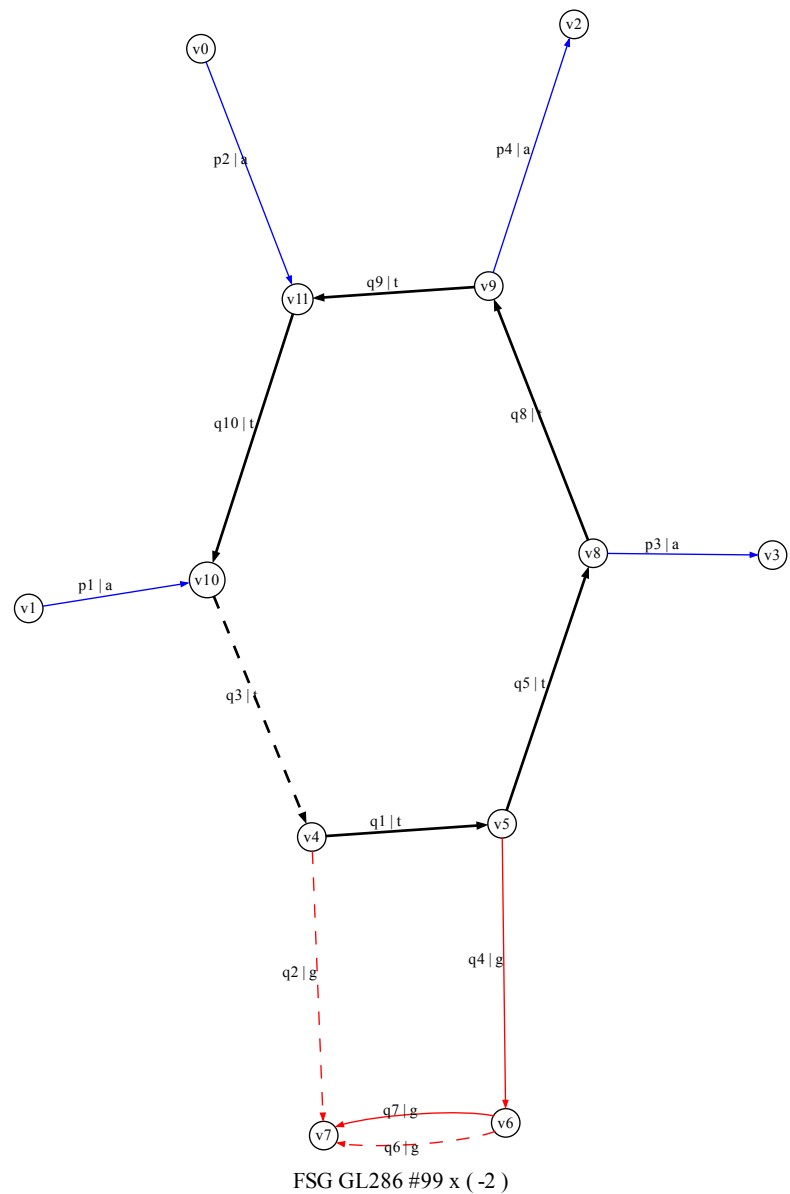

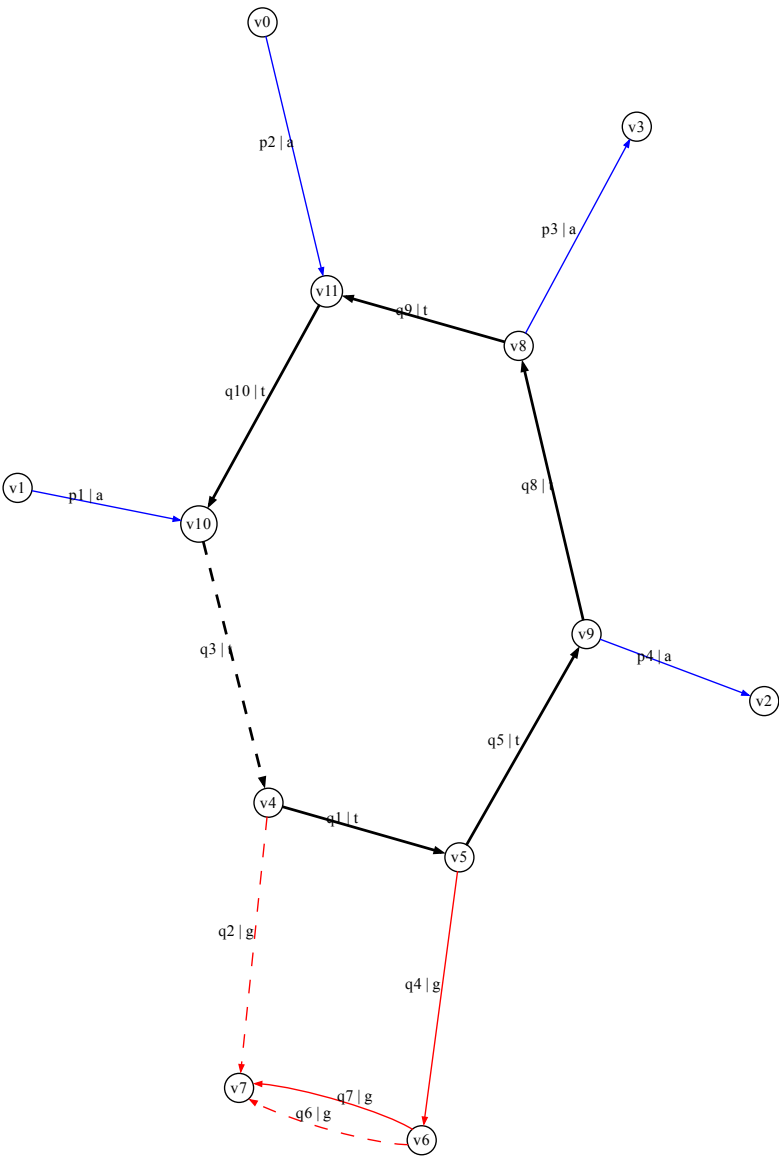

FSG GL288 #100 x (-2)

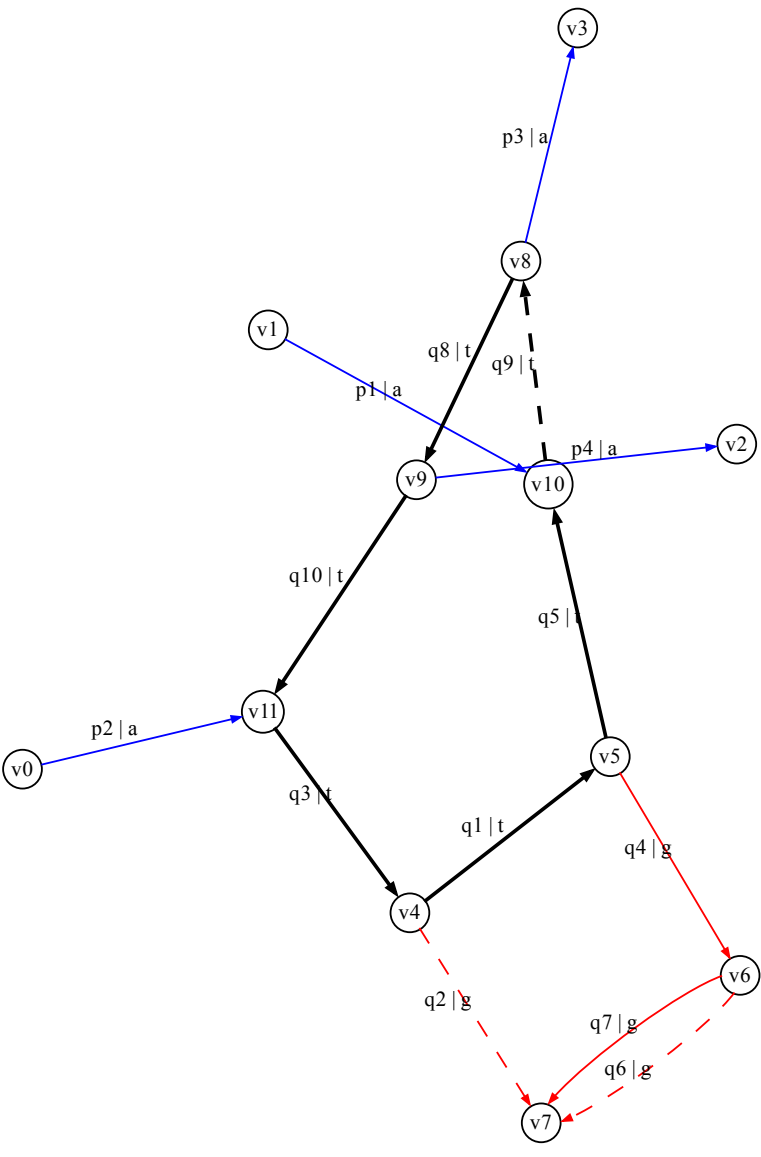

FSG GL290 #101 x (-2)

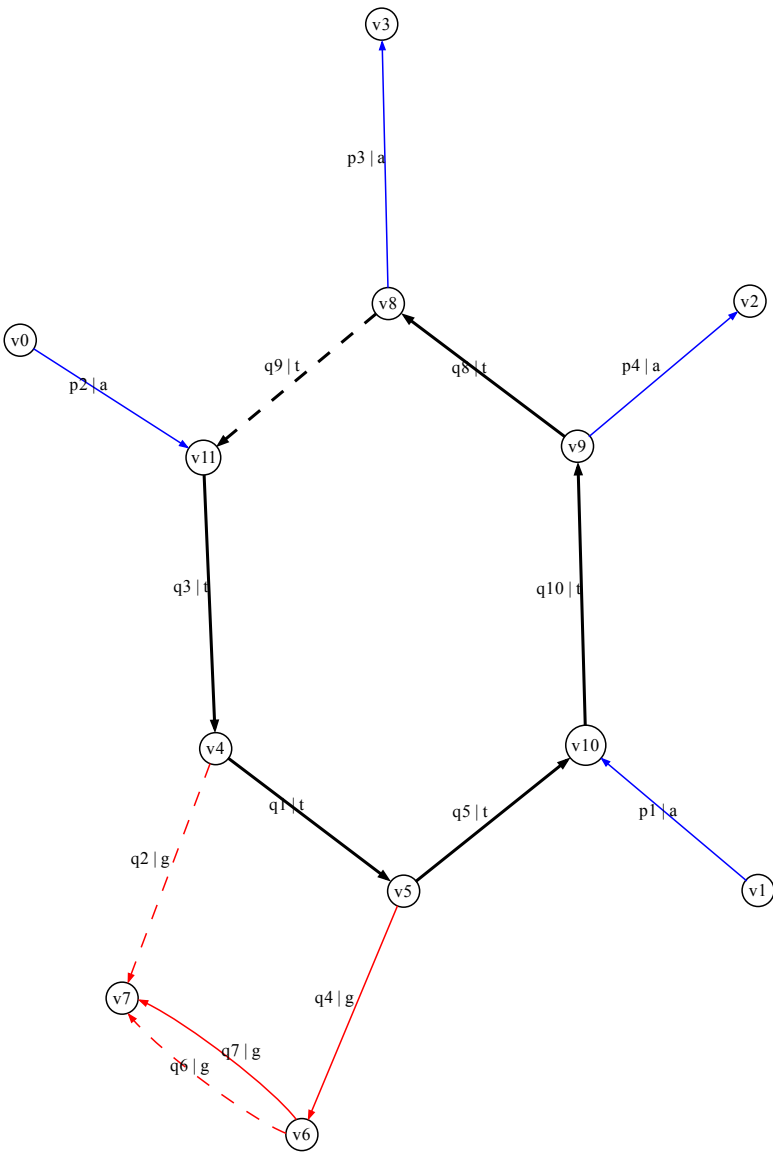

FSG GL292 #102 x (-2)

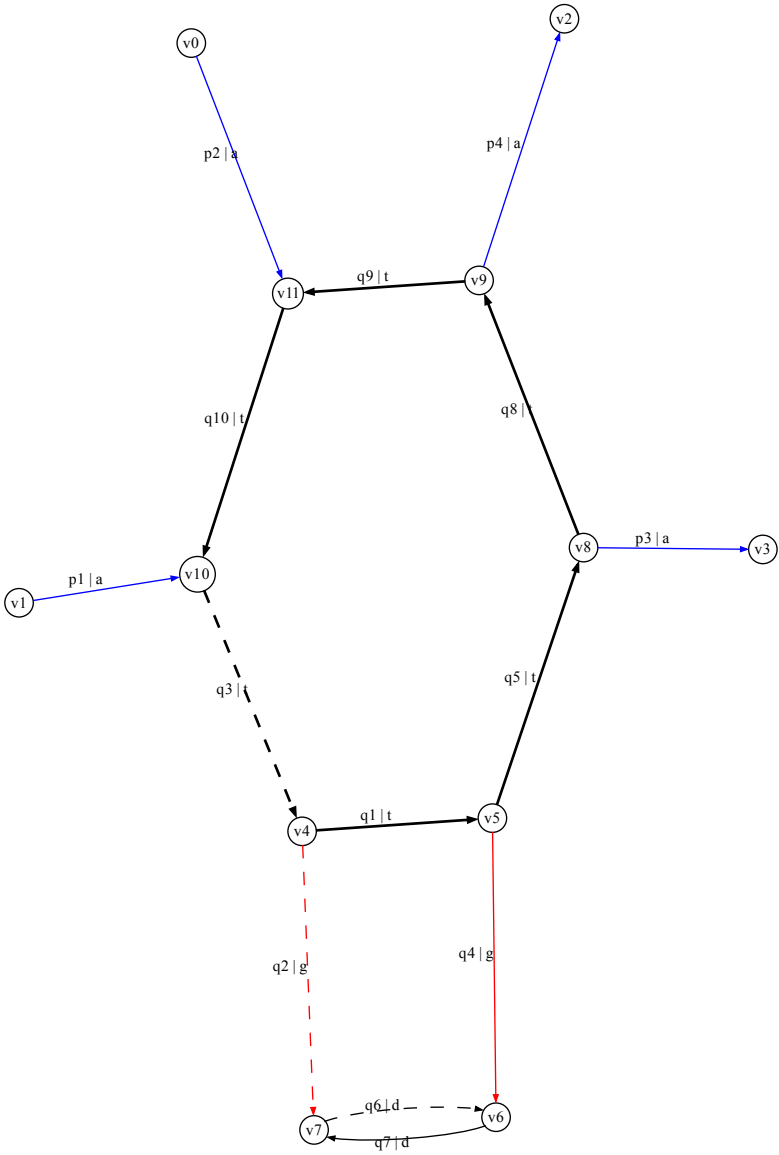

FSG GL294 #103 x (4)

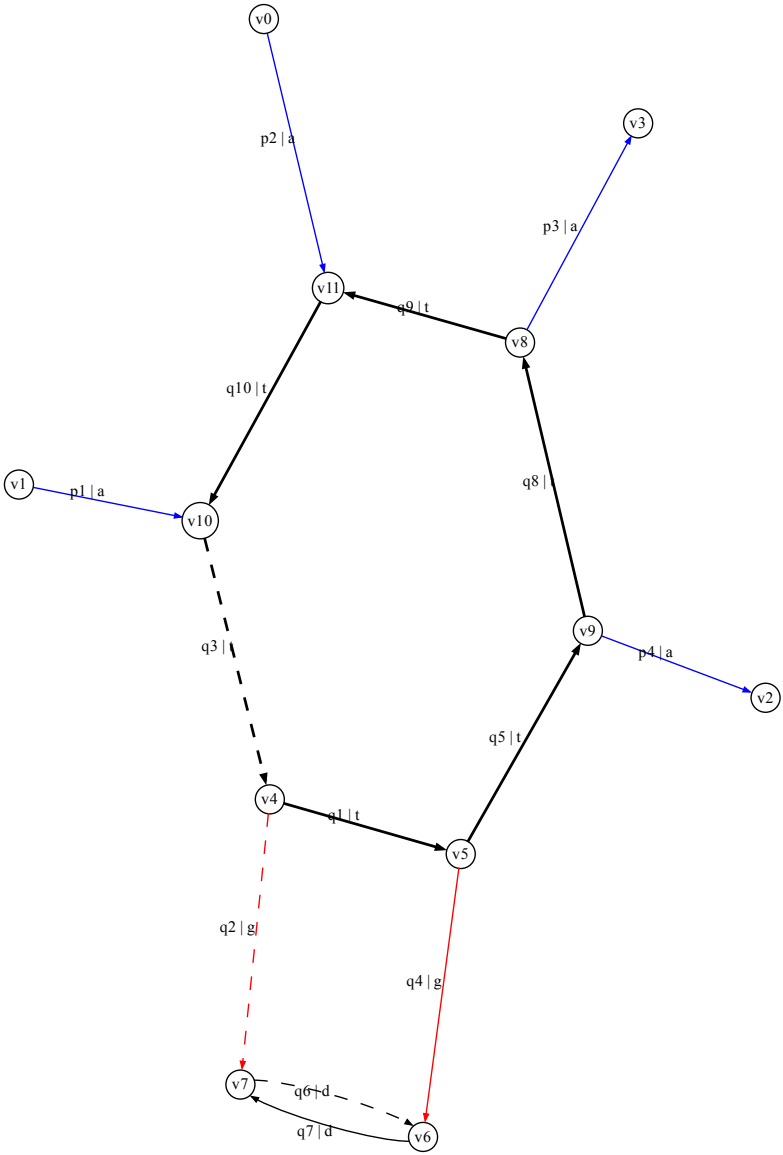

FSG GL296 #104 x (4)

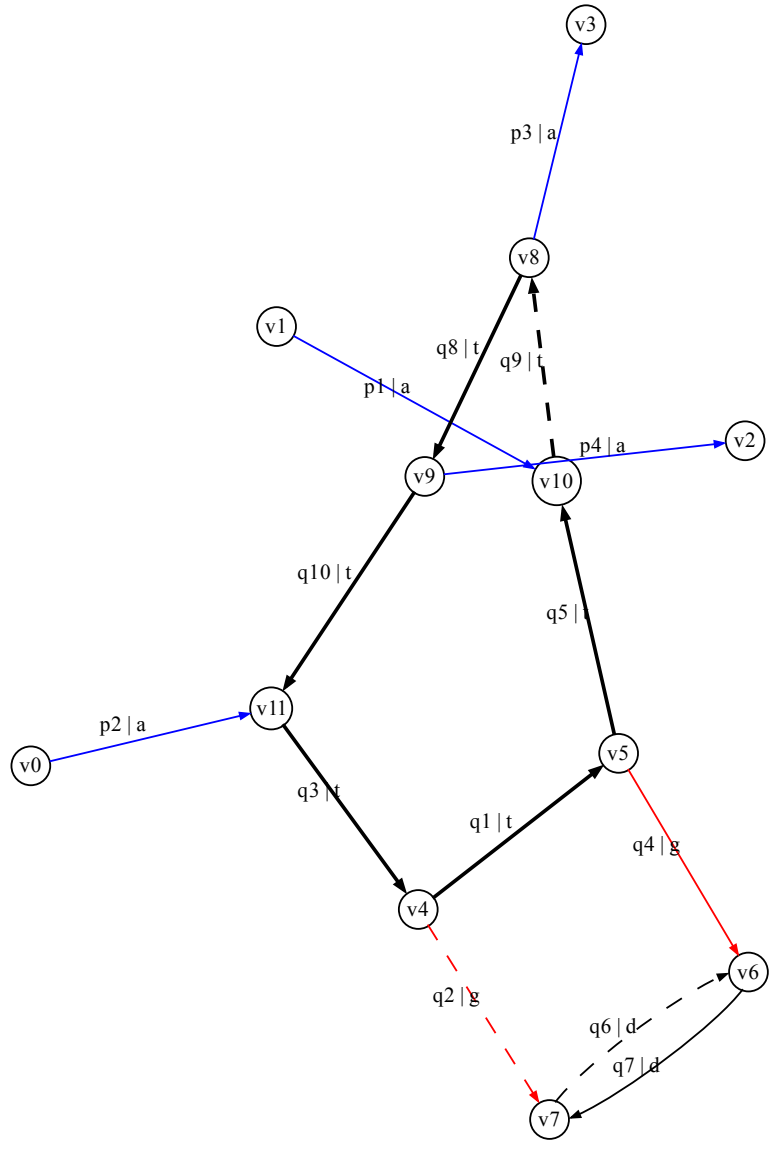

FSG GL298 #105 x (4)

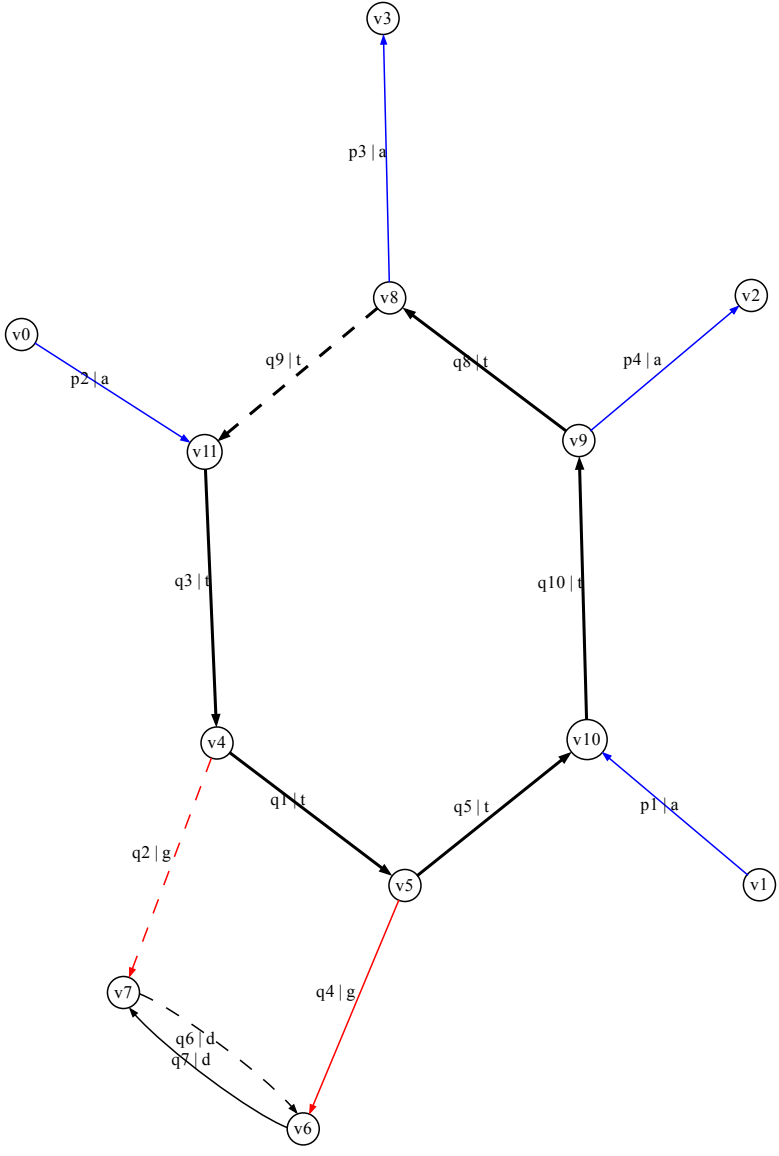

FSG GL300 #106 x (4)

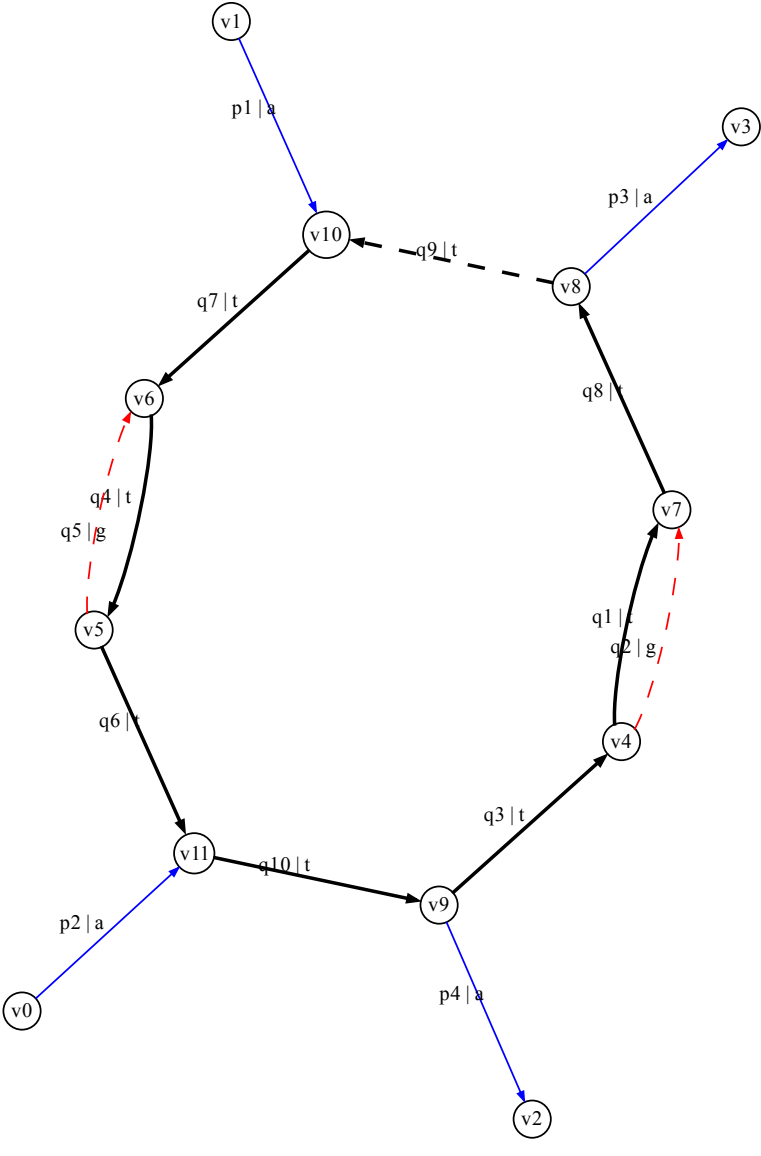

FSG GL362 #107 x (-2)

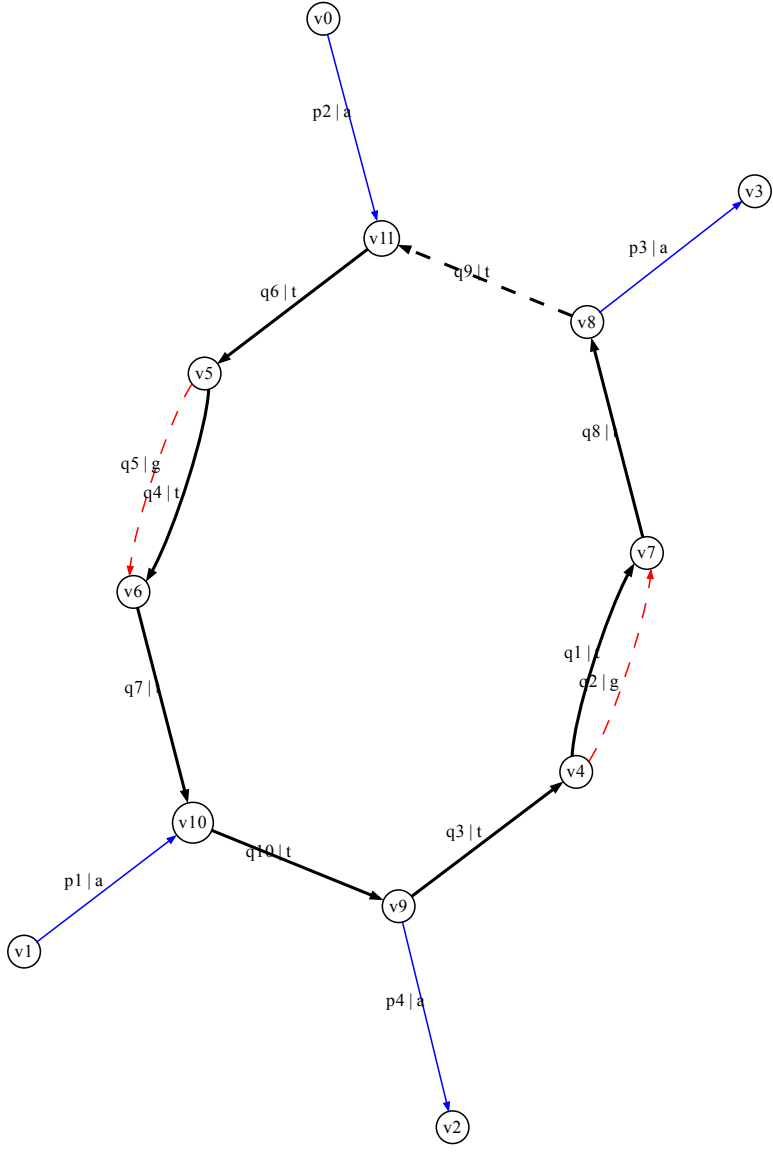

FSG GL364 #108 x (-2)

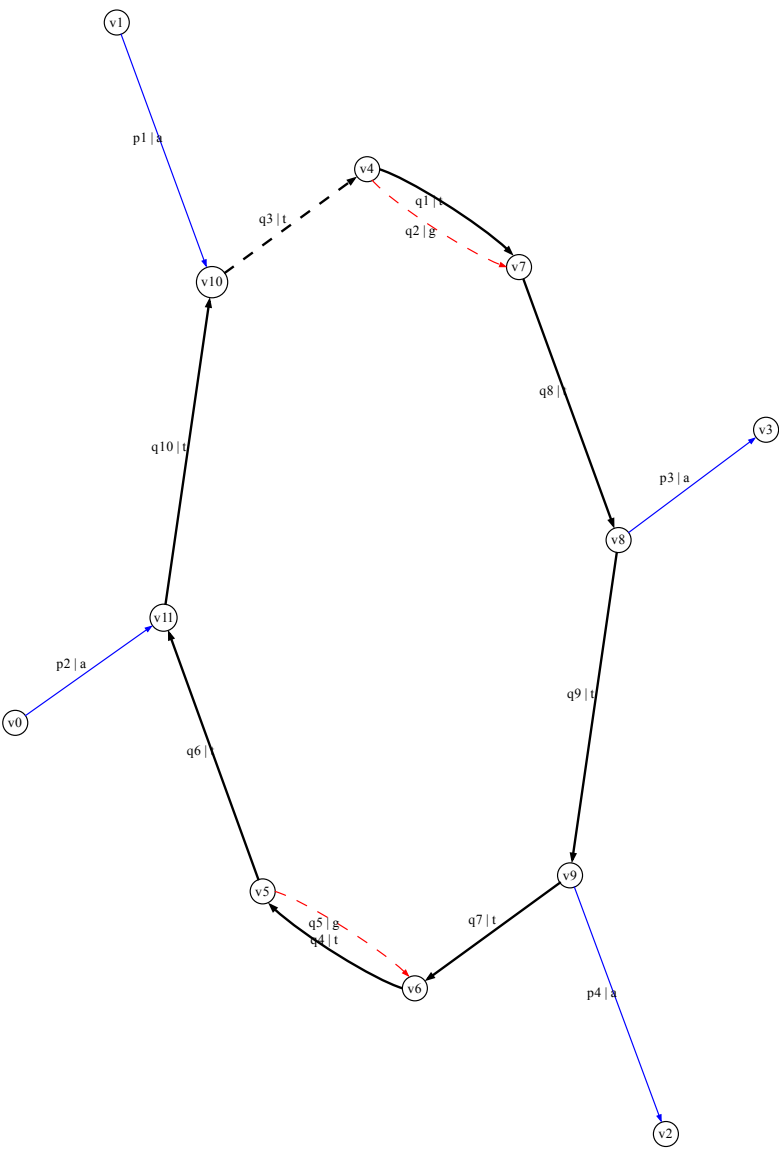

FSG GL366 #109 x (-2)

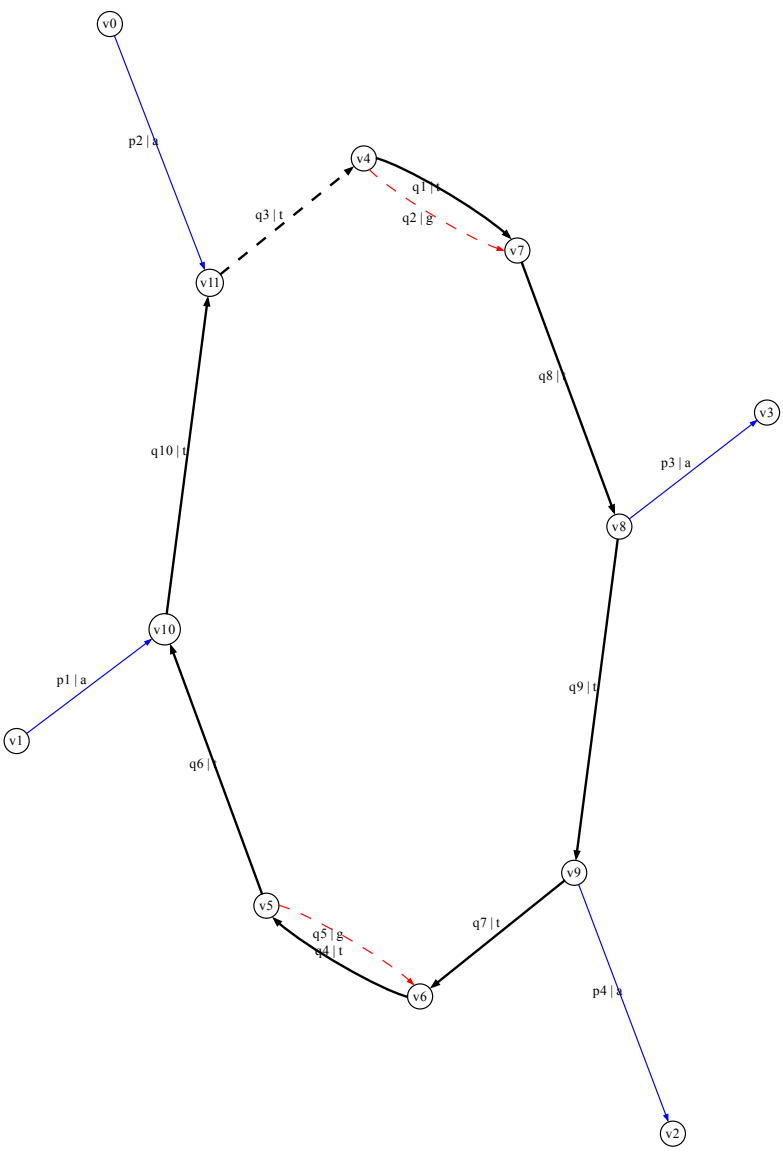

FSG GL368 #110 x (-2)

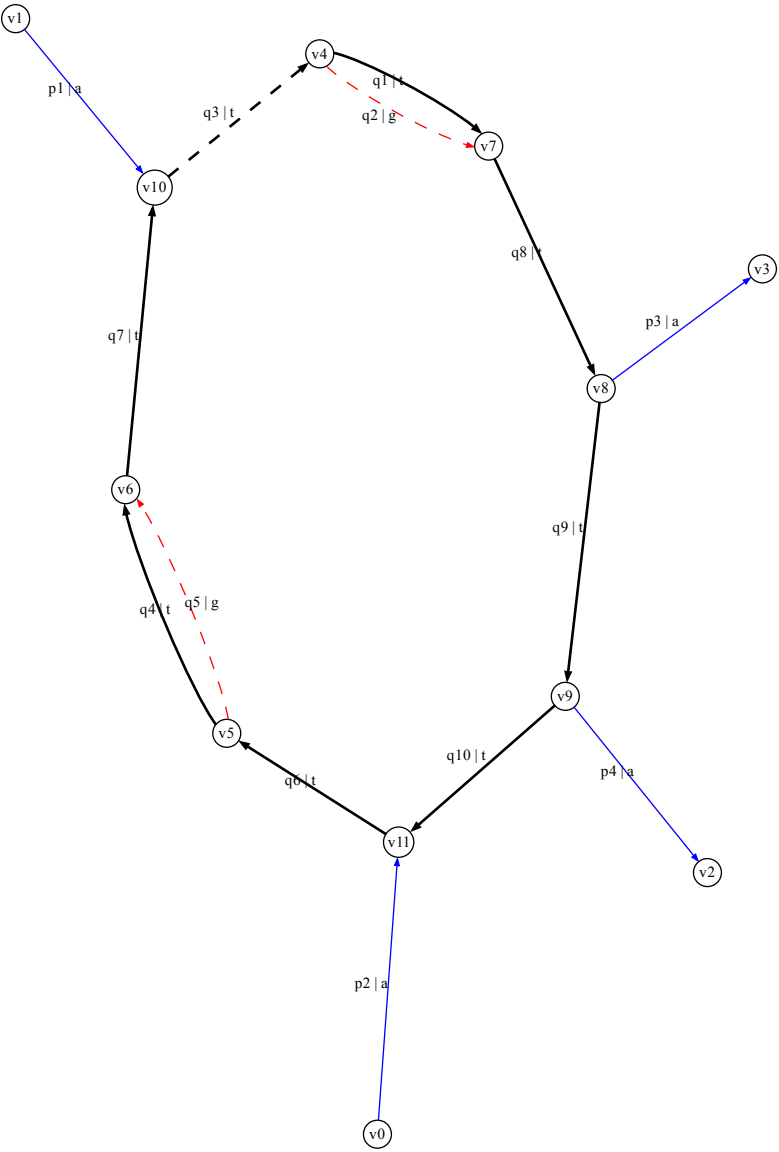

FSG GL370 #111 x (-8)

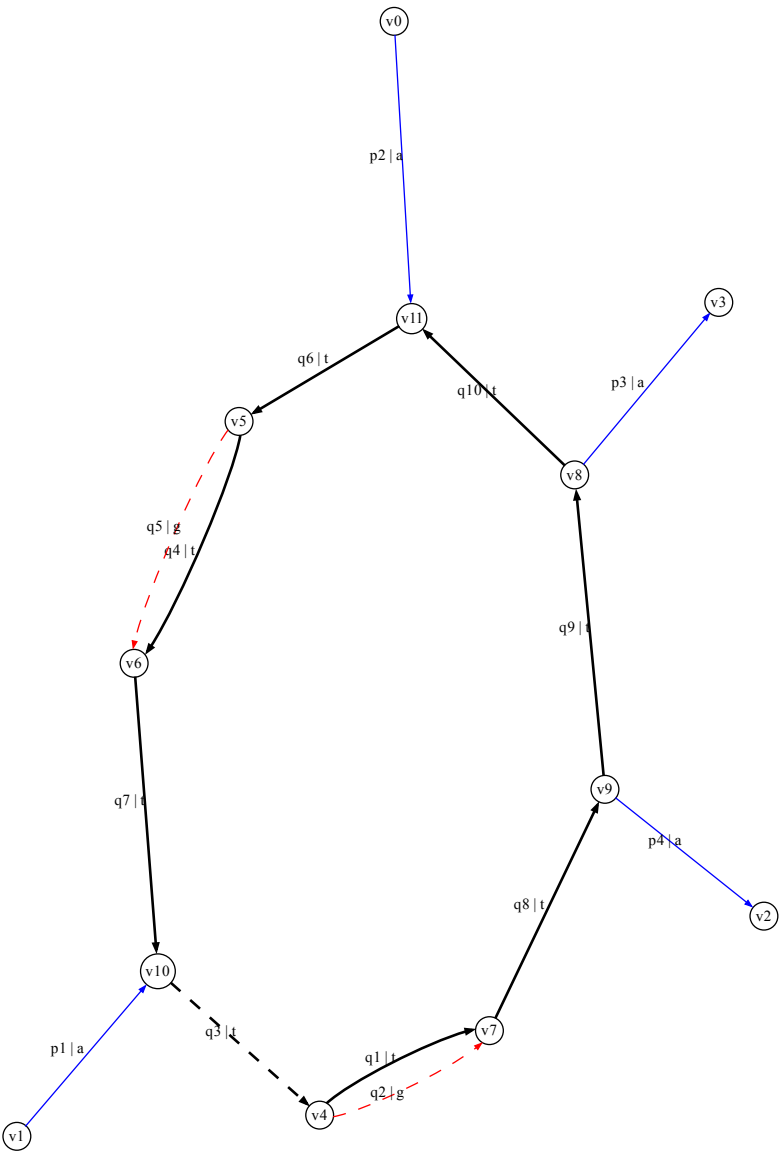

FSG GL372 #112 x (-8)

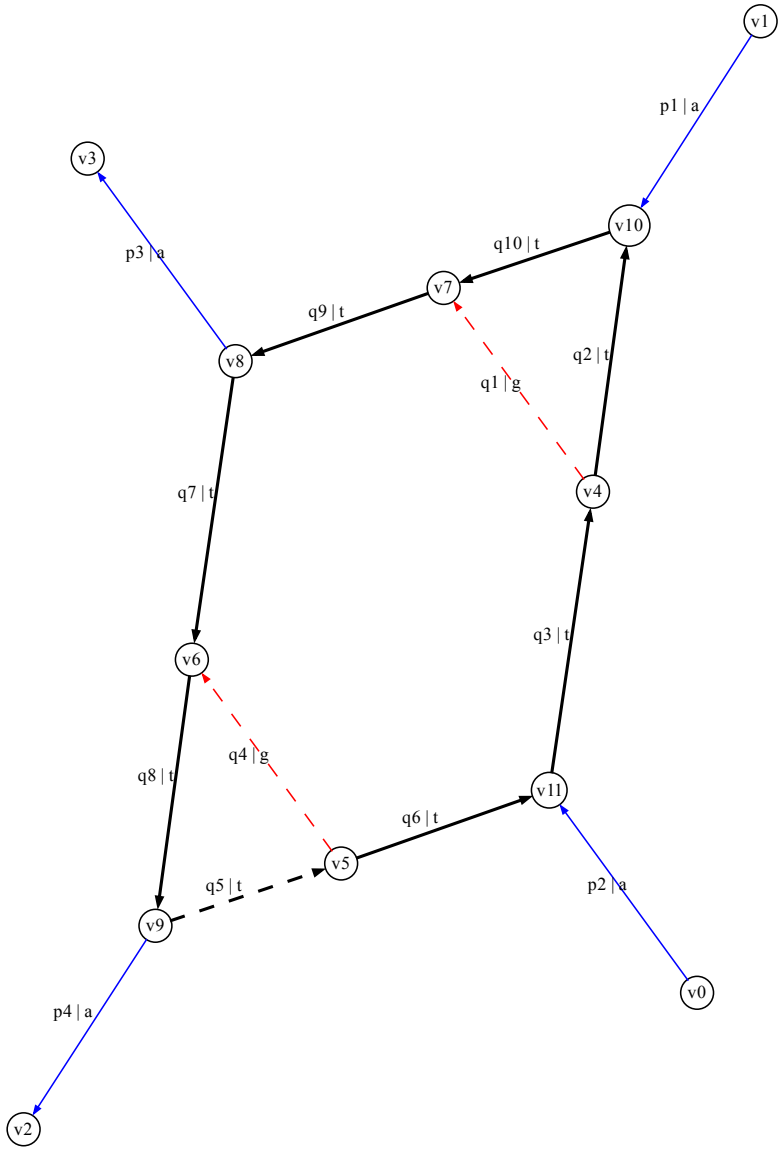

FSG GL374 #113 x (-4)

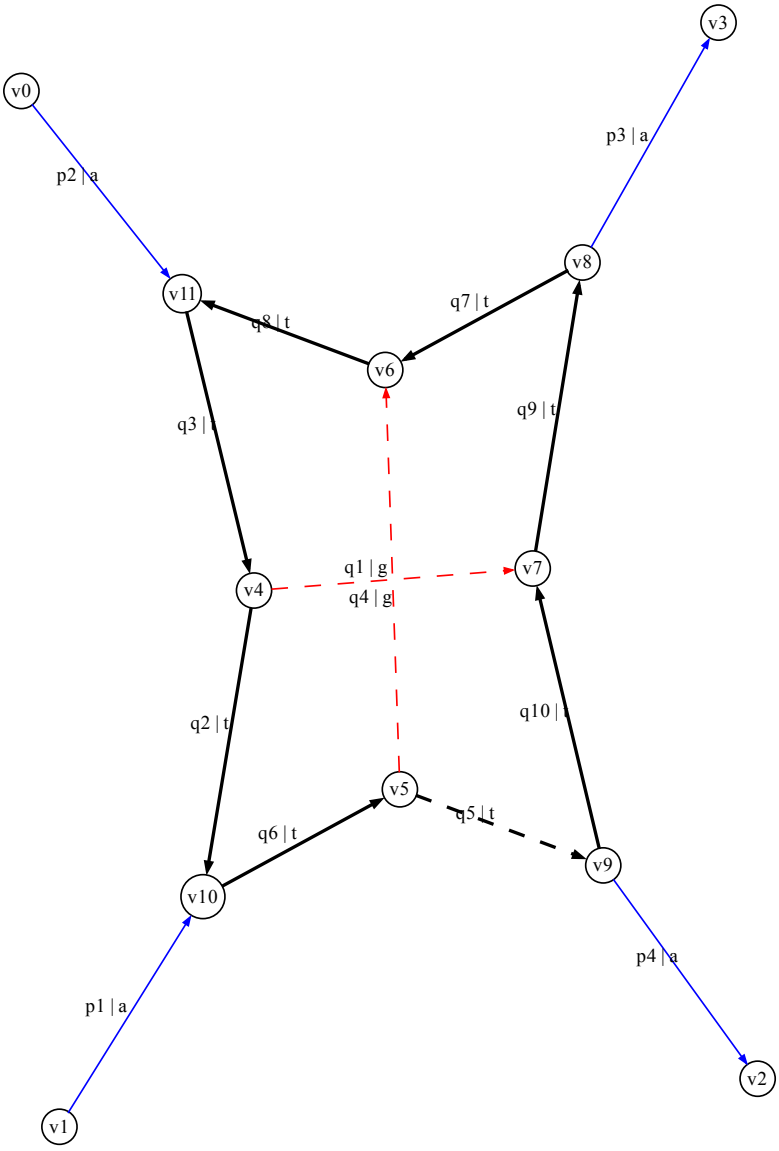

FSG GL376 #114 x (-2)

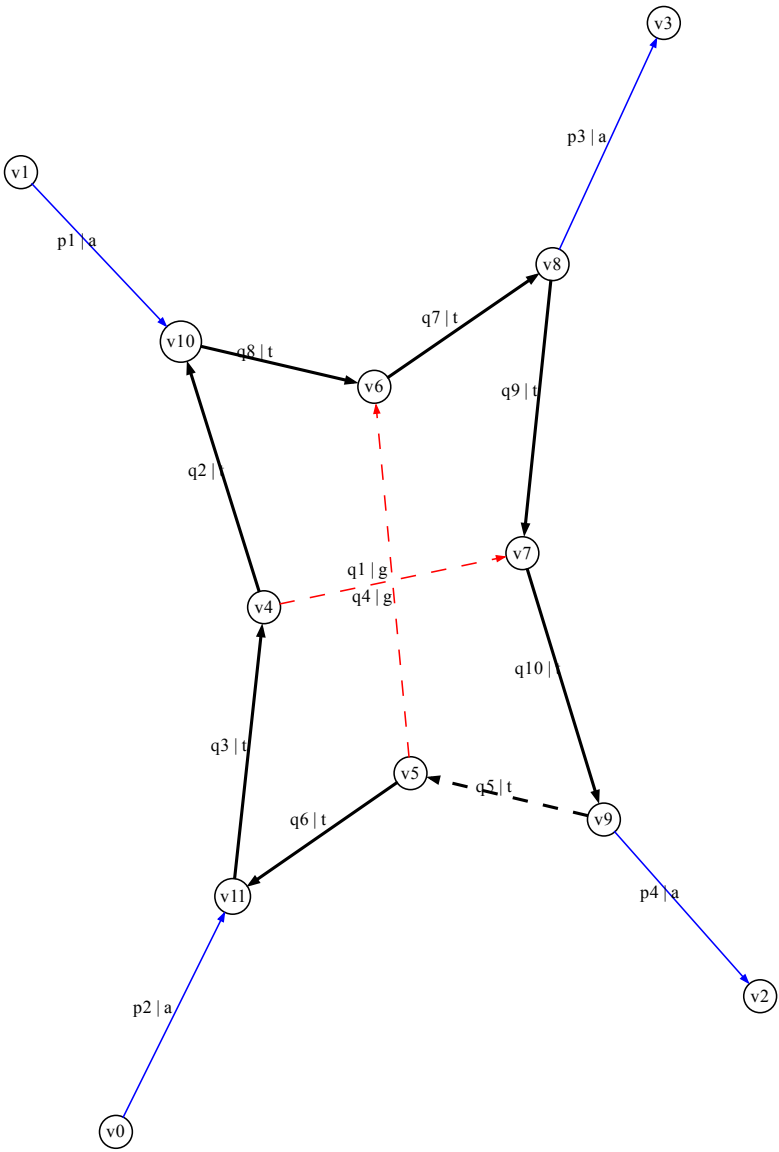

FSG GL378 #115 x (-2)

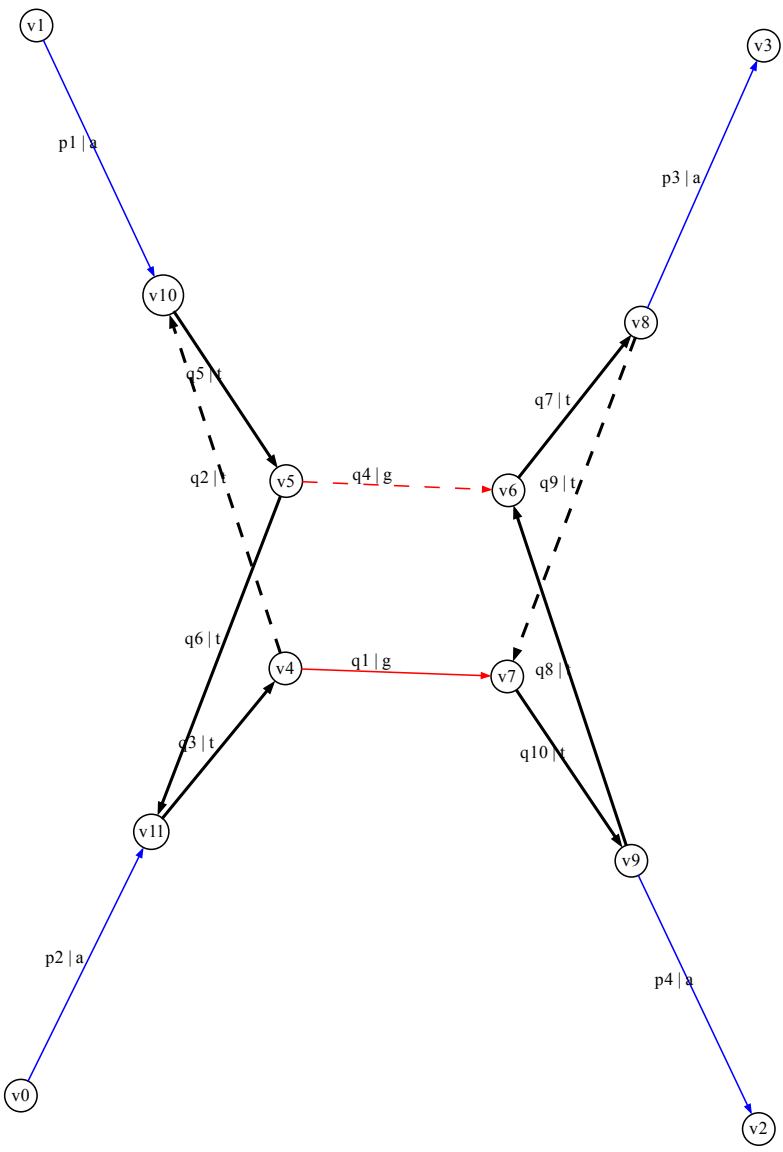

FSG GL380 #116 x (2)

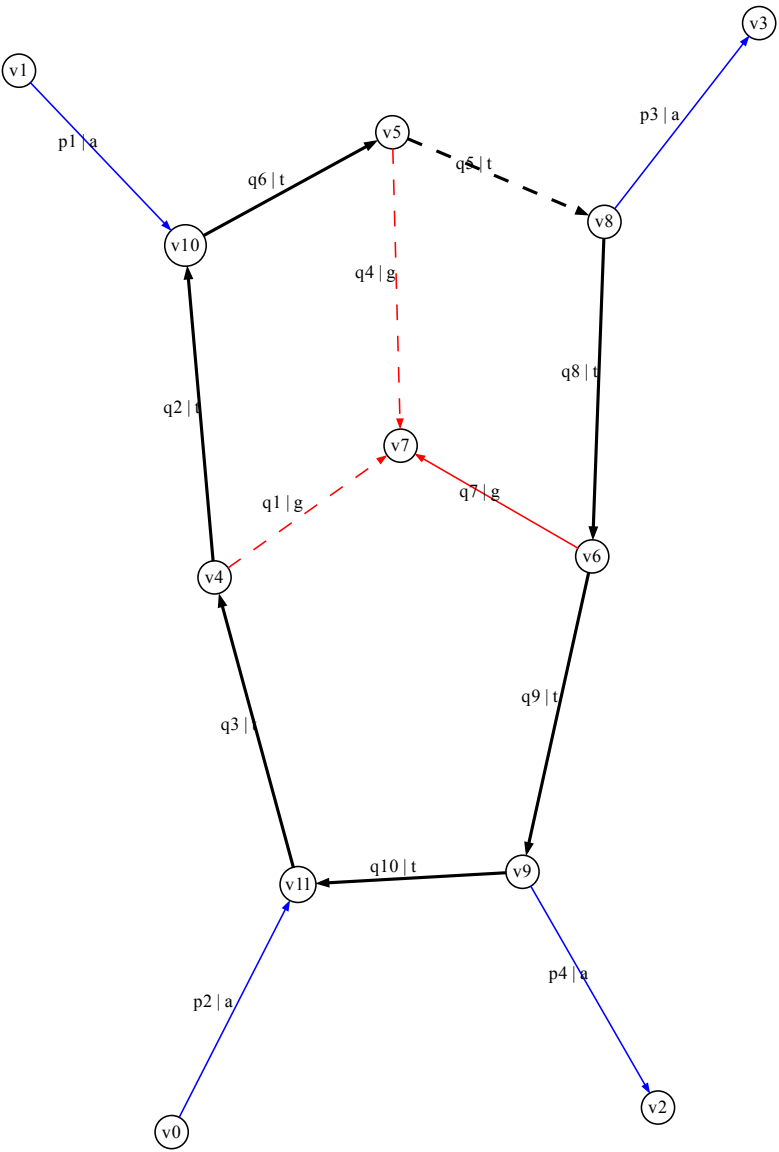

FSG GL382 #117 x (-4)

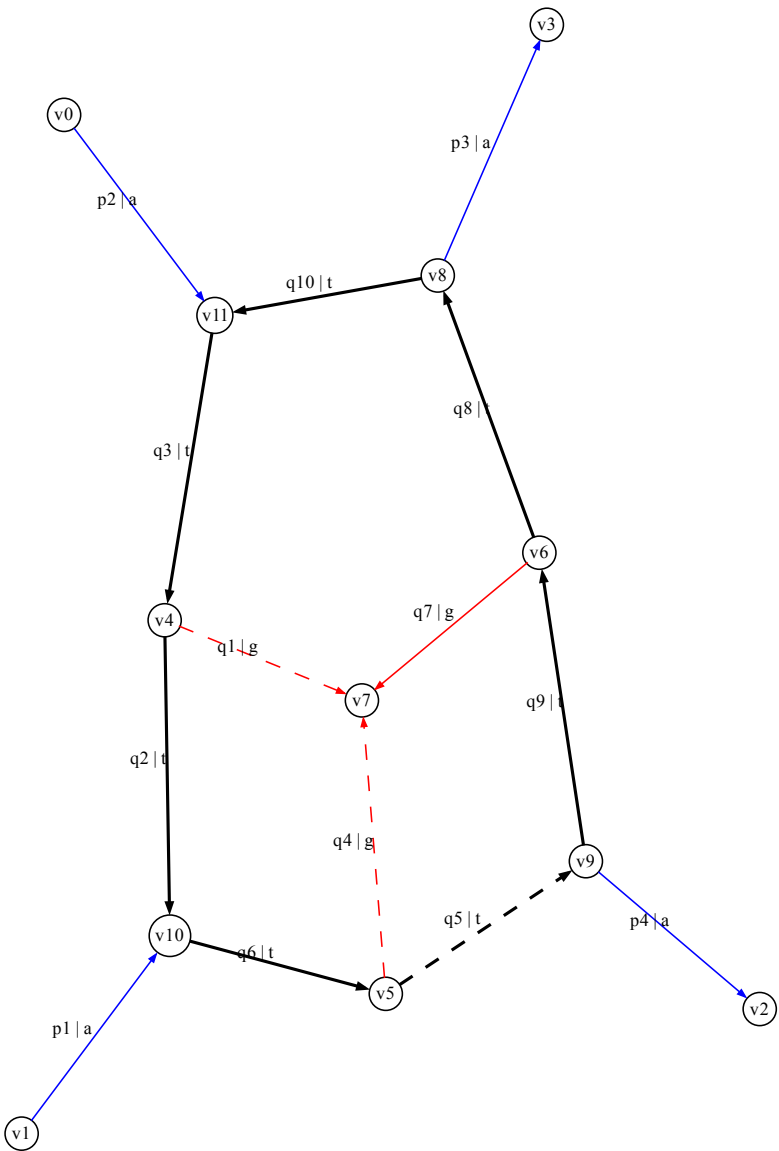

FSG GL384 #118 x (-4)

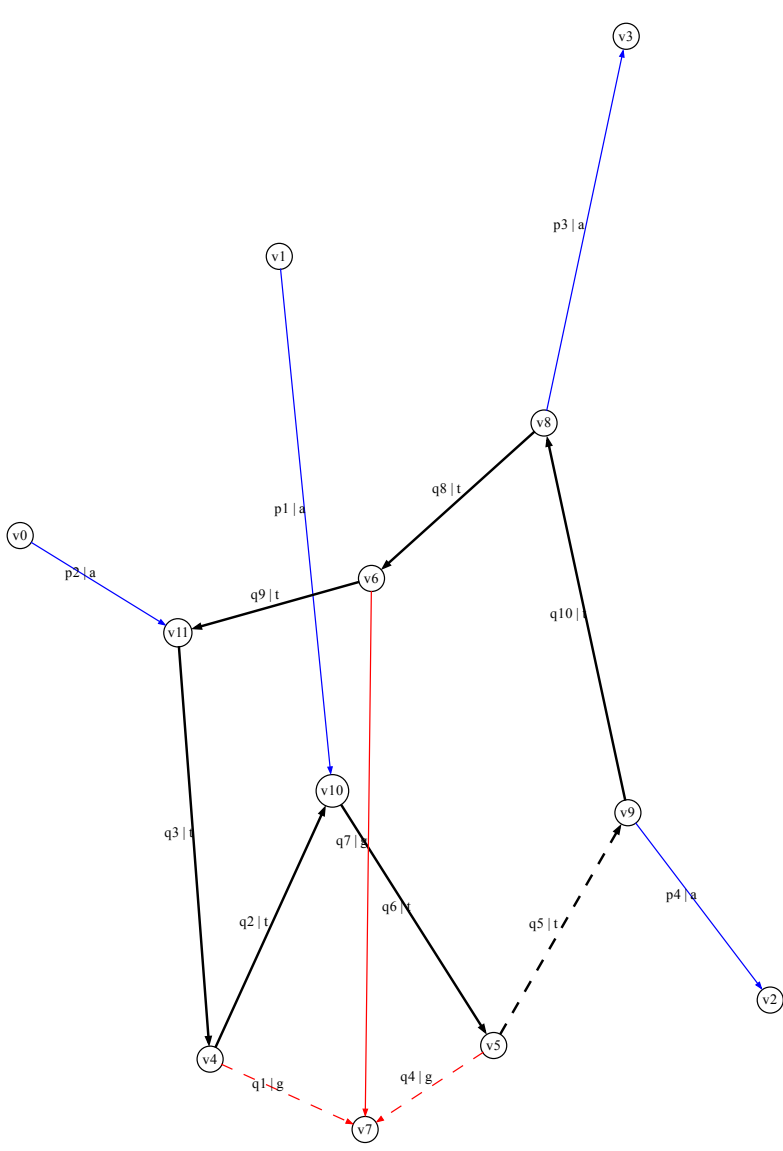

FSG GL386 #119 x (-4)

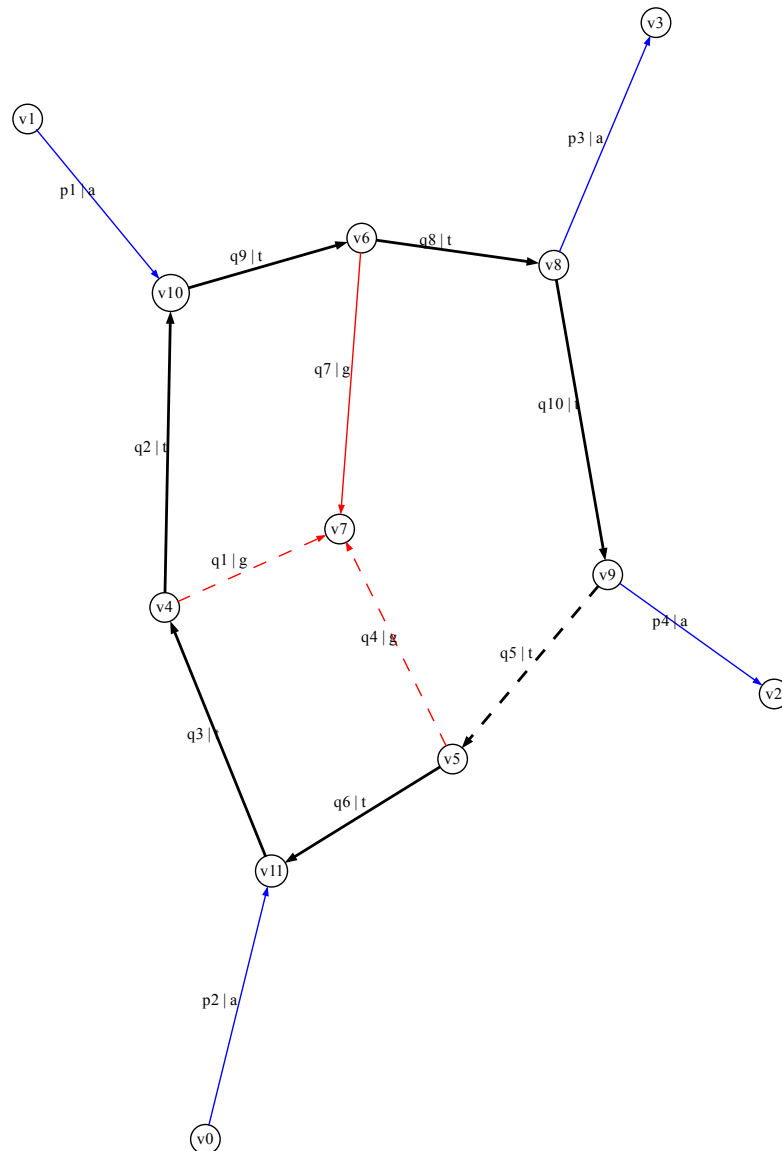

FSG GL388 #120 x (-4)

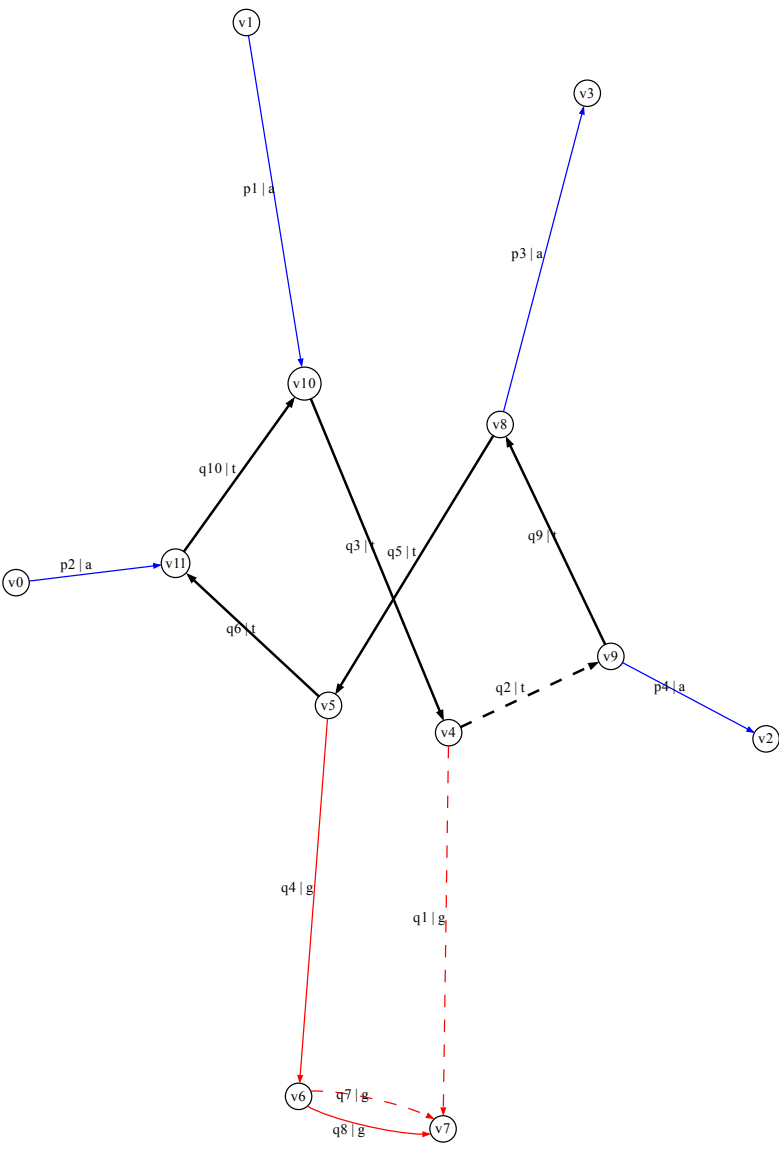

FSG GL394 #121 x (-1)

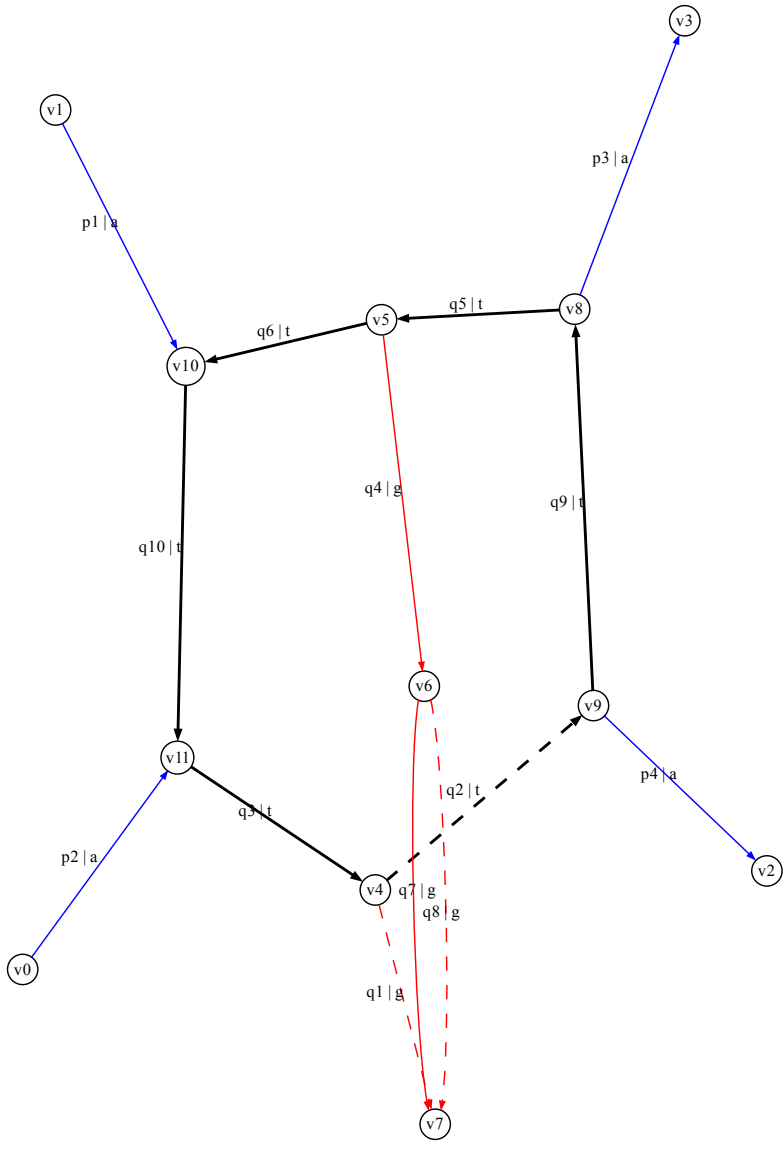

FSG GL396 #122 x (-1)

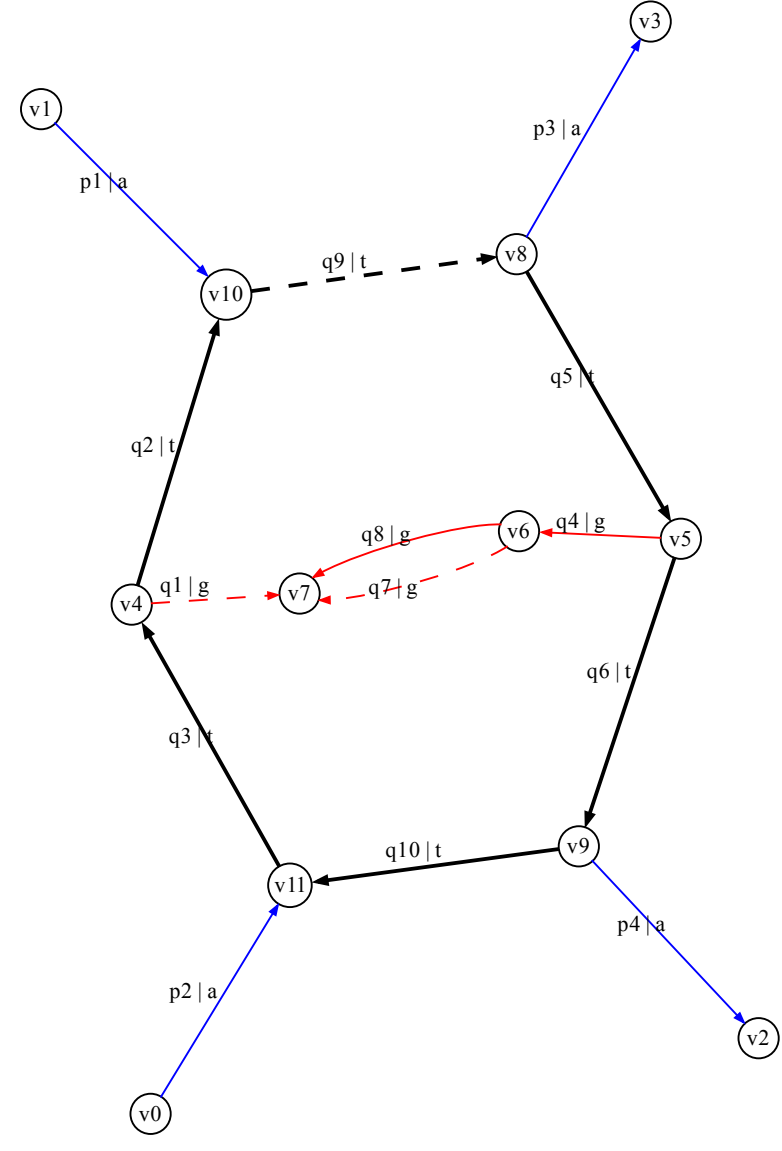

FSG GL402 #123 x (-1)

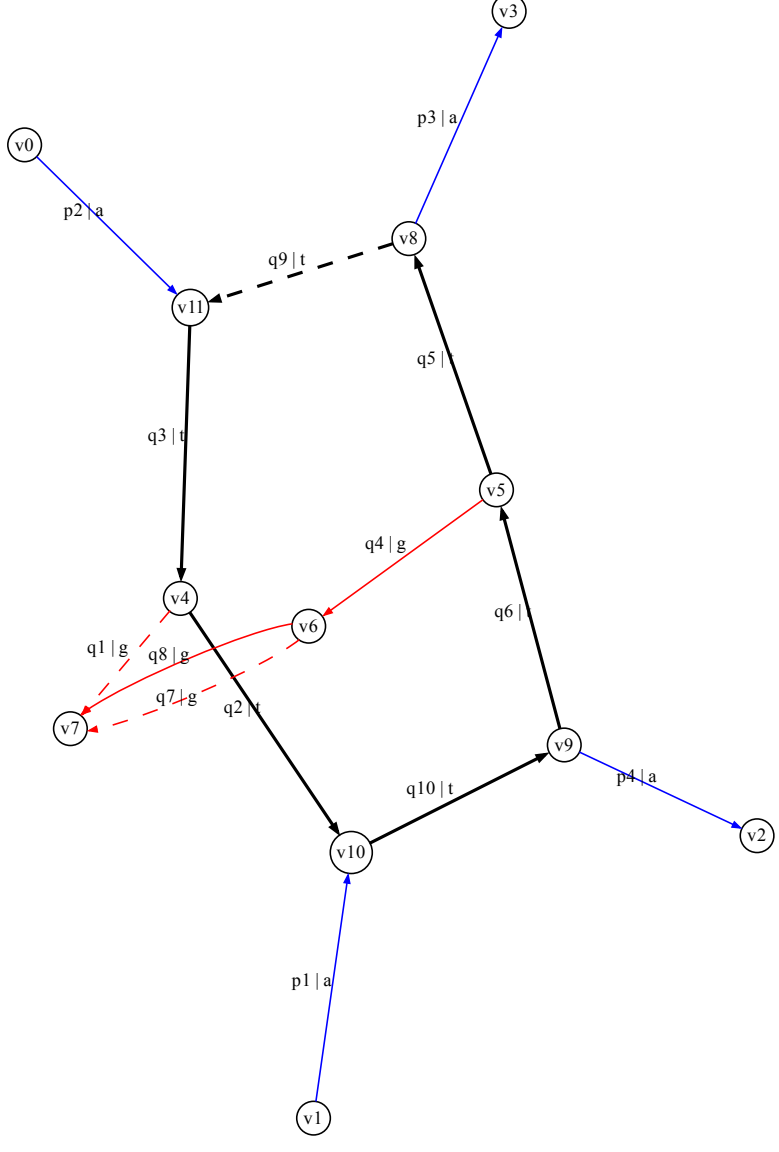

FSG GL404 #124 x (-1)

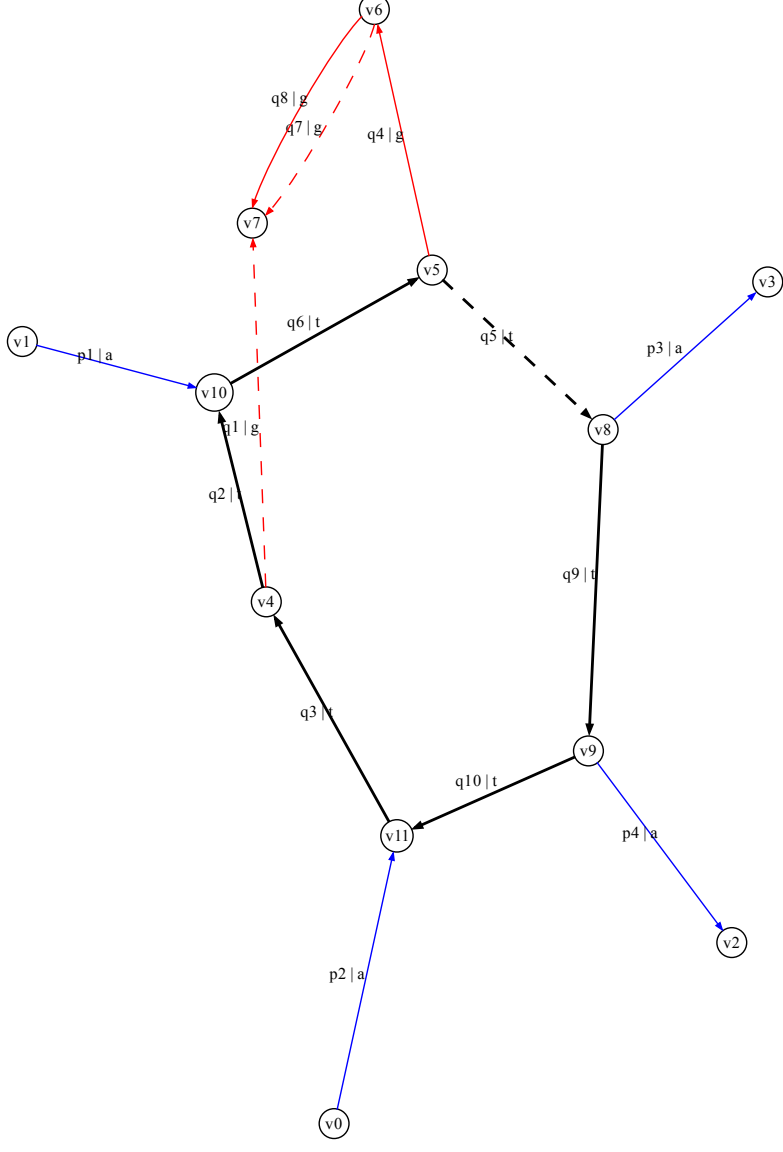

FSG GL406 #125 x (-4)

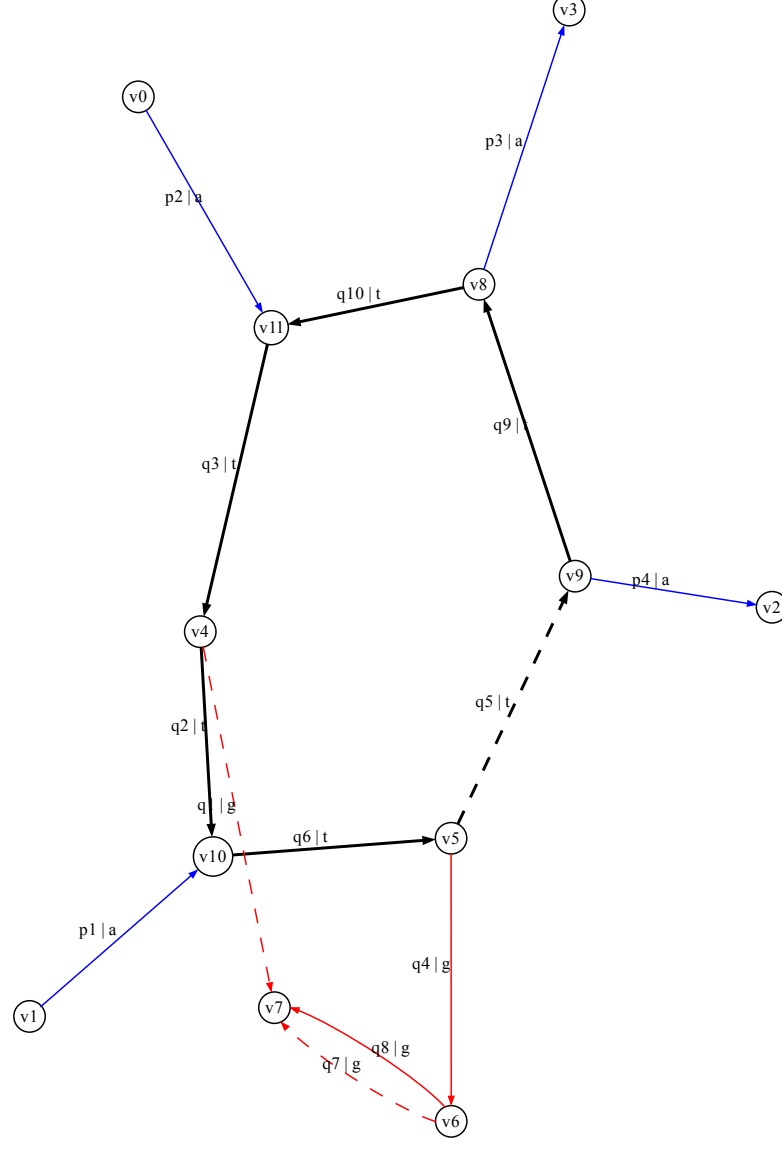

FSG GL408 #126 x (-4)

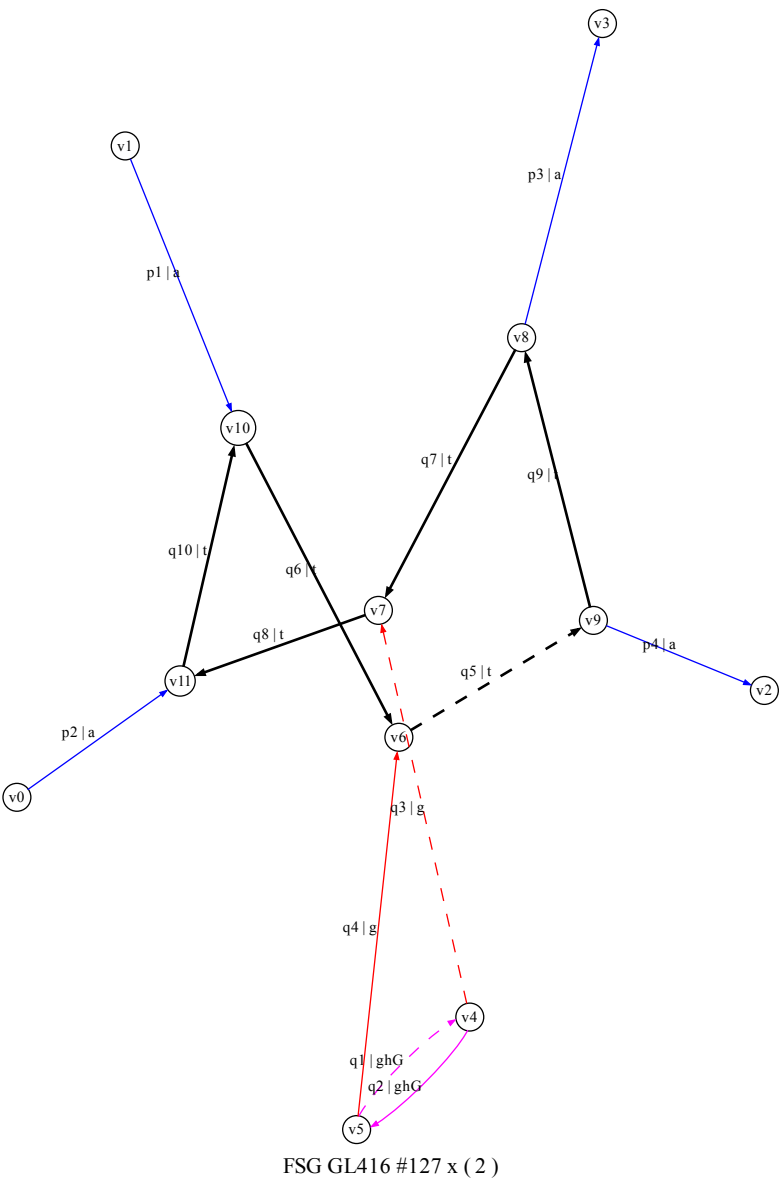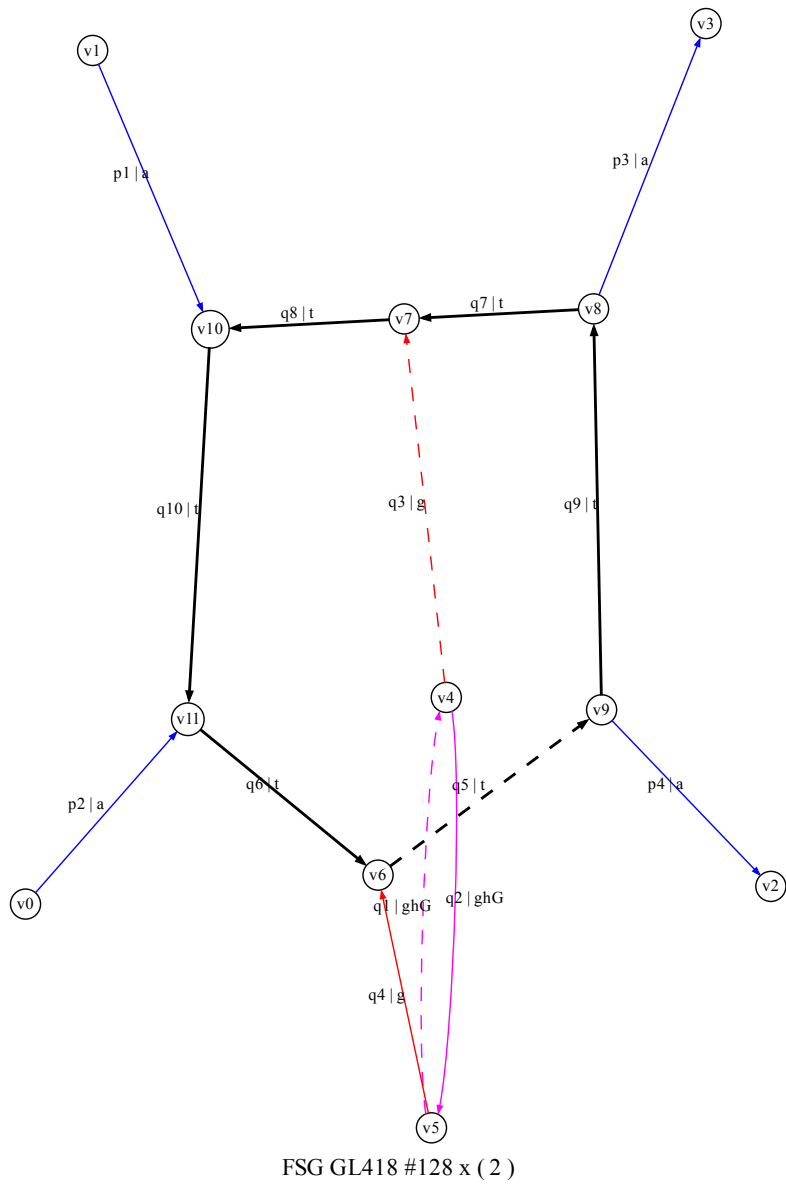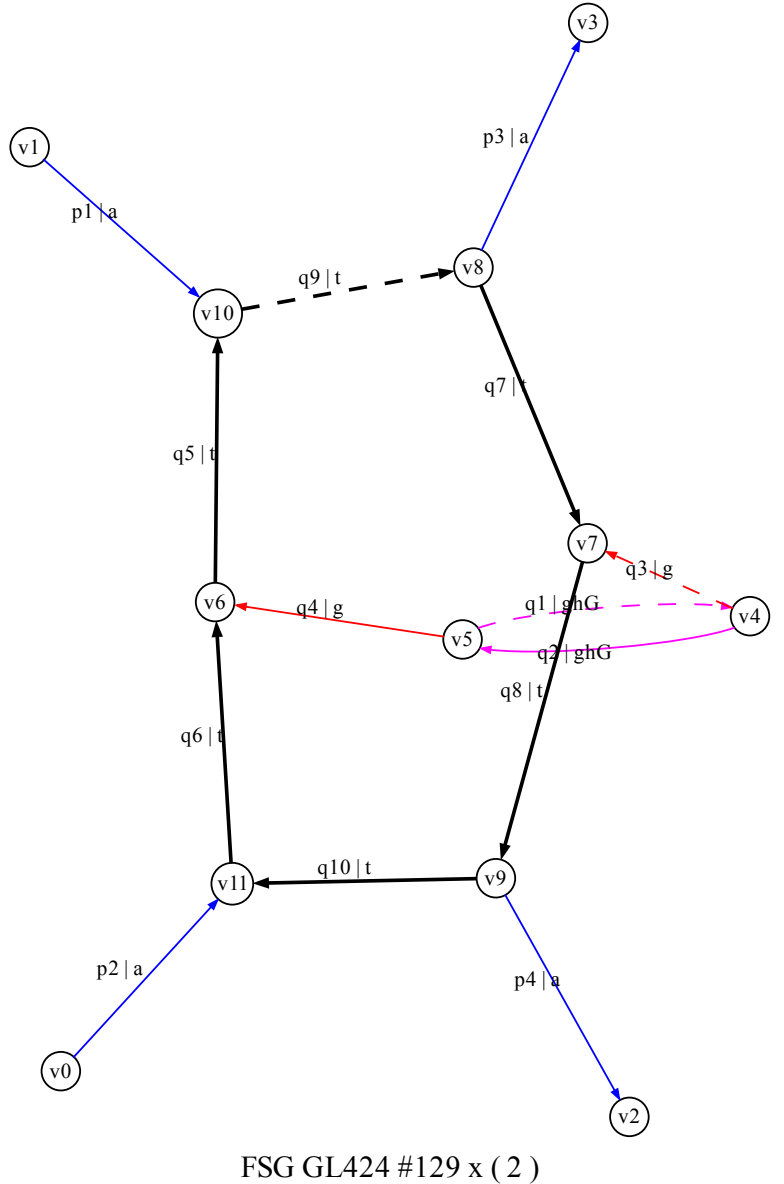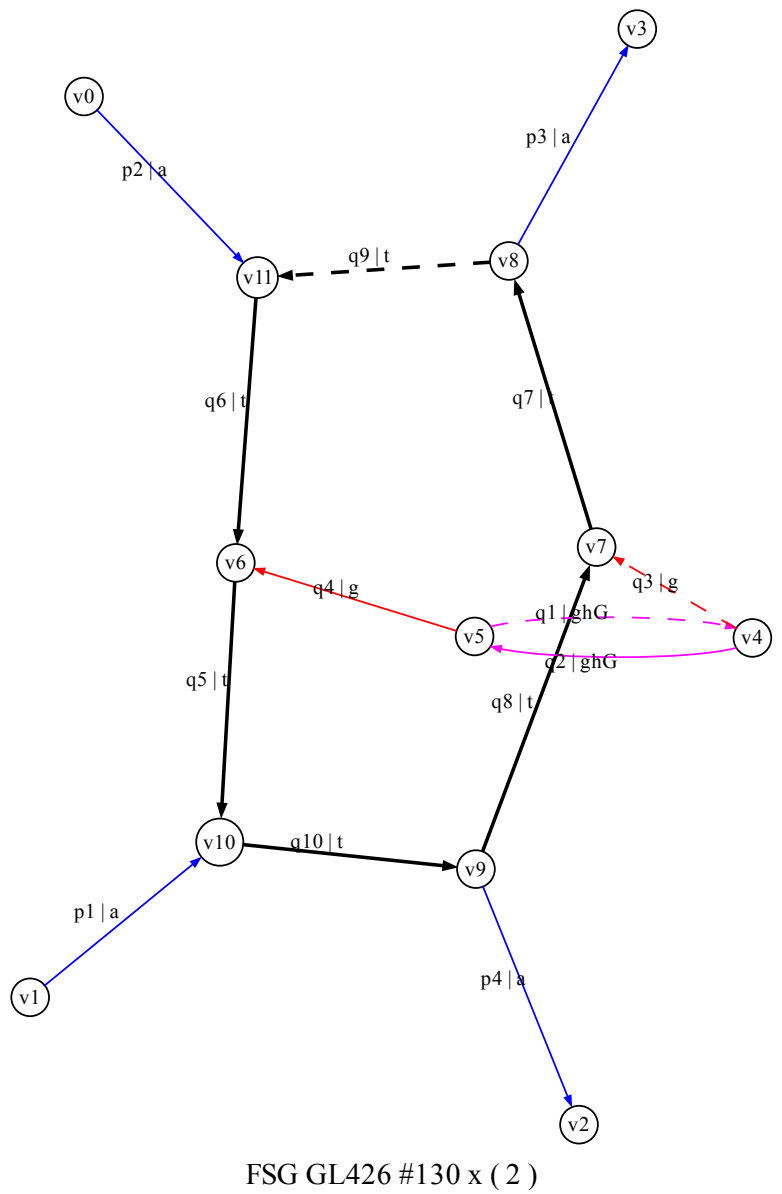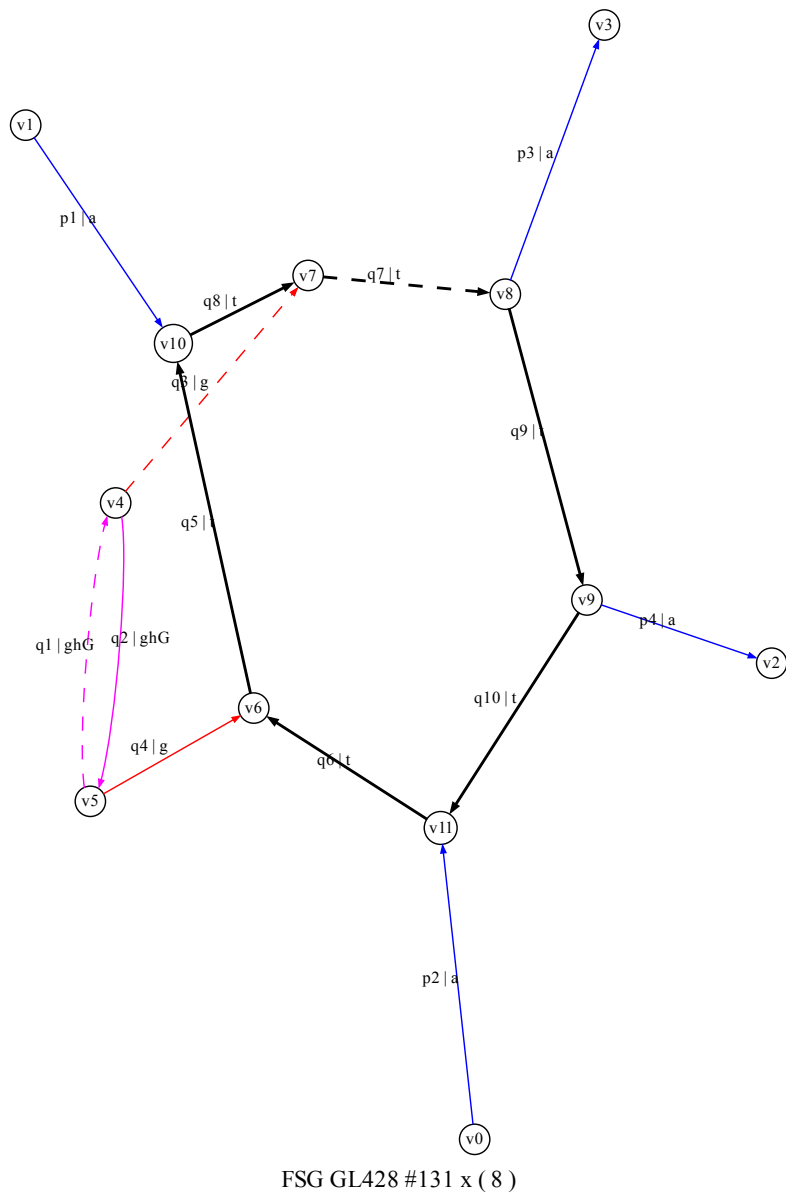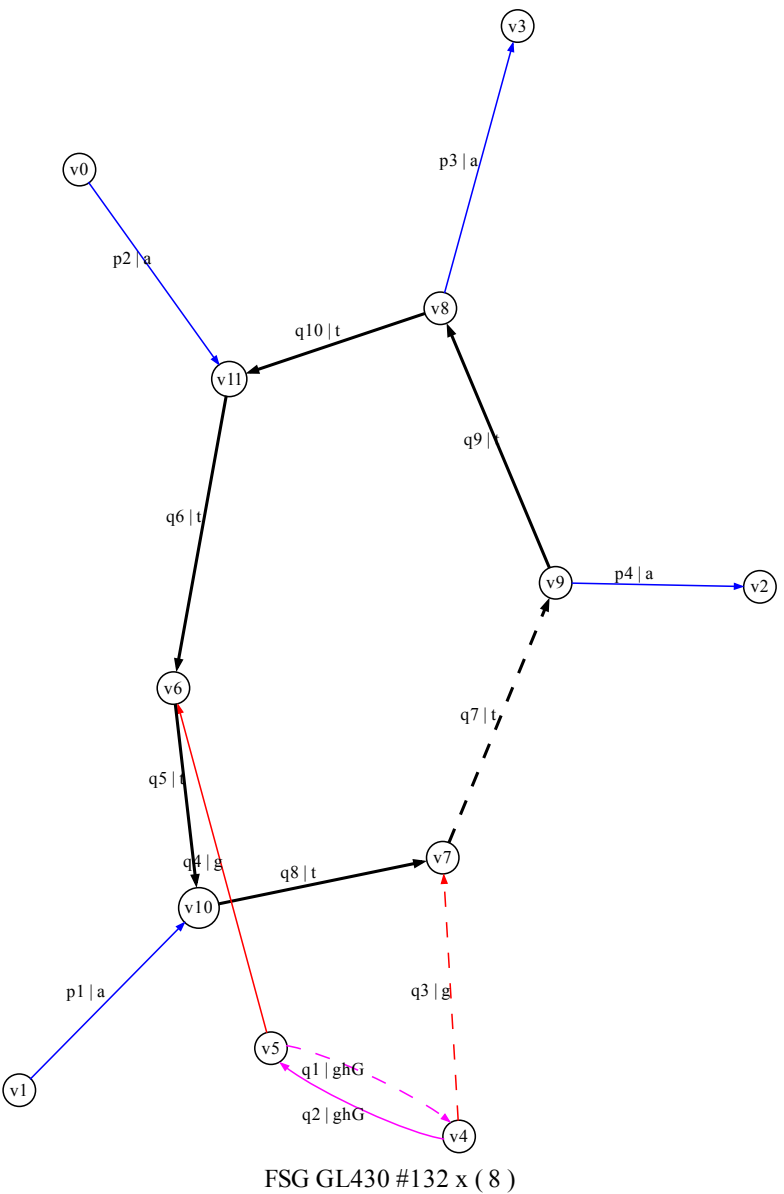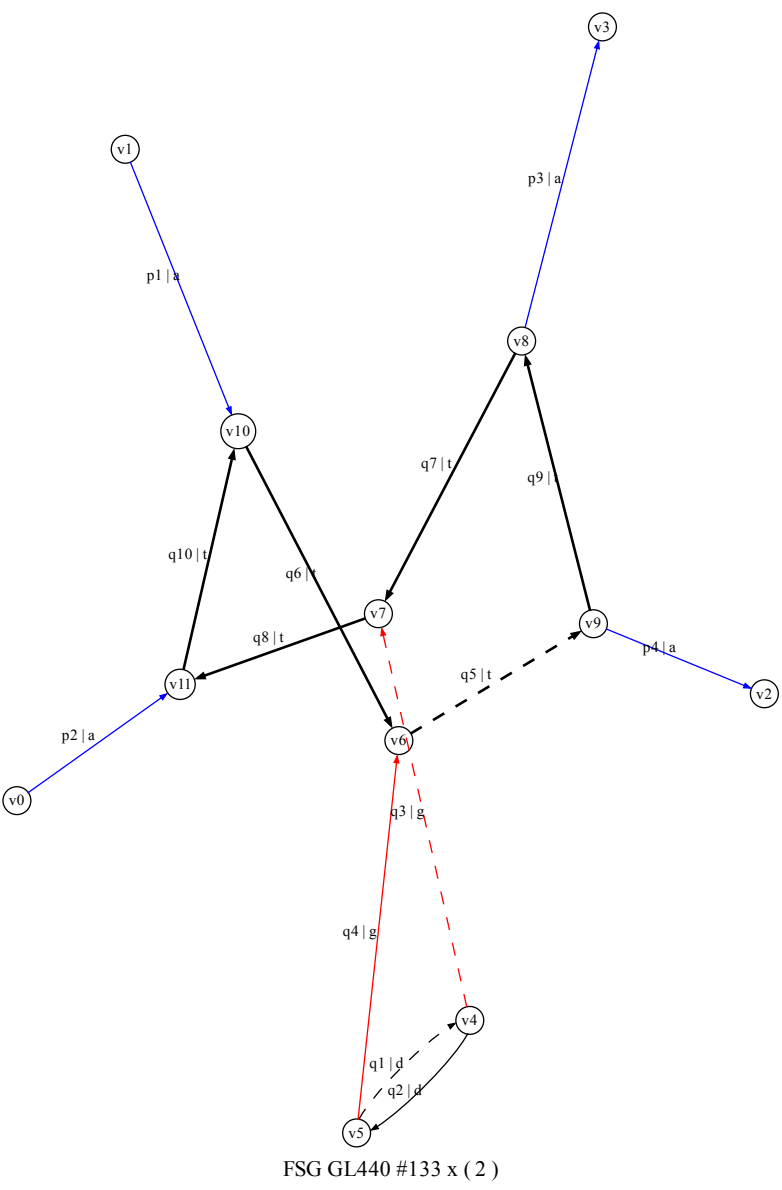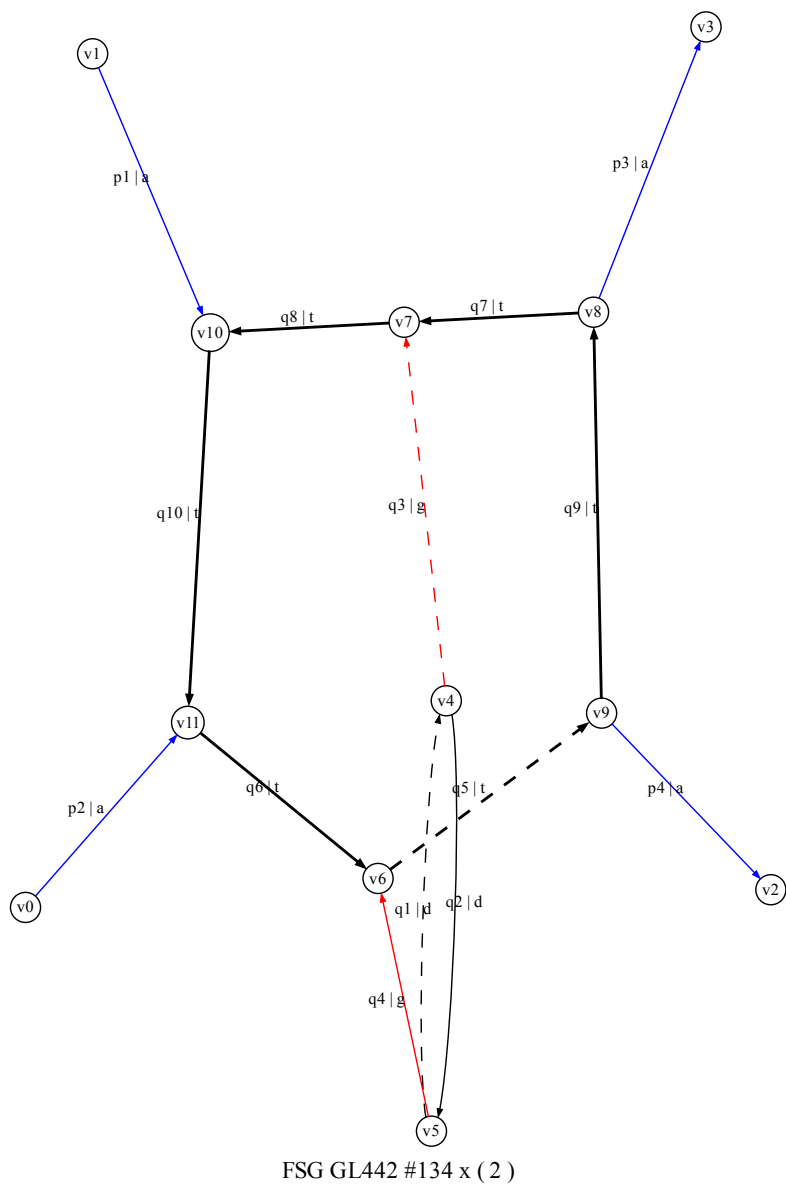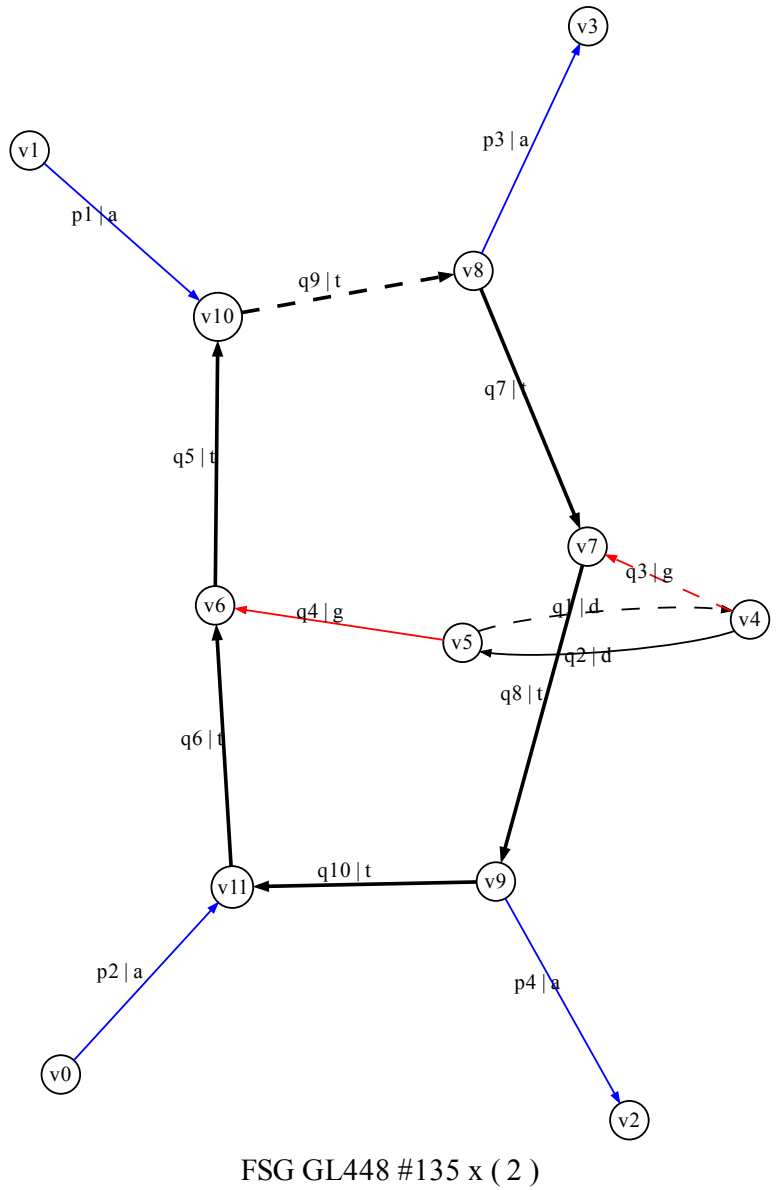

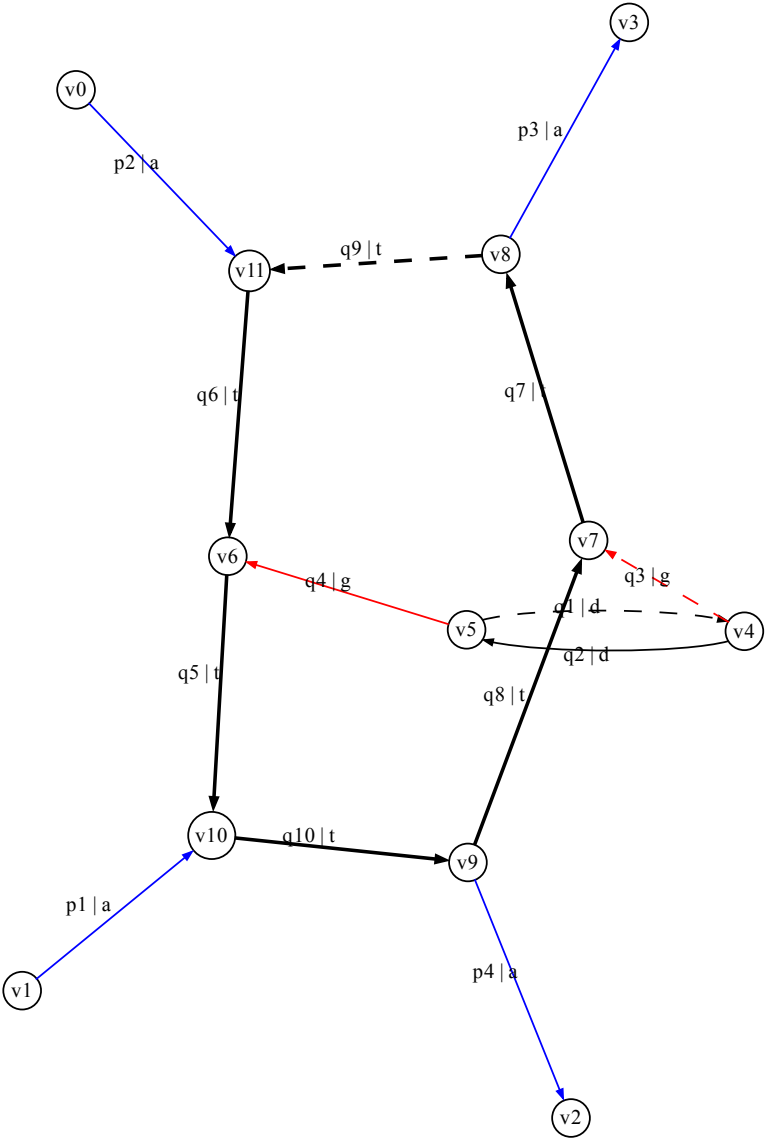

FSG GL450 #136 x ( 2 )

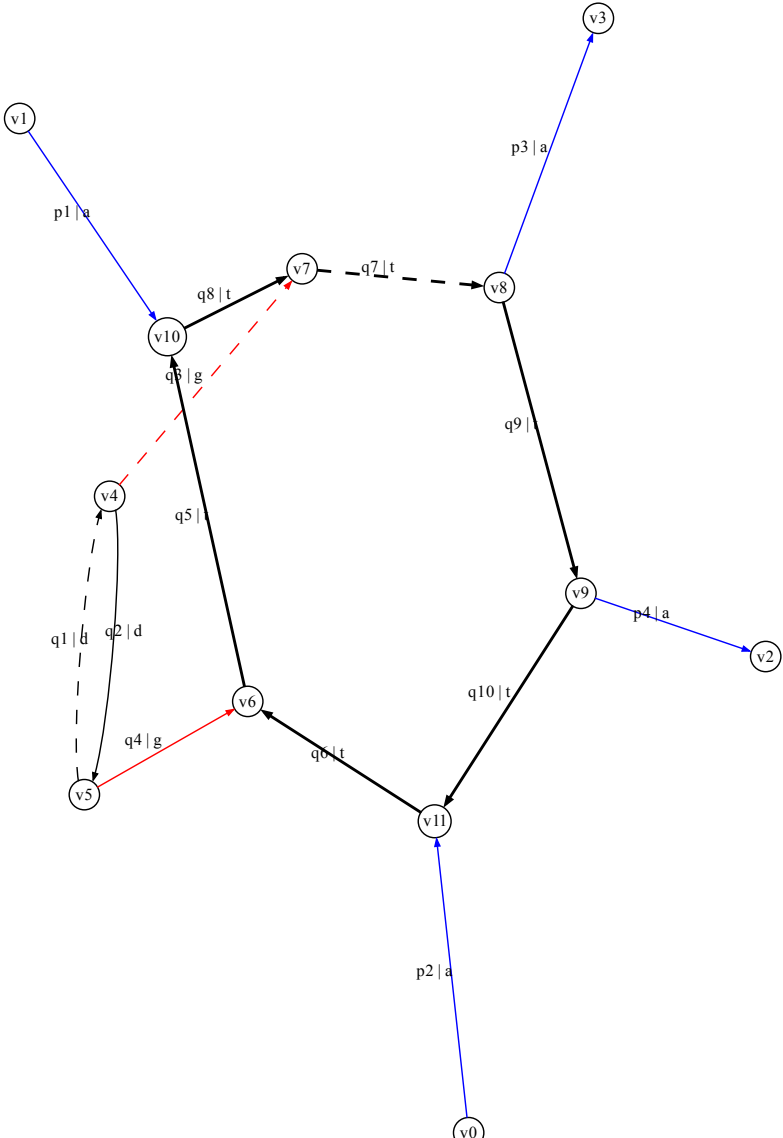

FSG GL452 #137 x ( 8 )

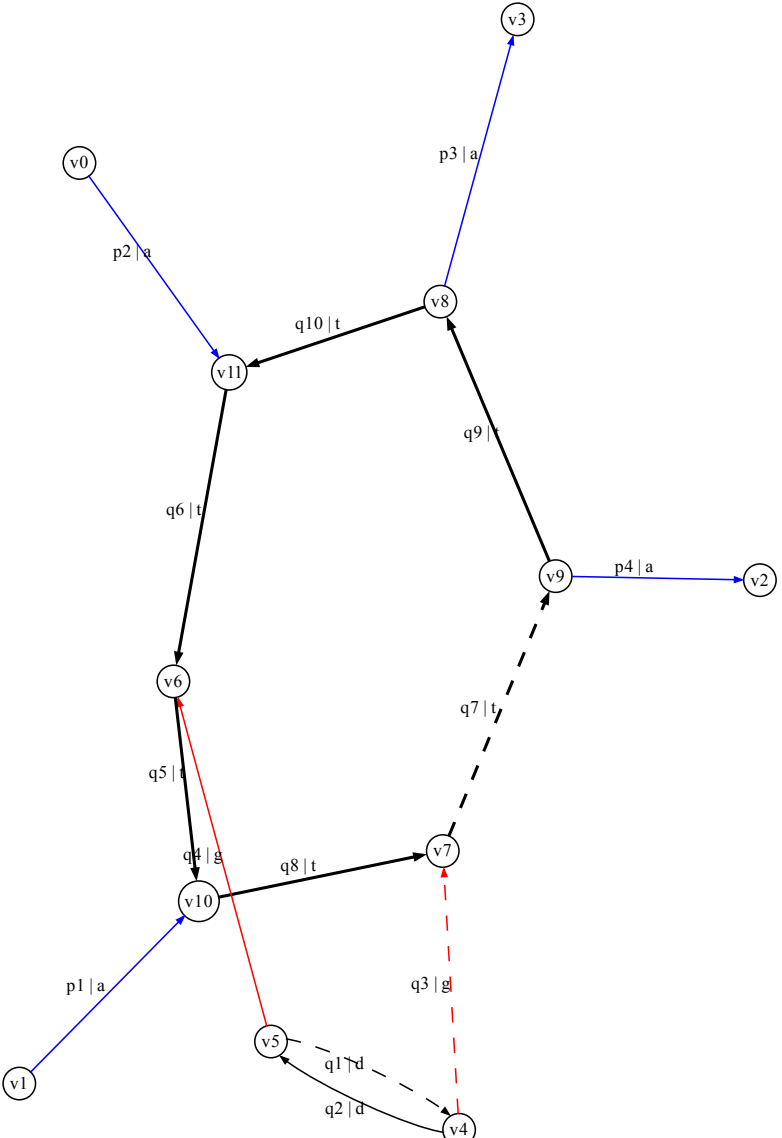

FSG GL454 #138 x ( 8 )
